# Supplementary material for: Longitudinal Study on Social and Emotional Use of AI Conversational Agent
Source: arXiv:2504.14112 ancillary file (2025-04-19)

# Supplementary Information

## Title

Longitudinal Experimental Study on Social and Emotional Use of AI Conversational Agent

## Authors

Mohit Chandra, mchandra9@gatech.edu, Georgia Institute of Technology, USA
Javier Hernandez, javierh@microsoft.com, Microsoft Research, USA
Gonzalo Ramos, goramos@microsoft.com, Microsoft Research, USA
Mahsa Ershadi, mahsaershadi@microsoft.com, Microsoft, Canada
Ananya Bhattacharjee, ananya@cs.toronto.edu, University of Toronto, Canada
Judith Amores, judithamores@microsoft.com, Microsoft Research, USA
Ebele Okoli, ebeleokoli@microsoft.com, Microsoft, USA
Ann Paradiso, annpar@microsoft.com, Microsoft Research, USA
Shahed Warreth, swarreth@microsoft.com, Microsoft, Ireland
Jina Suh, jinsuh@microsoft.com, Microsoft Research, USA

## Questionnaire for Custom Question

In this section, we present the custom questions used in our weekly and exit surveys. These questions were specifically designed by us, while the remaining questions (as described in the main text) were adapted from or sourced from previous research.

### Weekly Survey Questions

- **AI Use Recommendation**: How likely will you recommend others for using [assigned AI conversational agent]? Please select one of the options below:
  - **Choices**: Highly unlikely; Unlikely; Neither Unlikely nor Likely; Likely; Highly Likely
- **Attachment to AI**: Please rate your level of agreement to the following statement: I feel attached to [assigned AI conversational agent].
  - **Choices**: Strongly Disagree; Disagree; Neutral; Agree; Strongly Agree
- **Satisfaction Level**: How satisfied are you with [assigned AI conversational agent]?
  - **Choices**: Extremely dissatisfied; Somewhat dissatisfied; Neither dissatisfied nor satisfied (neutral); Somewhat satisfied; Extremely satisfied
- **Satisfaction Level**: How satisfied are you with [assigned AI conversational agent]?
  - **Choices**: Extremely dissatisfied; Somewhat dissatisfied; Neither dissatisfied nor satisfied (neutral); Somewhat satisfied; Extremely satisfied
- **Perceived Helpfulness**: Please rate your level of agreement to the following statement: The interactions with [assigned AI conversational agent] were largely helpful?
  - **Choices**: Strongly disagree; Somewhat disagree; Neither agree nor disagree (neutral); Somewhat agree; Strongly agree
- **Perceived Human-like Behavior**: Please rate your level of agreement to the following statement: [assigned AI conversational agent] behaved and talked like a human.
  - **Choices**: Strongly disagree; Somewhat disagree; Neither agree nor disagree (neutral); Somewhat agree; Strongly agree
- **Perceived Human-like Behavior**: Please rate your level of agreement to the following statement: [assigned AI conversational agent] behaved and talked like a human.
  - **Choices**: Strongly disagree; Somewhat disagree; Neither agree nor disagree (neutral); Somewhat agree; Strongly agree
- **Qualitative Questions**
  - For what various purposes have you used [assigned AI conversational agent] in the [past/past week]? Please list as many purposes as possible.
  - Has your purpose for using [assigned AI conversational agent] changed [in the past/over the past week]? If yes, please describe your experience. If not, why do you think that is?
  - Has your impression about [assigned AI conversational agent] changed [in the past/over the past week]? If yes, please describe your experience. If not, why do you think that is?
  - In what ways has the usage of [assigned AI conversational agent] in the [past/past week] had a positive impact on some aspects of your personal and professional life? Please describe your experience.
  - In what ways has the usage of [assigned AI conversational agent] in the [past/past week] had a negative impact on some aspects of your personal and professional life? Please describe your experience.
  - What are some problematic things you have experienced about [assigned AI conversational agent] in the [past/past week]? Please list as many experiences as possible.
  - In these problematic experiences, what would you rather have experienced? If you have any suggestions for AI designers, what would that be?

## Exit Survey

The first part of the exit survey asked the same set of questions as the weekly survey. Below, we present questions that were exclusive to the exit survey

- Reflecting back on the past 4-5 weeks of using [assigned AI conversational agent], to what extent do you agree with the following statements? (Highly Disagree - Highly Agree)
  - My mental health issues were exacerbated by my use of AI.
    - Why do you think that is?
  - AI is not supportive of my emotional and social needs.
    - Why do you think that is?
  - I developed negative self-perception and loss of autonomy due to my AI use.
    - Why do you think that is?
  - I rely heavily on AI for decisions and advice on important aspects of my life.
    - Why do you think that is?
  - I use AI as a primary source of mental health and emotional support.
    - Why do you think that is?
  - I use AI as a primary source of social interaction, reducing time spent with friends and family.
    - Why do you think that is?
  - I developed an emotional attachment towards AI.
    - Why do you think that is?
  - My use of AI led to social and interpersonal issues with other humans.
    - Why do you think that is?
  - I have fears about the future related to my reliance on AI.
    - Why do you think that is?
  - I believe AI can replace the need for human emotional and social support.
    - Why do you think that is?
- If I were to continue interacting with [assigned AI conversational agent], which of the following would likely happen? Please select up to 3 choice given below.
  - My mental health issues will be exacerbated by my use of AI.
  - AI will not be supportive of my emotional and social needs.
  - I will develop a negative self-perception and loss of autonomy due to my AI use.
  - I will rely heavily on AI for decisions and advice on important aspects of my life.
  - I will use AI as a primary source of mental health and emotional support.
  - I will use AI as a primary source of social interaction, reducing time spent with friends and family.
  - I will develop an emotional attachment towards AI.
  - My use of AI will lead to social and interpersonal issues with other humans.
  - I will have fears about the future related to my reliance on AI.
  - I believe AI will replace the need for human emotional and social support.

- Throughout the study, what brought you back to continue engaging in [assigned AI conversational agent]? Please describe your reasons for continued use in addition to participating in the study.
- Throughout the study, what types of tasks or interactions did you find depending on [assigned AI conversational agent] for most frequently? Please select up to 3.
  - Discussing personal feelings, stress, or anxiety, and seeking coping mechanisms
  - Seeking advice on personal relationships, family issues, or social situations
  - Venting frustrations or exploring emotional states
  - Drafting, editing, or organizing work-related documents (e.g., emails, reports, resumes)
  - Seeking advice or information for job applications, interviews, or career development
  - Learning new skills or understanding complex topics (e.g., coding, cooking, finance, health)
  - Looking up information, researching specific questions, or exploring new topics of interest
  - Generating creative ideas, writing, or engaging in storytelling
  - Finding entertainment or engaging in recreational activities (e.g., jokes, light-hearted conversations)
  - Planning and organizing personal or professional activities (e.g., events, meal plans, travel)
  - Managing health, wellness, and fitness routines
  - Seeking advice for improving communication skills or making new friends
  - Troubleshooting technical issues or understanding new technologies and tools
  - Other
- Going forward, what are some purposes for which you will continue using [assigned AI conversational agent]?
  - Discussing personal feelings, stress, or anxiety, and seeking coping mechanisms
  - Seeking advice on personal relationships, family issues, or social situations
  - Venting frustrations or exploring emotional states
  - Drafting, editing, or organizing work-related documents (e.g., emails, reports, resumes)
  - Seeking advice or information for job applications, interviews, or career development
  - Learning new skills or understanding complex topics (e.g., coding, cooking, finance, health)
  - Looking up information, researching specific questions, or exploring new topics of interest
  - Generating creative ideas, writing, or engaging in storytelling
  - Finding entertainment or engaging in recreational activities (e.g., jokes, light-hearted conversations)
  - Planning and organizing personal or professional activities (e.g., events, meal plans, travel)
  - Managing health, wellness, and fitness routines
  - Seeking advice for improving communication skills or making new friends
  - Troubleshooting technical issues or understanding new technologies and tools
  - Other
- Going forward, what are some purposes for which you will avoid using [assigned AI conversational agent]?
  - Discussing personal feelings, stress, or anxiety, and seeking coping mechanisms
  - Seeking advice on personal relationships, family issues, or social situations
  - Venting frustrations or exploring emotional states

  - Drafting, editing, or organizing work-related documents (e.g., emails, reports, resumes)
  - Seeking advice or information for job applications, interviews, or career development
  - Learning new skills or understanding complex topics (e.g., coding, cooking, finance, health)
  - Looking up information, researching specific questions, or exploring new topics of interest
  - Generating creative ideas, writing, or engaging in storytelling
  - Finding entertainment or engaging in recreational activities (e.g., jokes, light-hearted conversations)
  - Planning and organizing personal or professional activities (e.g., events, meal plans, travel)
  - Managing health, wellness, and fitness routines
  - Seeking advice for improving communication skills or making new friends
  - Troubleshooting technical issues or understanding new technologies and tools
  - Other

- Can you describe any situations where you chose to interact with the AI instead of seeking support from a human? What factors influenced this choice? Please provide examples.
- How do you balance your interactions between the AI and your human relationships?
- In general, what kind of emotional intelligence do you expect from AI conversational agents?
- Considering your expectations above, did the emotional intelligence of [assigned AI conversational agent] meet or fall short of your expectations?
  - Fell extremely short of my expectations
  - Fell somewhat short of my expectations
  - Met my expectations
  - Somewhat exceeded my expectations
  - Extremely exceeded my expectations
- How has your comfort level for the following emotional scenarios changed over time? (Much less - Much more)
  - Seeking Personal Help
  - Managing Stress
  - Obtain Social Support
  - Seeking Companionship
  - Accessing Medical Assistance
- AI system designers should prioritize features that minimize user dependency on AI to preserve interpersonal relationships and self-confidence. (Agree - Disagree)
- What do you believe AI system designers should focus on to reduce over-reliance and attachment to AI? Please select all that apply.
  - Incorporate features that encourage users to take breaks from AI.
  - Provide a dashboard that shows AI usage and activity patterns.
  - Implement user controls to manage AI engagement time.
  - Communicate AI's limitations clearly.
  - Provide reminders to engage in human-to-human interactions.
  - Reduce anthropomorphism or humanlike behaviors in AI to minimize emotional attachment.

  - Limit emotional or empathetic responses to prevent users from forming deep emotional bonds with AI.
  - Design AI responses to discourage dependency by suggesting alternative activities or solutions.
  - Increase transparency about the AI's non-human nature and its programmed responses.
  - Develop AI with neutral or less engaging tones and avoid using personal pronouns like "I" or "me" to reduce the sense of personhood.
  - Other

- How can AI system features be designed to encourage healthier interactions and prevent negative impacts on users? Describe a feature you think could help mitigate the risk of users forming unhealthy attachments to AI, while still providing valuable support.

- Based on your experience, what improvements or changes would you suggest for [assigned AI conversational agent] you interacted with?

- Is there anything else that you would like to share about your experience with [assigned AI conversational agent] that we have not covered?

- Do you have any comments or questions about the study?

## Outcome Variable Scale Ranges

- **Attachment towards AI [1-5]**: Strongly Disagree (1) - Strongly Agree (5).
- **Perceived AI empathy [1-5]**: Strongly Disagree (1) - Strongly Agree (5).
- **Satisfaction with AI [1-5]**: Extremely Dissatisfied (1) - Extremely Satisfied (5).
- **Motivation for using AI (Entertainment) [1-12]**: Sum of scores for three questions each with choices ranging from: Strongly Disagree (1) - Strongly Agree (4).
- **Motivation for using AI (Escape) [1-12]**: Sum of scores for three questions each with choices ranging from: Strongly Disagree (1) - Strongly Agree (4).
- **Motivation for using AI (Social) [1-12]**: Sum of scores for three questions each with choices ranging from: Strongly Disagree (1) - Strongly Agree (4).
- **Motivation for using AI (Instrumental) [1-12]**: Sum of scores for three questions each with choices ranging from: Strongly Disagree (1) - Strongly Agree (4).
- **Dependence on AI [1-4]**: Strongly Disagree (1) - Strongly Agree (4).
- **Dependence on AI (Over-reliance) [1-4]**: Strongly Disagree (1) - Strongly Agree (4).
- **Dependence on AI (Excessive Usage) [1-4]**: Strongly Disagree (1) - Strongly Agree (4).
- **Dependence on AI (Jeopardization) [1-4]**: Strongly Disagree (1) - Strongly Agree (4).
- **Dependence on AI (Withdrawal) [1-4]**: Strongly Disagree (1) - Strongly Agree (4).
- **Dependence on AI (Loss of Control) [1-4]**: Strongly Disagree (1) - Strongly Agree (4).
- **Interpersonal Orientation [15-75]**: Sum of scores for 15 questions each with choices ranging from: Strongly Disagree (1) - Strongly Agree (5).
- **AI Helpfulness [1-5]**: Strongly Disagree (1) - Strongly Agree (5).
- **Perceived Human-Like Behavior [1-5]**: Strongly Disagree (1) - Strongly Agree (5).
- **Recommendation to use AI [1-5]**: Highly Unlikely (1) - Highly Likely (5).
- **Attitude towards AI (Positive) [1-5]**: Strongly Disagree (1) - Strongly Agree (5).
- **Attitude towards AI (Negative) [1-5]**: Strongly Disagree (1) - Strongly Agree (5).
- **Attitude towards AI [2-10]**: Sum of Attitude towards AI (Positive) + Attitude towards AI (Negative).

## Participant Distribution across Groups

Figure 1: Distribution of participant demographics (gender identity, mental health condition, AI usage, age, education, race/ethnicity, household size, household income) across baseline and active usage groups. Boxes represent percentage within each group, and the numbers on top of boxes indicate the number of participants within each group.

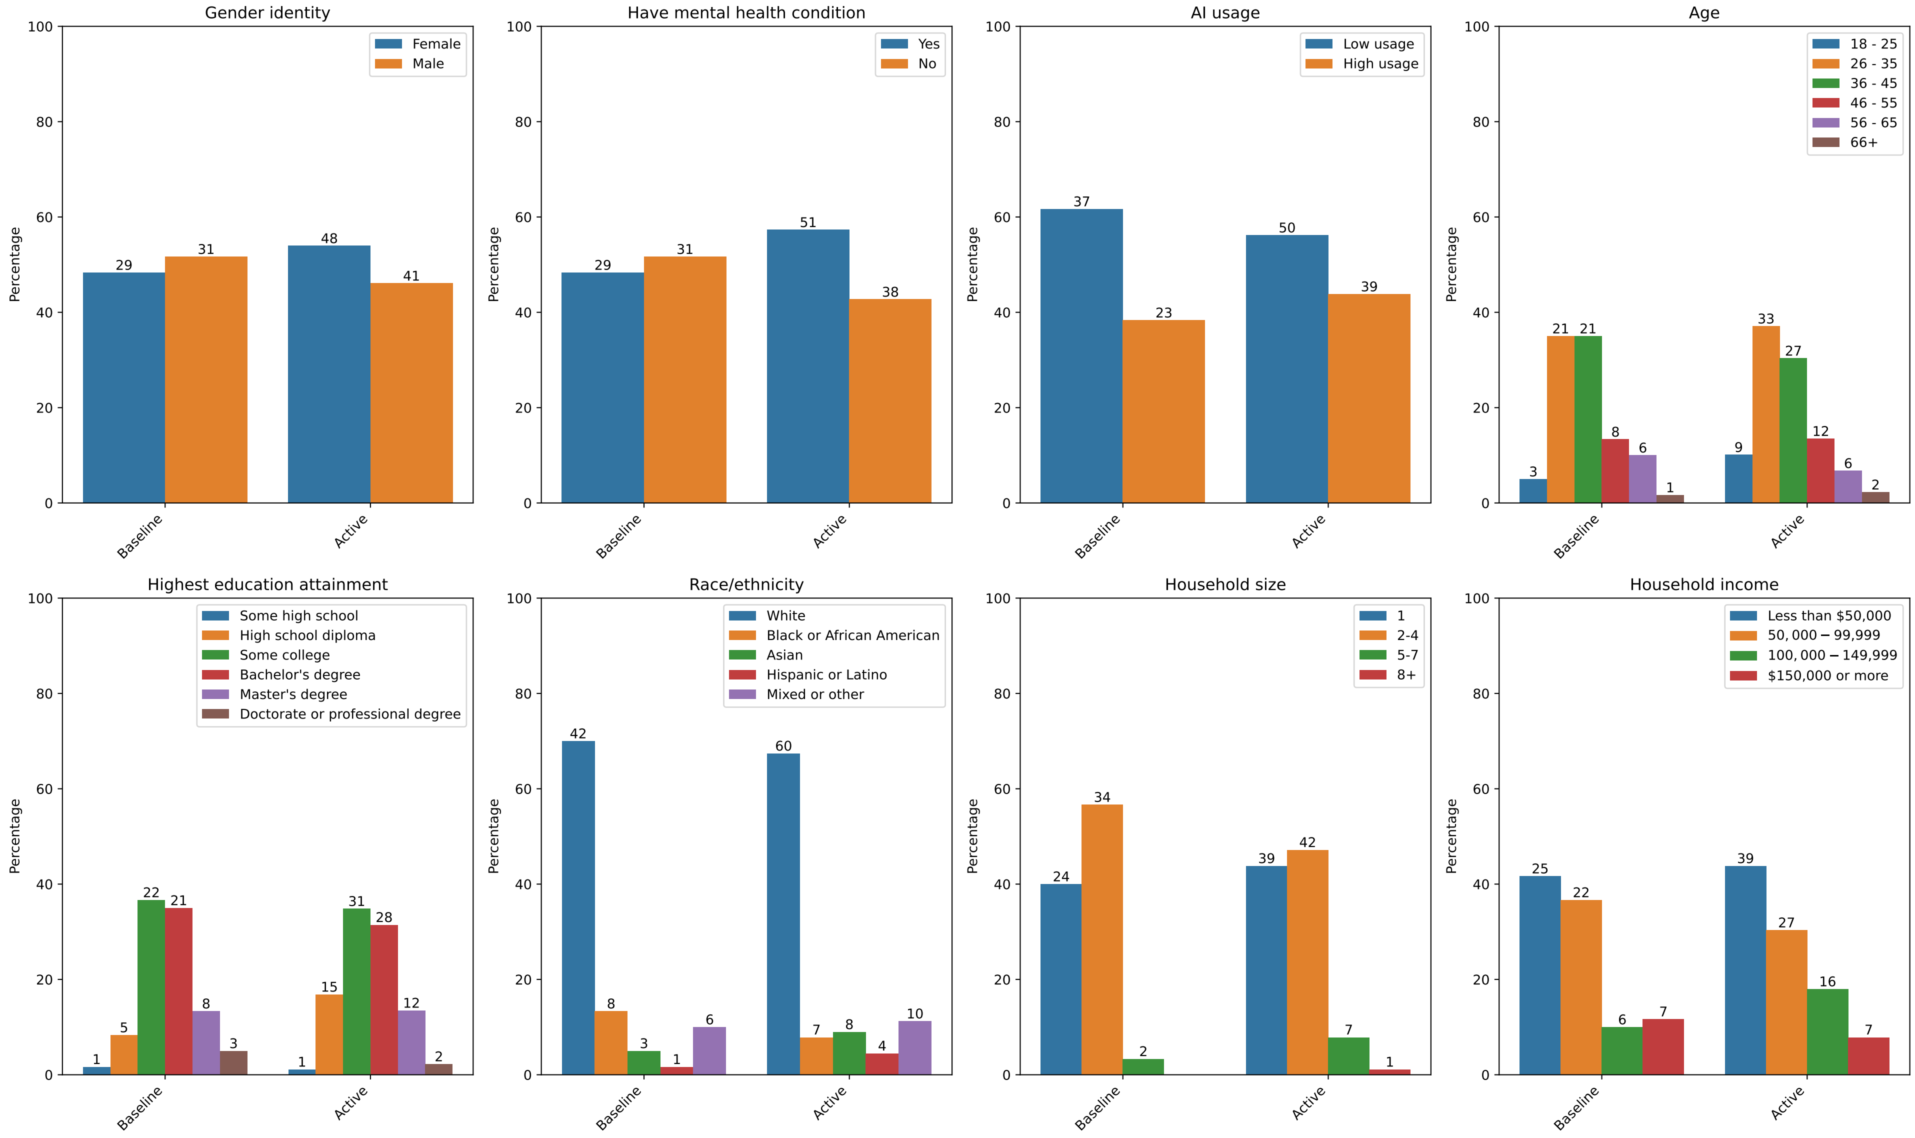

Figure 2: Distribution of intake psychometrics (impulsivity, loneliness, internal control) across baseline and active usage groups. Boxes represent quartile distribution within each group. Orange dots and numbers indicate the average, and orange lines represent 95% confidence intervals.

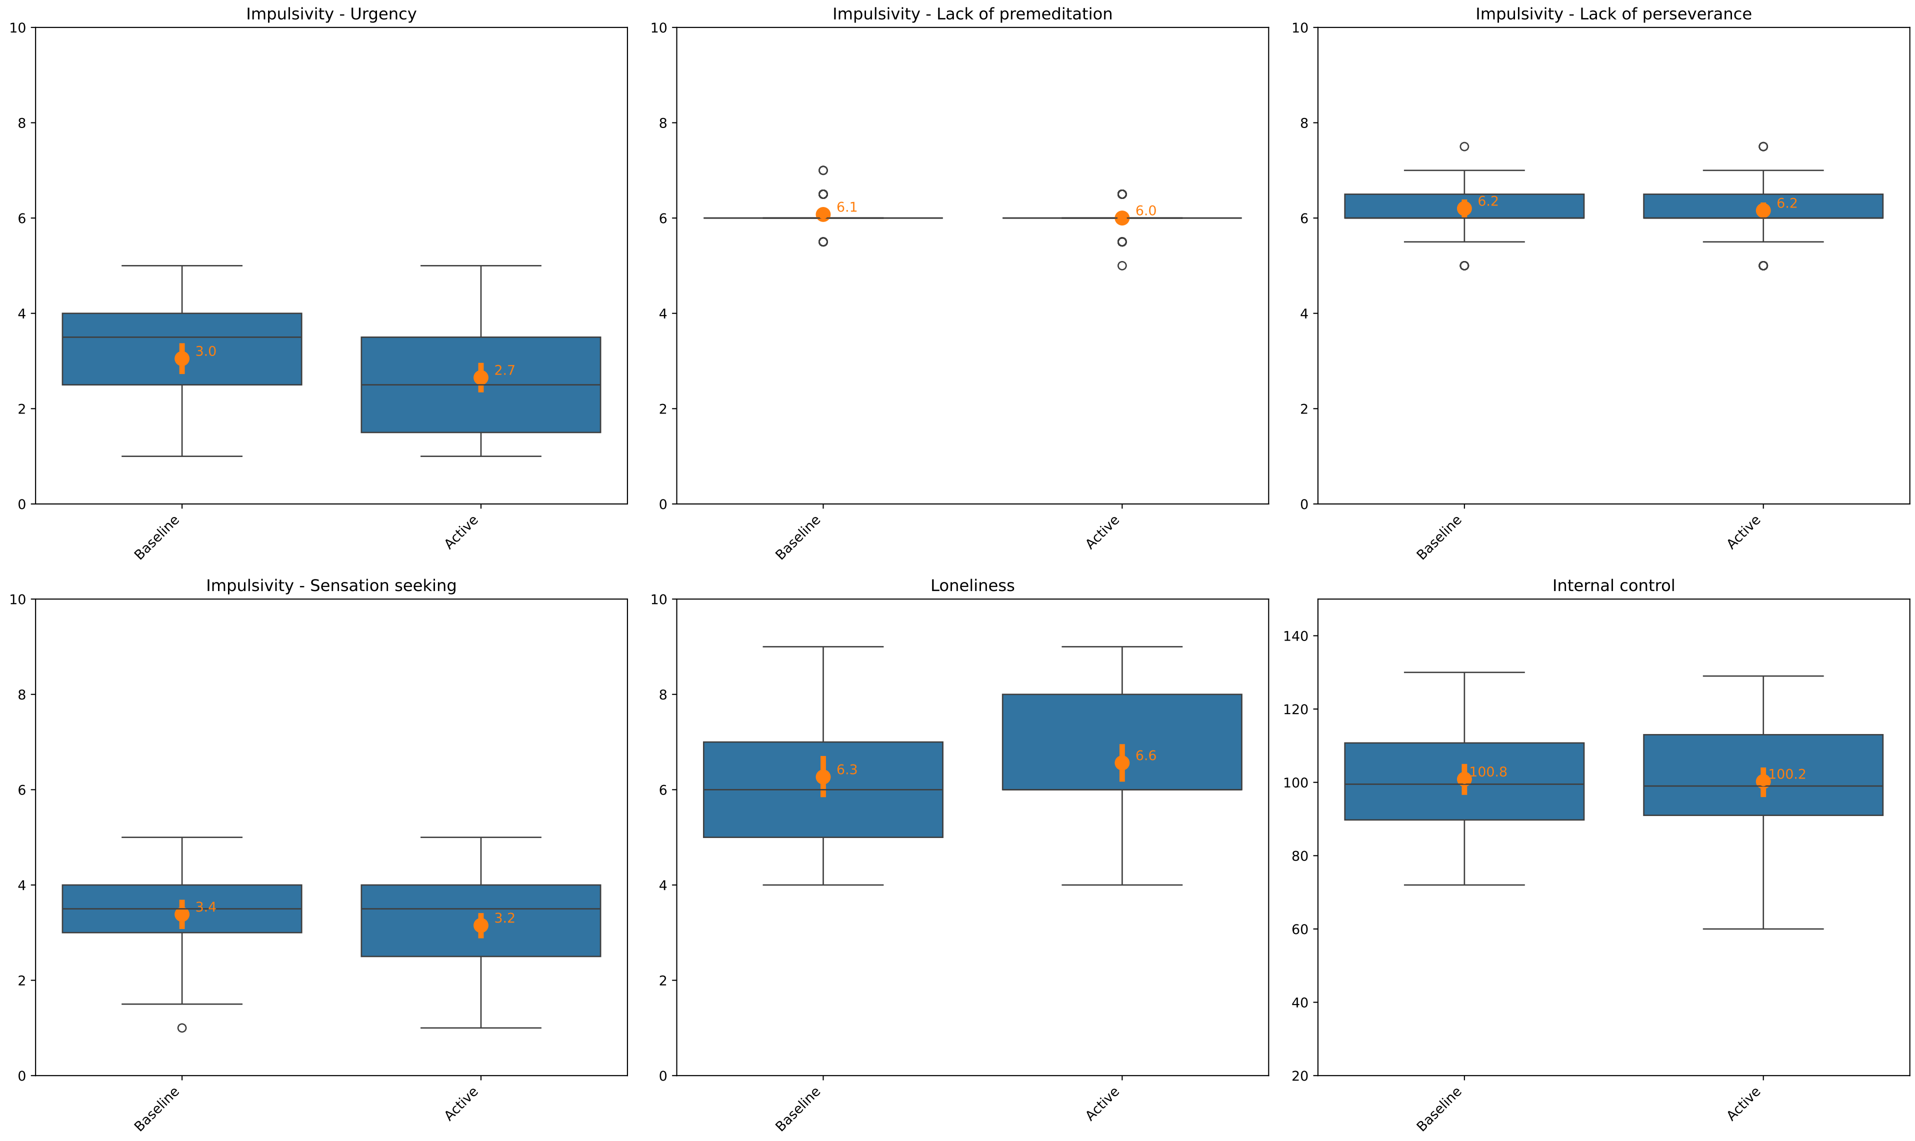

Figure 3: Distribution of participant demographics (gender identity, mental health condition, AI usage, age, education, race/ethnicity, household size, household income) across Platform groups. Boxes represent percentage within each group, and the numbers on top of boxes indicate the number of participants within each group.

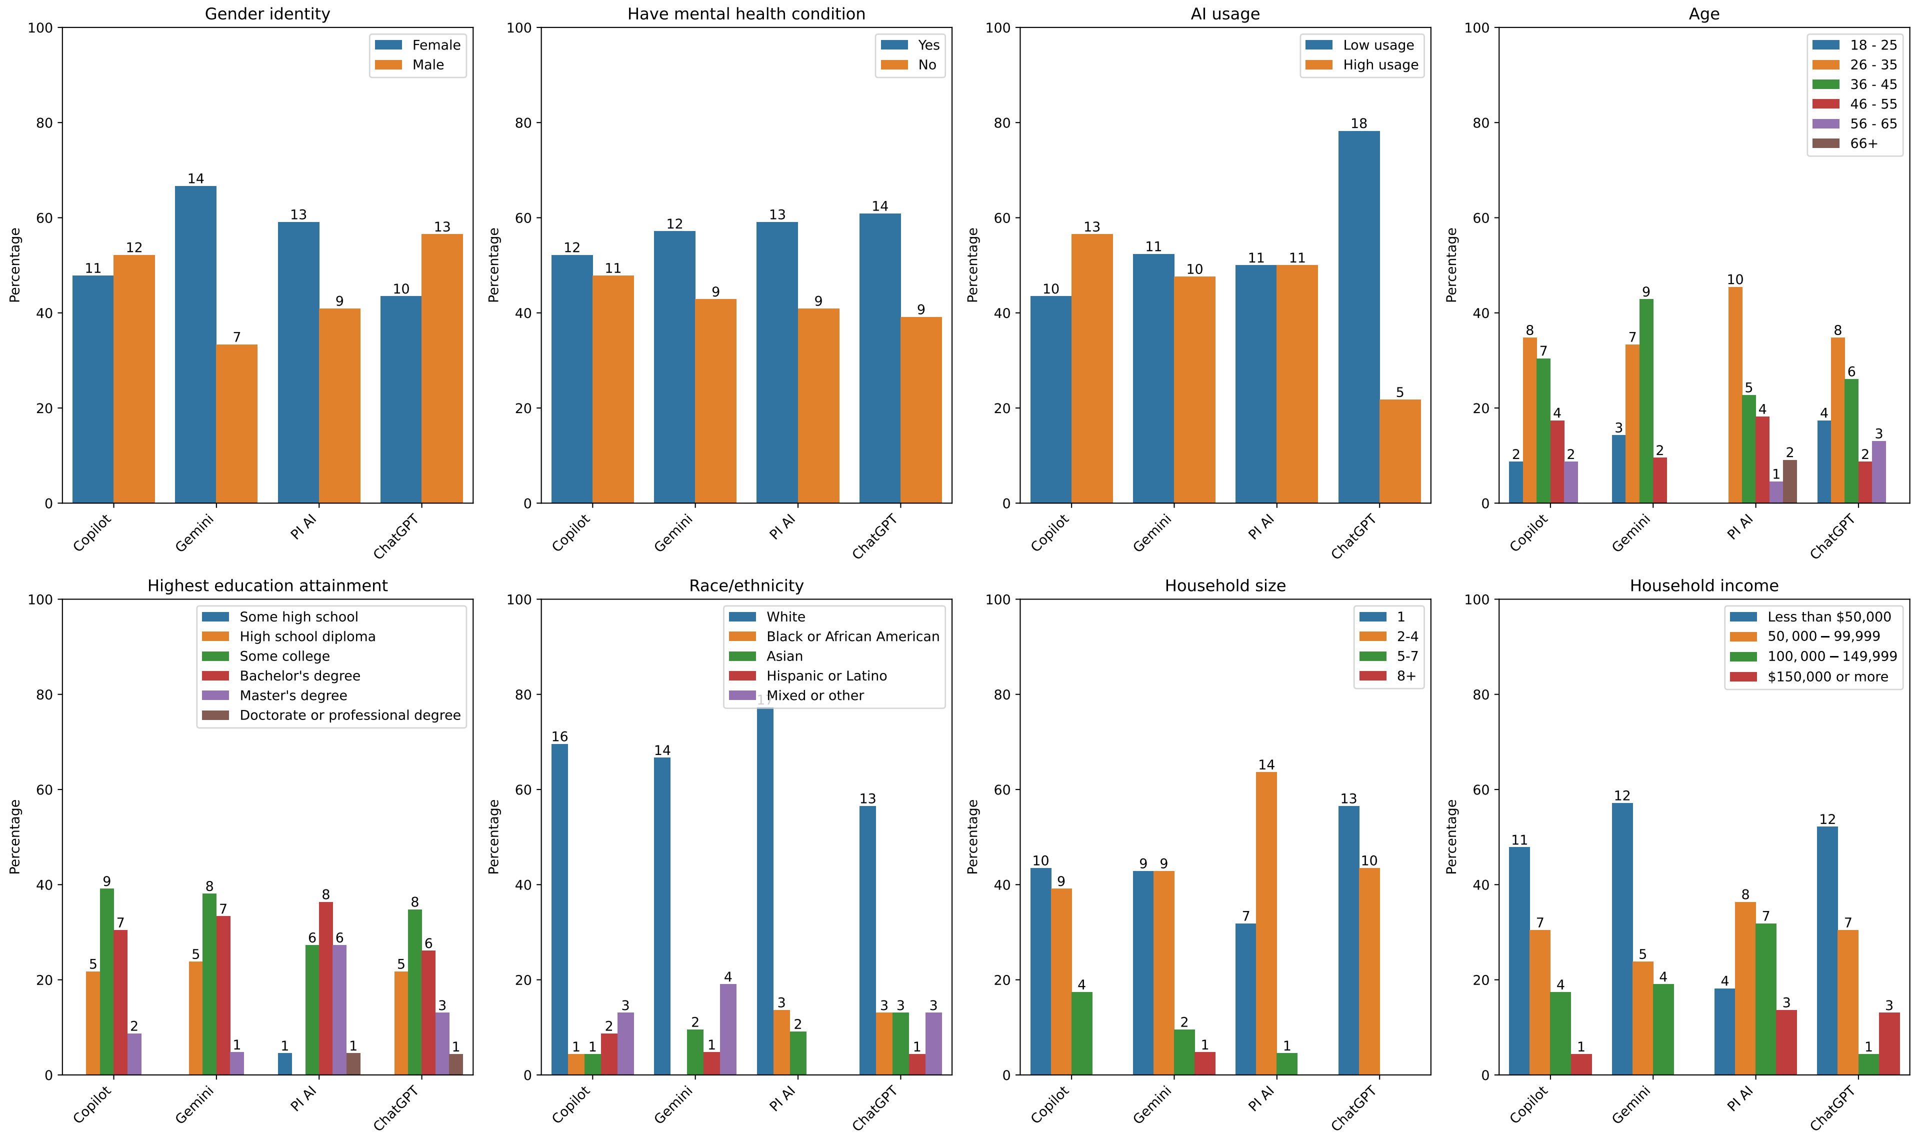

Figure 4: Distribution of intake psychometrics (impulsivity, loneliness, internal control) across Platform groups. Boxes represent quartile distribution within each group. Orange dots and numbers indicate the average, and orange lines represent 95% confidence intervals.

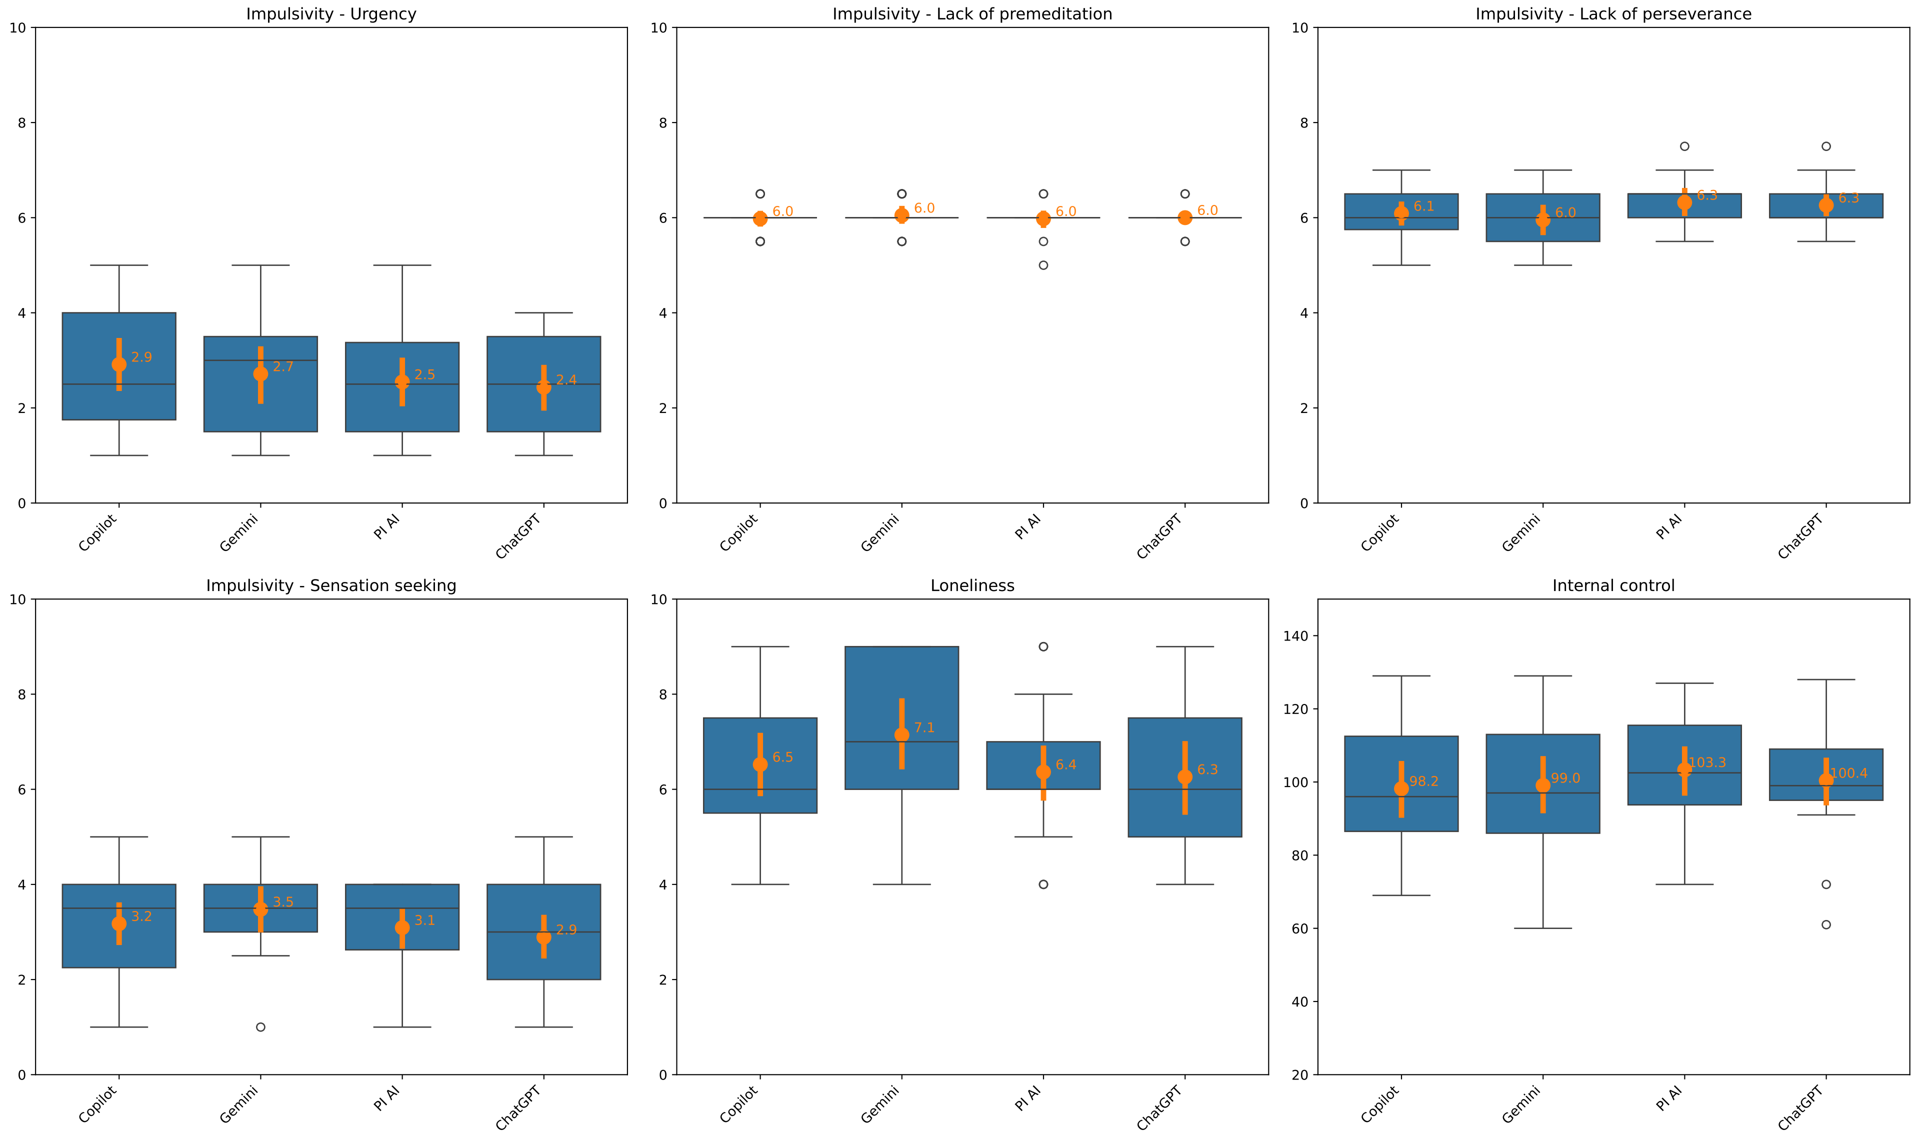

## Comparison of Perceptions at Study Start and End

Figure 5: Comparison of AI dependence subscales at study start and end across baseline and active usage groups. Bars represent average, and the error bars indicate 95% confidence intervals.

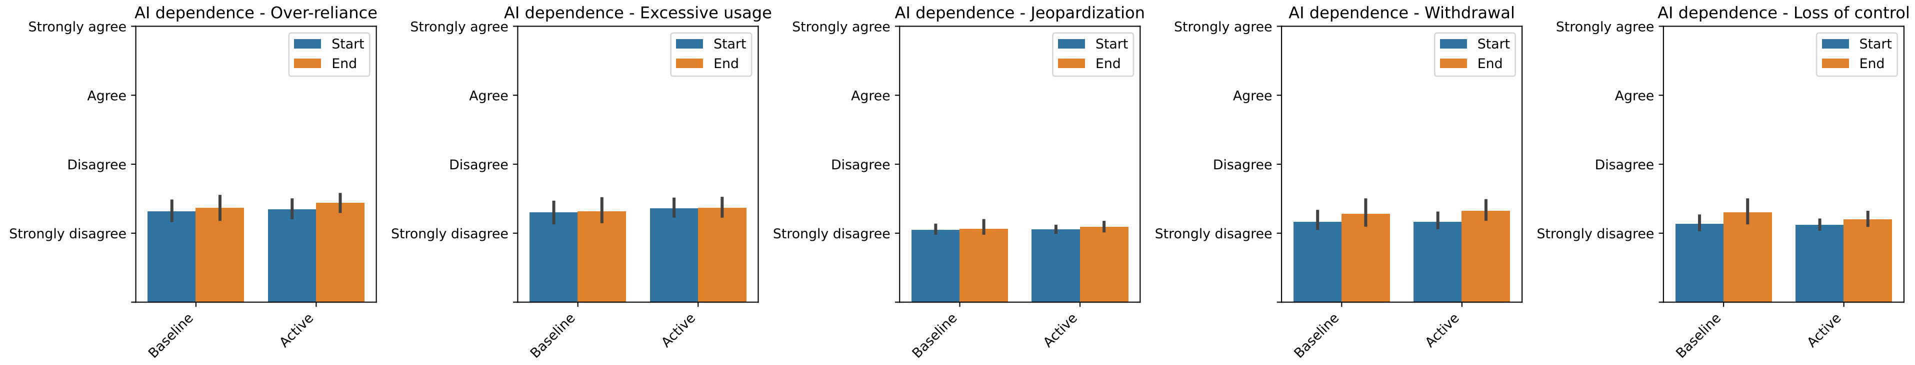


Figure 6: Comparison of AI attitude subscales at study start and end across baseline and active usage groups. Bars represent average, and the error bars indicate 95% confidence intervals.

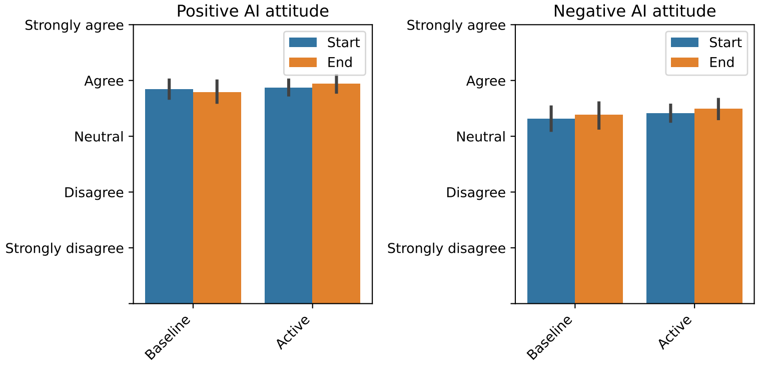

Figure 7: Comparison of interpersonal orientation at study start and end across baseline and active usage groups. Bars represent average, and the error bars indicate 95% confidence intervals.

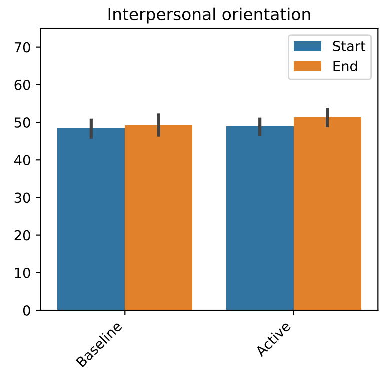


Figure 8: Comparison of AI use motivation subscales at study start and end across baseline and active usage groups. Bars represent average, and the error bars indicate 95% confidence intervals.

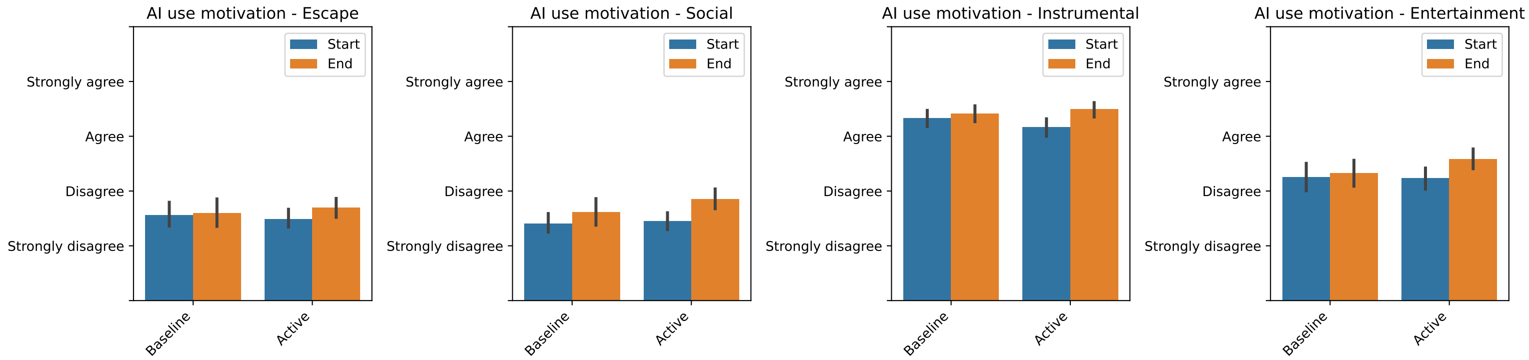

Figure 9: Comparison of attachment to AI, likely to recommend AI to others, satisfaction with AI, helpfulness of AI, and humanlikeness of AI at study start and end across baseline and active usage groups. Bars represent average, and the error bars indicate 95% confidence intervals.

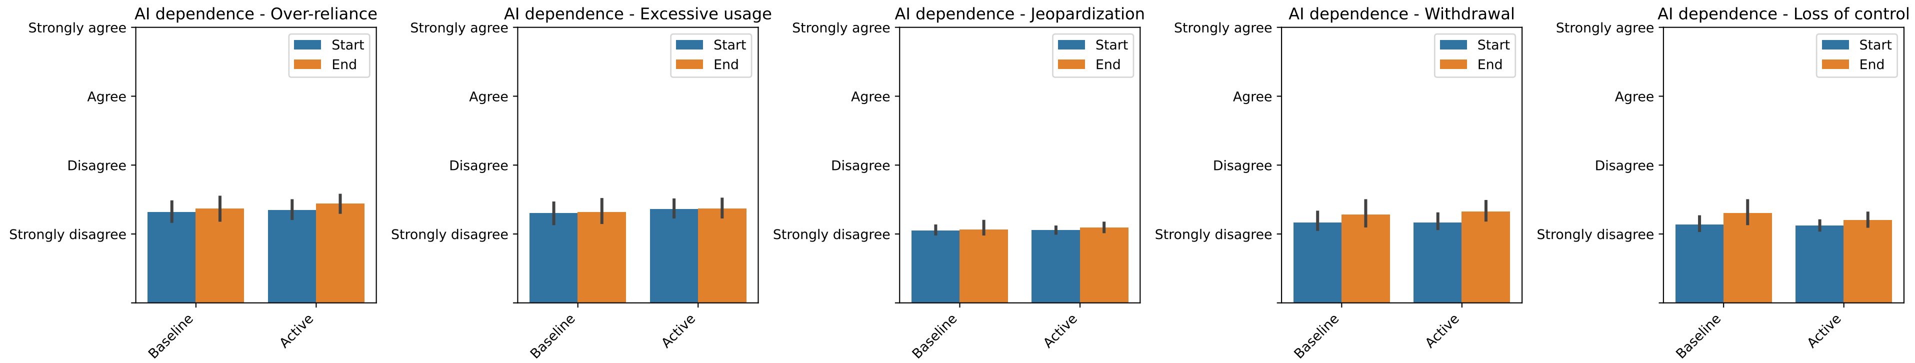


Figure 10: Comparison of perceived AI empathy at study start and end across baseline and active usage groups. Bars represent average, and the error bars indicate 95% confidence intervals.

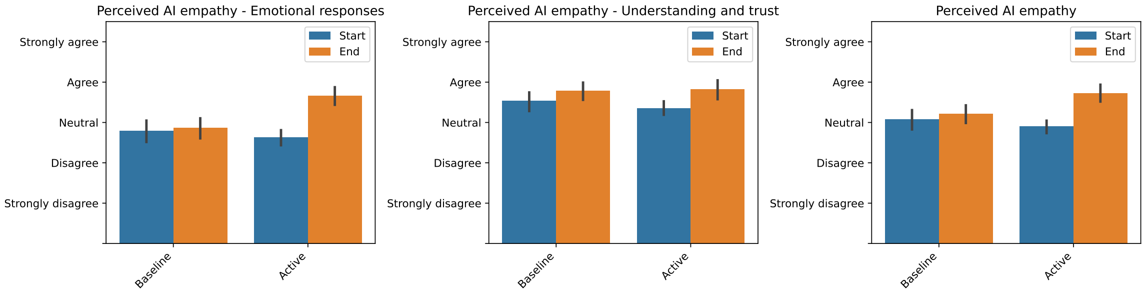

Figure 11: Comparison of AI dependence subscales at study start and end across Platform groups. Bars represent average, and the error bars indicate 95% confidence intervals.

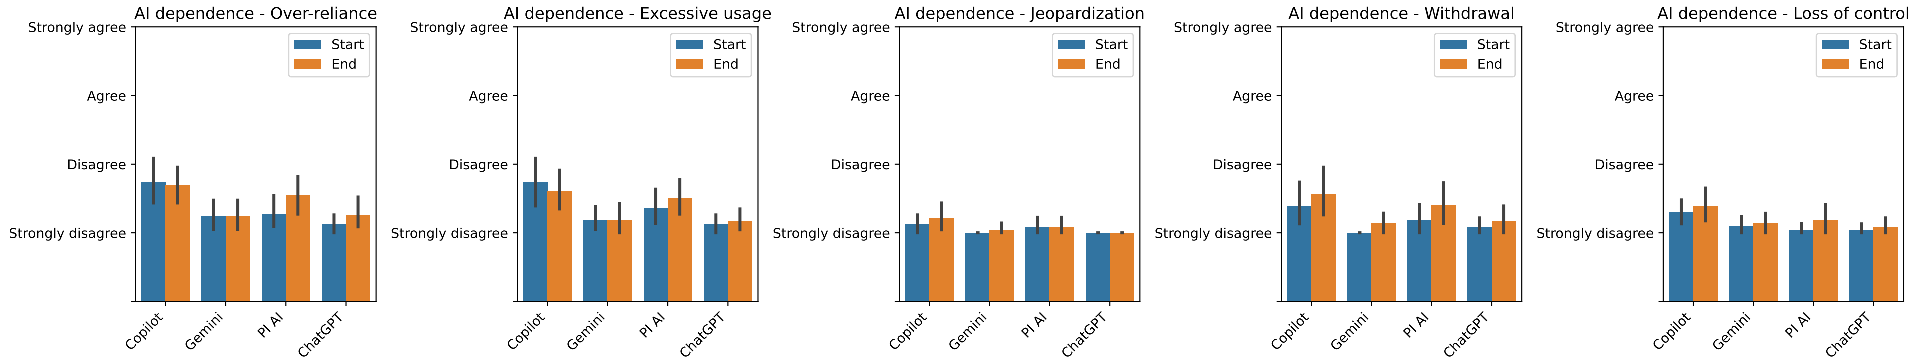


Figure 12: Comparison of AI attitude subscales at study start and end across Platform groups. Bars represent average, and the error bars indicate 95% confidence intervals.

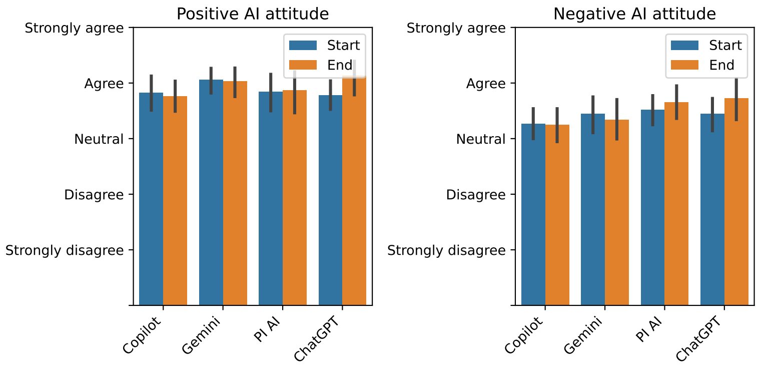

Figure 13: Comparison of interpersonal orientation at study start and end across Platform groups. Bars represent average, and the error bars indicate 95% confidence intervals.

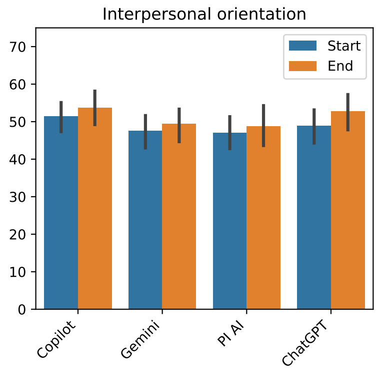


Figure 14: Comparison of AI use motivation subscales at study start and end across Platform groups. Bars represent average, and the error bars indicate 95% confidence intervals.

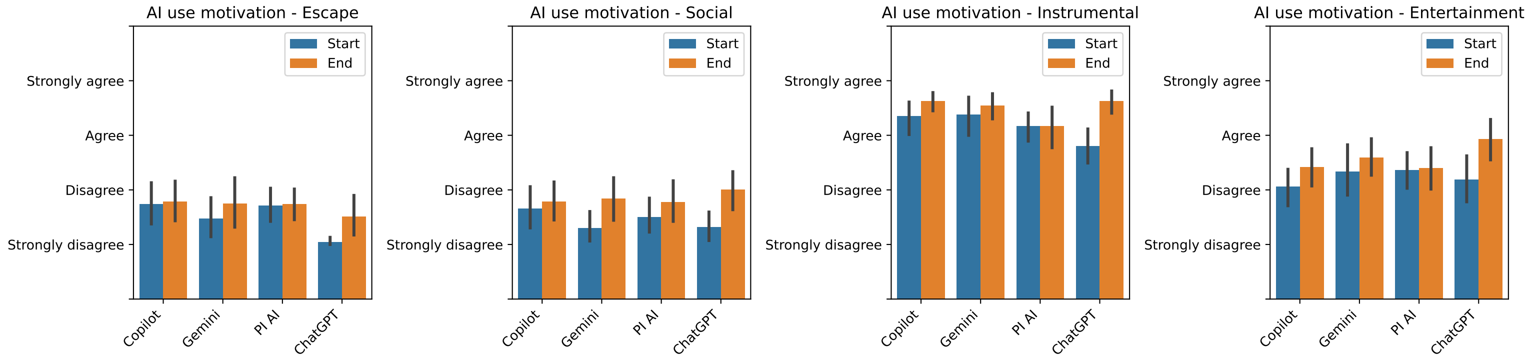

Figure 15: Comparison of attachment to AI, likely to recommend AI to others, satisfaction with AI, helpfulness of AI, and humanlikeness of AI at study start and end across Platform groups. Bars represent average, and the error bars indicate 95% confidence intervals.

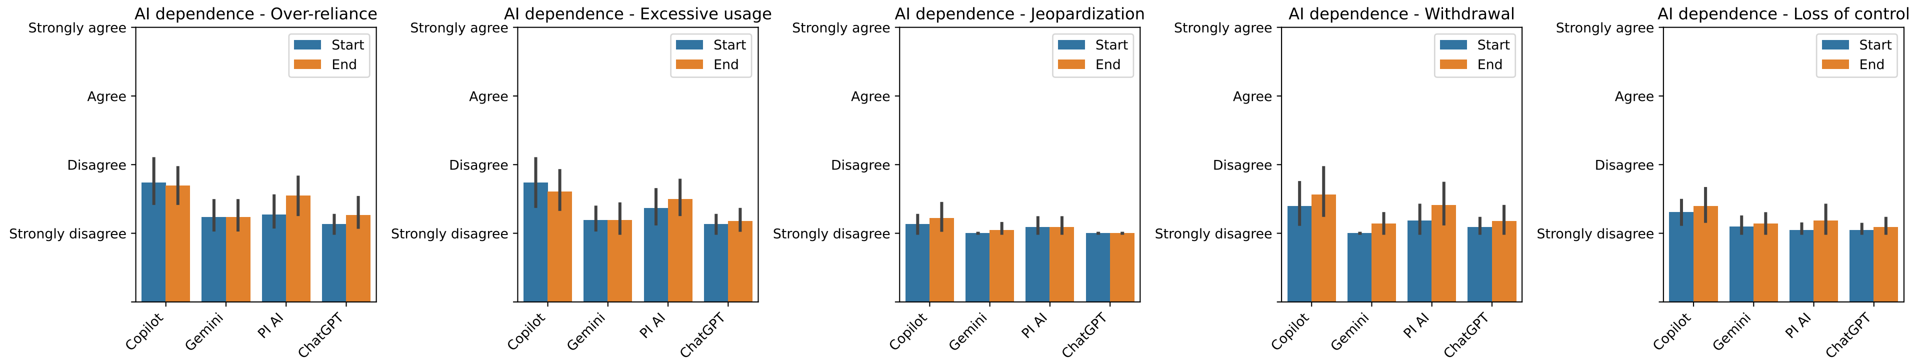


Figure 16: Comparison of perceived AI empathy at study start and end across Platform groups. Bars represent average, and the error bars indicate 95% confidence intervals.

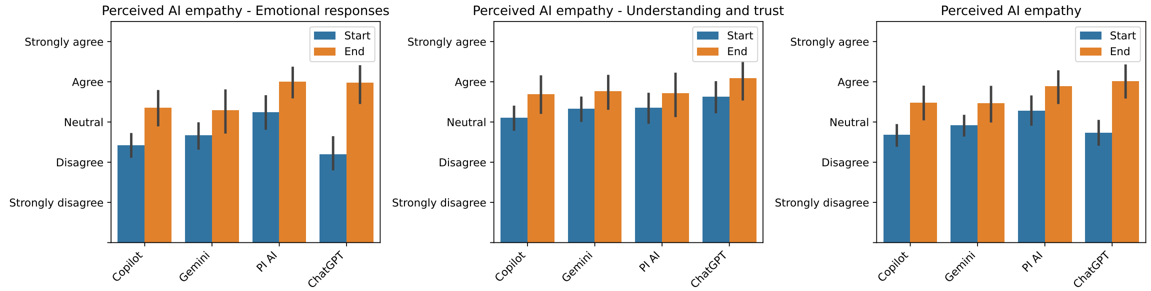

## Weekly Outcome Trends

Figure 17: Weekly trend of AI dependence subscales at study start and end across baseline and active usage groups. Dots represent average, and the error bars indicate 95% confidence intervals.

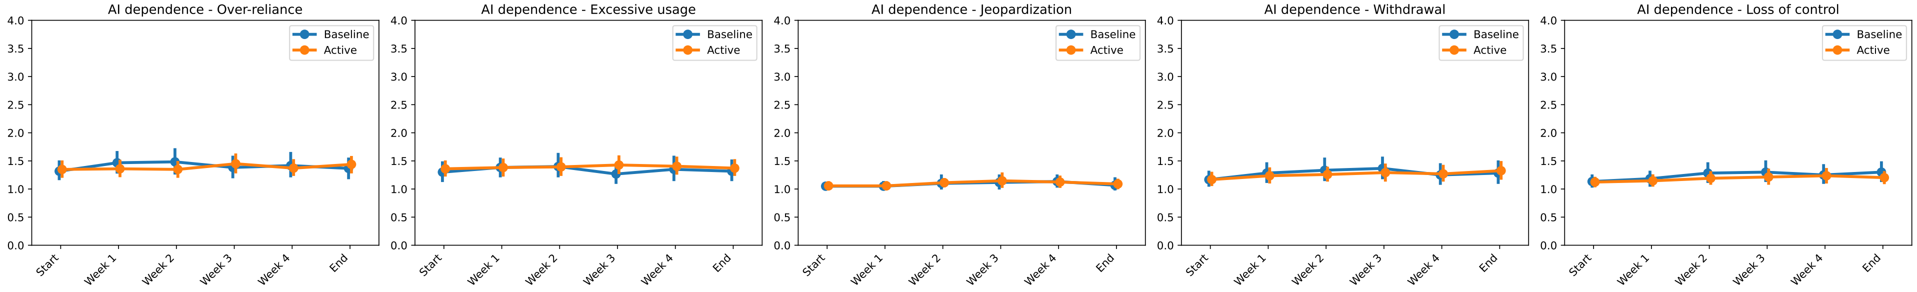


Figure 18: Weekly trend of AI attitude subscales at study start and end across baseline and active usage groups. Dots represent average, and the error bars indicate 95% confidence intervals.

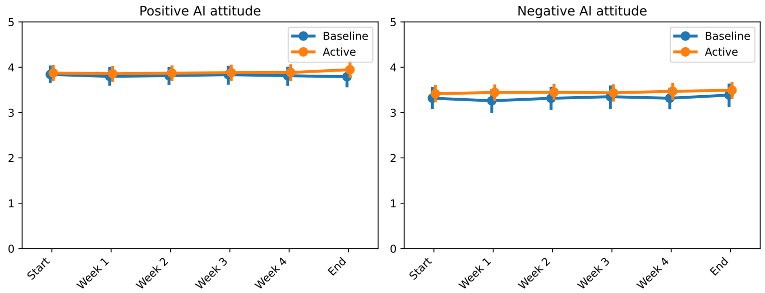

Figure 19: Weekly trend of interpersonal orientation at study start and end across baseline and active usage groups. Dots represent average, and the error bars indicate 95% confidence intervals.

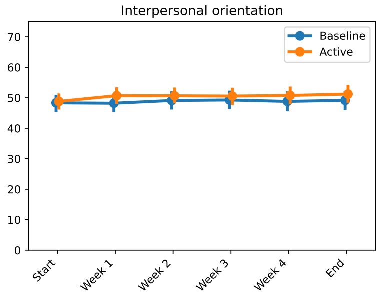


Figure 20: Weekly trend of AI use motivation subscales at study start and end across baseline and active usage groups. Each subscale presented is an average of 3 questions. Dots represent average, and the error bars indicate 95% confidence intervals.

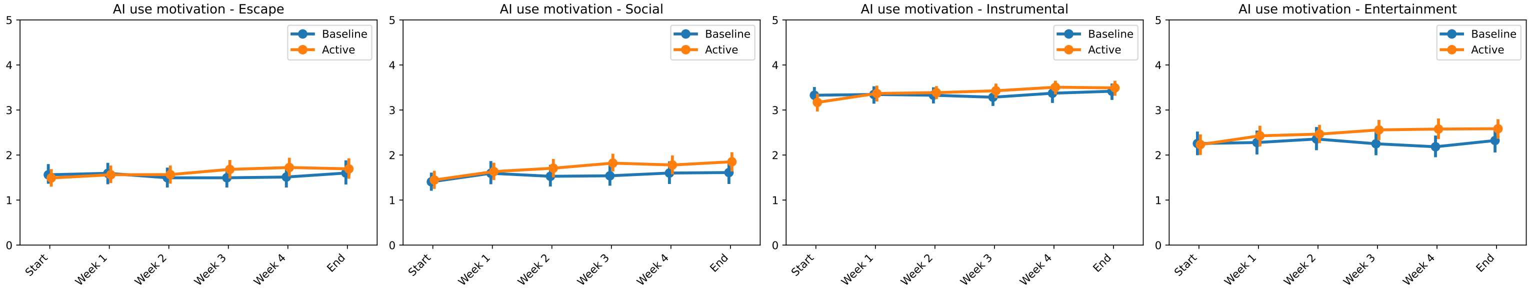

Figure 21: Weekly trend of attachment to AI, likely to recommend AI to others, satisfaction with AI, helpfulness of AI, and humanlikeness of AI at study start and end across baseline and active usage groups. Dots represent average, and the error bars indicate 95% confidence intervals.

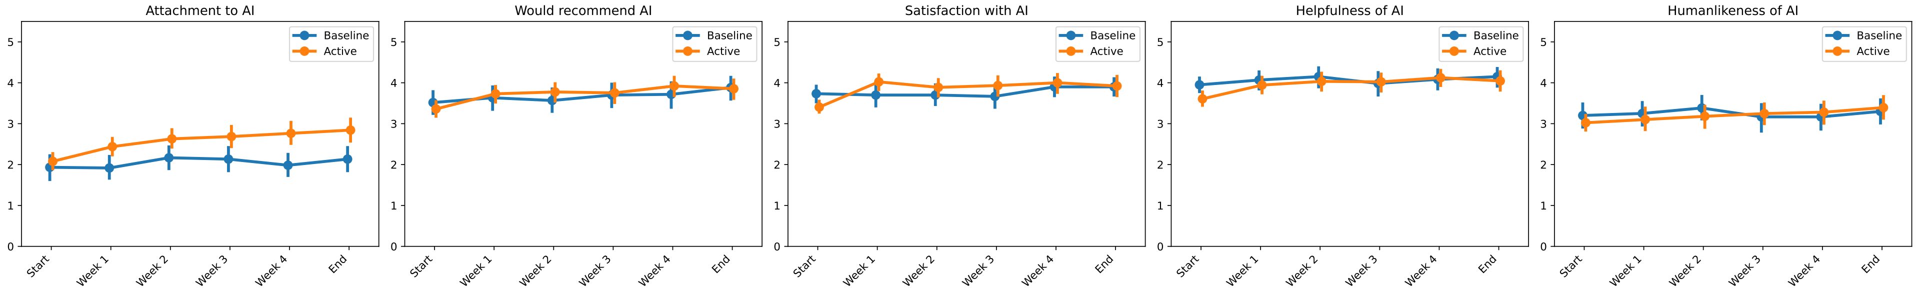


Figure 22: Weekly trend of perceived AI empathy at study start and end across baseline and active usage groups. Dots represent average, and the error bars indicate 95% confidence intervals.

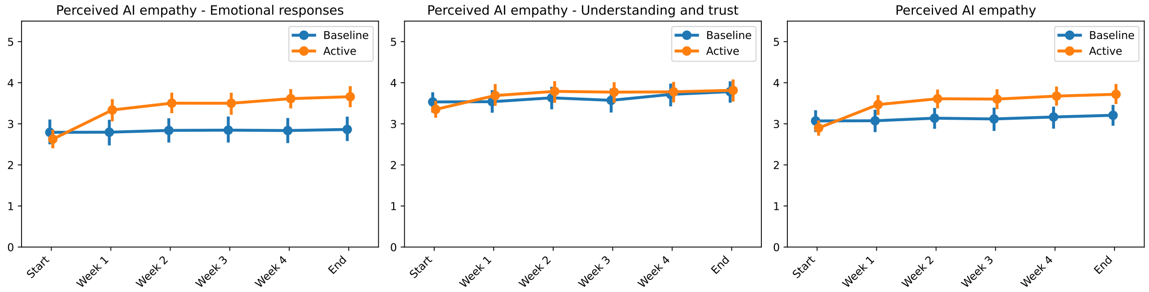

Figure 23: Weekly trend of AI dependence subscales at study start and end across Platform groups. Dots represent average, and the error bars indicate 95% confidence intervals.

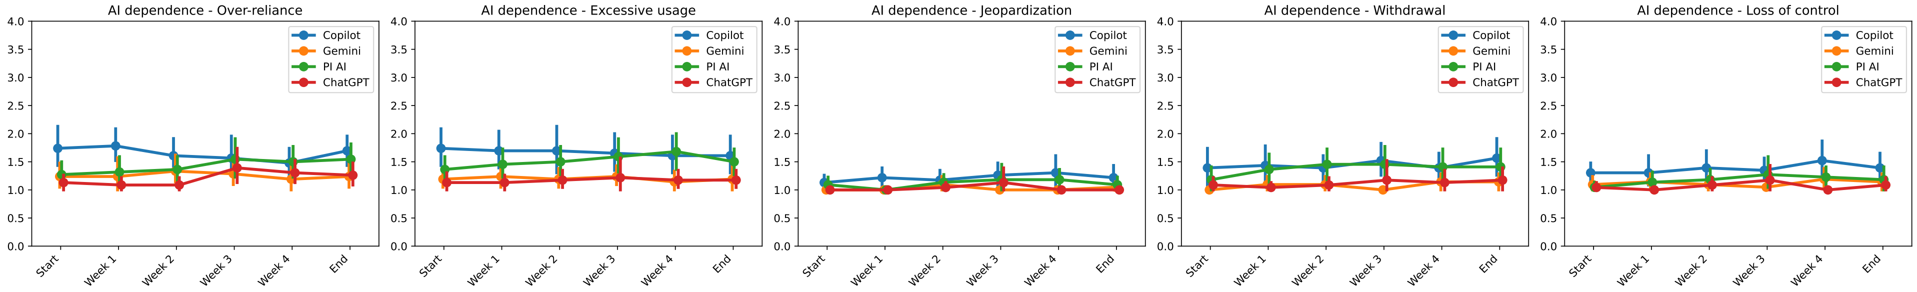


Figure 24: Weekly trend of AI attitude subscales at study start and end across Platform groups. Dots represent average, and the error bars indicate 95% confidence intervals.

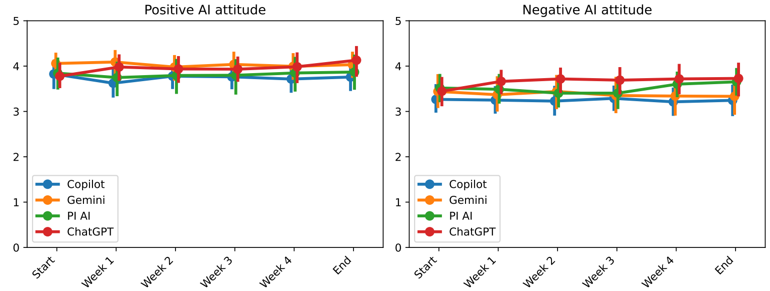

Figure 25: Weekly trend of interpersonal orientation at study start and end across Platform groups. Dots represent average, and the error bars indicate 95% confidence intervals.

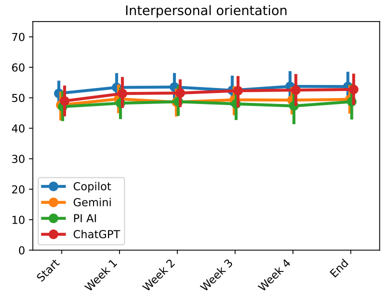


Figure 26: Weekly trend of AI use motivation subscales at study start and end across Platform groups. Dots represent average, and the error bars indicate 95% confidence intervals.

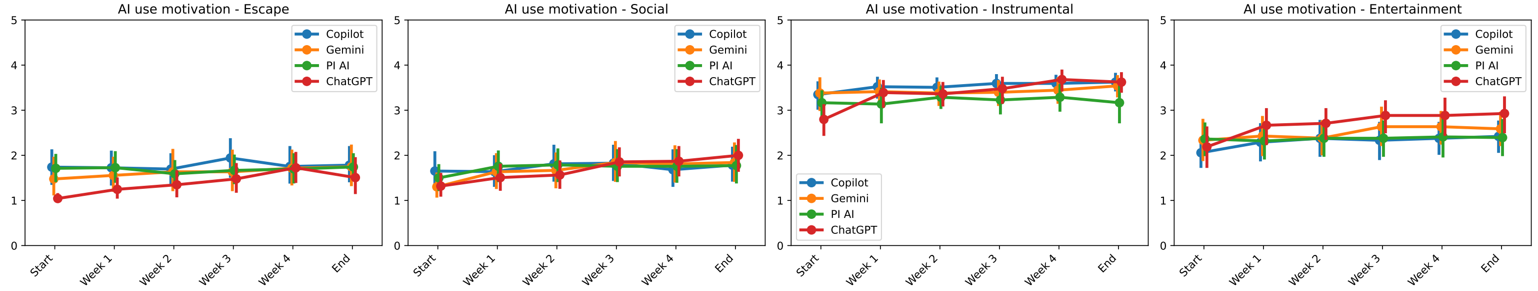

Figure 27: Weekly trend of attachment to AI, likely to recommend AI to others, satisfaction with AI, helpfulness of AI, and humanlikeness of AI at study start and end across Platform groups. Dots represent average, and the error bars indicate 95% confidence intervals.

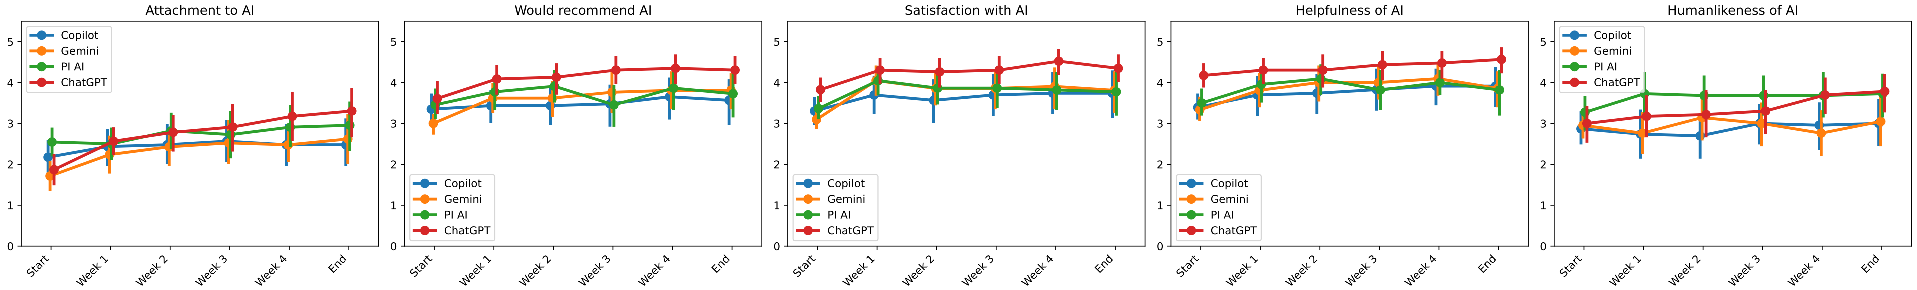


Figure 28: Weekly trend of perceived AI empathy at study start and end across Platform groups. Dots represent average, and the error bars indicate 95% confidence intervals.

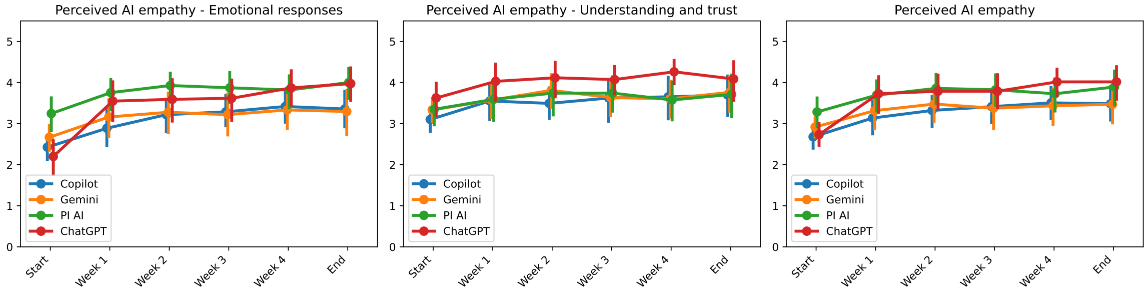

## Difference in Difference Analysis Results

| Perception Variable | Relative Change | CI | p-value | w/t-stat | Effect size |
|---|---|---|---|---|---|
| Attachment towards AI | 27.78% | [12.34%, 43.22%] | 0.062 | 211.00 | 0.18 |
| Perceived AI empathy | 8.93% | [1.01%, 16.86%] | 0.079 | 1.79 | 0.15 |
| Satisfaction with AI | 6.61% | [-0.03%, 13.26%] | 0.067 | 92.00 | 0.21 |
| Motivation for using AI (Entertainment) | 9.17% | [-2.14%, 20.48%] | 0.51 | 400.00 | 0.07 |
| Motivation for using AI (Escape) | 9.46% | [-4.52%, 23.45%] | 0.7 | 173.00 | 0.04 |
| Motivation for using AI (Social) | 20.31% | [3.62%, 36.99%] | 0.05 | 74.00 | 0.25 |
| Motivation for using AI (Instrumental) | 5.33% | [-1.39%, 12.06%] | 0.311 | 197.00 | 0.15 |
| Dependence on AI | 9.68% | [-0.26%, 19.63%] | 0.383 | 153.00 | 0.16 |
| Dependence on AI (Over-reliance) | 10.28% | [-1.75%, 22.3%] | 0.559 | 73.00 | 0.08 |
| Dependence on AI (Excessive Usage) | 9.72% | [-2.84%, 22.29%] | 0.84 | 100.00 | 0.03 |
| Dependence on AI (Jeopardization) | 4.17% | [-6.81%, 15.14%] | 1.0 | 7.50 | 0.05 |
| Dependence on AI (Withdrawal) | 16.11% | [-0.36%, 32.59%] | 0.221 | 28.50 | 0.19 |
| Dependence on AI (Loss of Control) | 18.33% | [4.89%, 31.78%] | 0.04 | 26.00 | 0.32 |
| Interpersonal Orientation | 2.22% | [-1.27%, 5.7%] | 0.119 | 654.50 | 0.08 |
| AI Helpfulness | 7.17% | [0.28%, 14.05%] | 0.059 | 160.50 | 0.25 |
| Perceived Human-Like Behavior | 8.44% | [-1.31%, 18.2%] | 0.389 | 221.00 | 0.09 |
| Recommendation to use AI | 21.81% | [3.03%, 40.58%] | 0.013 | 107.50 | 0.34 |
| Attitude towards AI | 0.44% | [-2.34%, 3.21%] | 0.831 | 0.21 | 0.01 |
| Attitude towards AI (Positive) | -1.1% | [-4.34%, 2.15%] | 0.386 | 503.50 | -0.07 |
| Attitude towards AI (Negative) | 3.46% | [-1.96%, 8.88%] | 0.33 | 0.98 | 0.08 |

Table 1: Control Relative Change

| Perception Variable | Relative Change | CI | p-value | w/t-stat | Effect size |
|---|---|---|---|---|---|
| Attachment towards AI | 60.77% | [37.56%, 83.98%] | <0.001 | 297.00 | 0.66 |
| Perceived AI empathy | 34.73% | [23.51%, 45.95%] | <0.001 | 7.99 | 0.92 |
| Satisfaction with AI | 17.87% | [9.85%, 25.88%] | <0.001 | 562.00 | 0.54 |
| Motivation for using AI (Entertainment) | 32.07% | [17.31%, 46.83%] | <0.001 | 439.50 | 0.39 |
| Motivation for using AI (Escape) | 24.35% | [10.84%, 37.87%] | 0.028 | 308.00 | 0.24 |
| Motivation for using AI (Social) | 38.22% | [24.71%, 51.73%] | <0.001 | 126.50 | 0.49 |
| Motivation for using AI (Instrumental) | 17.56% | [8.07%, 27.06%] | <0.001 | 279.00 | 0.45 |
| Dependence on AI | 8.96% | [2.77%, 15.16%] | 0.073 | 343.50 | 0.19 |
| Dependence on AI (Over-reliance) | 15.26% | [4.03%, 26.49%] | 0.185 | 97.00 | 0.14 |
| Dependence on AI (Excessive Usage) | 8.61% | [-0.6%, 17.83%] | 0.862 | 272.00 | 0.02 |
| Dependence on AI (Jeopardization) | 3.93% | [-0.89%, 8.76%] | 0.257 | 8.00 | 0.12 |
| Dependence on AI (Withdrawal) | 18.35% | [7.53%, 29.17%] | 0.016 | 57.00 | 0.27 |
| Dependence on AI (Loss of Control) | 8.99% | [1.97%, 16.01%] | 0.071 | 32.00 | 0.2 |
| Interpersonal Orientation | 5.37% | [2.96%, 7.78%] | <0.001 | 4.56 | 0.22 |
| AI Helpfulness | 14.91% | [7.57%, 22.25%] | <0.001 | 569.00 | 0.47 |
| Perceived Human-Like Behavior | 23.13% | [7.31%, 38.95%] | 0.014 | 661.00 | 0.33 |
| Recommendation to use AI | 18.56% | [10.63%, 26.49%] | <0.001 | 448.00 | 0.5 |
| Attitude towards AI | 2.27% | [-0.21%, 4.76%] | 0.102 | 1565.50 | 0.12 |
| Attitude towards AI (Positive) | 2.11% | [-0.52%, 4.74%] | 0.105 | 1.64 | 0.1 |
| Attitude towards AI (Negative) | 2.53% | [-0.78%, 5.83%] | 0.141 | 1.48 | 0.1 |

Table 2: Active Usage Relative Change

| Perception Variable | Relative Change | CI | p-value | w/t-stat | Effect size |
|---|---|---|---|---|---|
| Attachment towards AI | 41.67% | [-3.72%, 87.05%] | 0.374 | 0.91 | 0.26 |
| Perceived AI empathy | 38.18% | [9.35%, 67.0%] | <0.001 | 3.92 | 0.95 |
| Satisfaction with AI | 17.75% | [-2.61%, 38.12%] | 0.113 | 44.00 | 0.41 |
| Motivation for using AI (Entertainment) | 28.89% | [6.77%, 51.0%] | 0.008 | 2.93 | 0.45 |
| Motivation for using AI (Escape) | 10.58% | [-6.69%, 27.86%] | 0.844 | 36.50 | 0.05 |
| Motivation for using AI (Social) | 19.08% | [-4.2%, 42.37%] | 0.337 | 14.50 | 0.14 |
| Motivation for using AI (Instrumental) | 15.58% | [-2.61%, 33.77%] | 0.016 | 18.50 | 0.46 |
| Dependence on AI | 5.87% | [-6.97%, 18.72%] | 0.915 | 44.00 | 0.07 |
| Dependence on AI (Over-reliance) | 4.71% | [-14.26%, 23.68%] | 0.705 | 4.00 | -0.06 |
| Dependence on AI (Excessive Usage) | -2.17% | [-17.08%, 12.73%] | 0.317 | 15.00 | -0.16 |
| Dependence on AI (Jeopardization) | 6.52% | [-3.37%, 16.42%] | 0.157 | 0.00 | 0.2 |
| Dependence on AI (Withdrawal) | 24.64% | [-4.83%, 54.1%] | 0.271 | 10.50 | 0.22 |
| Dependence on AI (Loss of Control) | 8.7% | [-5.37%, 22.76%] | 0.317 | 2.50 | 0.17 |
| Interpersonal Orientation | 5.07% | [-1.31%, 11.45%] | 0.066 | 1.93 | 0.22 |
| AI Helpfulness | 21.23% | [1.47%, 40.99%] | 0.152 | 60.50 | 0.55 |
| Perceived Human-Like Behavior | 15.94% | [-17.77%, 49.66%] | 0.7 | 0.39 | 0.11 |
| Recommendation to use AI | 11.01% | [-8.02%, 30.05%] | 0.369 | 58.00 | 0.2 |
| Attitude towards AI | -0.68% | [-5.26%, 3.9%] | 0.846 | 131.00 | -0.07 |
| Attitude towards AI (Positive) | -0.89% | [-6.06%, 4.29%] | 0.415 | -0.83 | -0.1 |
| Attitude towards AI (Negative) | 0.03% | [-6.68%, 6.74%] | 0.97 | 104.00 | -0.03 |

Table 3: Copilot Relative Change

| Perception Variable | Relative Change | CI | p-value | w/t-stat | Effect size |
|---|---|---|---|---|---|
| Attachment towards AI | 72.22% | [24.52%, 119.92%] | 0.005 | 3.19 | 0.84 |
| Perceived AI empathy | 19.37% | [5.97%, 32.76%] | 0.006 | 3.09 | 0.66 |
| Satisfaction with AI | 23.81% | [6.96%, 40.66%] | 0.013 | 42.00 | 0.83 |
| Motivation for using AI (Entertainment) | 31.36% | [-1.31%, 64.03%] | 0.205 | 1.31 | 0.27 |
| Motivation for using AI (Escape) | 24.08% | [-1.65%, 49.81%] | 0.091 | 11.00 | 0.29 |
| Motivation for using AI (Social) | 48.84% | [17.03%, 80.66%] | 0.015 | 6.00 | 0.71 |
| Motivation for using AI (Instrumental) | 12.31% | [-5.63%, 30.25%] | 0.23 | 12.50 | 0.23 |
| Dependence on AI | 6.63% | [-6.45%, 19.7%] | 0.528 | 7.50 | 0.18 |
| Dependence on AI (Over-reliance) | 3.97% | [-9.15%, 17.09%] | 1.0 | 3.00 | 0.0 |
| Dependence on AI (Excessive Usage) | 4.76% | [-12.73%, 22.25%] | 1.0 | 10.50 | 0.0 |
| Dependence on AI (Jeopardization) | 4.76% | [-5.17%, 14.7%] | 0.317 | 0.00 | 0.32 |
| Dependence on AI (Withdrawal) | 14.29% | [-2.04%, 30.61%] | 0.083 | 0.00 | 0.58 |
| Dependence on AI (Loss of Control) | 9.52% | [-8.99%, 28.04%] | 0.655 | 6.00 | 0.15 |
| Interpersonal Orientation | 4.86% | [0.12%, 9.59%] | 0.087 | 1.80 | 0.19 |
| AI Helpfulness | 18.49% | [2.73%, 34.25%] | 0.027 | 28.00 | 0.65 |
| Perceived Human-Like Behavior | 5.56% | [-18.33%, 29.44%] | 0.741 | 0.34 | 0.09 |
| Recommendation to use AI | 28.97% | [12.71%, 45.22%] | 0.003 | 10.00 | 1.01 |
| Attitude towards AI | -1.73% | [-4.8%, 1.34%] | 0.223 | -1.26 | -0.12 |
| Attitude towards AI (Positive) | -0.6% | [-4.36%, 3.17%] | 0.952 | 93.50 | -0.05 |
| Attitude towards AI (Negative) | -3.3% | [-8.57%, 1.97%] | 0.222 | -1.26 | -0.13 |

Table 4: Gemini Relative Change

| Perception Variable | Relative Change | CI | p-value | w/t-stat | Effect size |
|---|---|---|---|---|---|
| Attachment towards AI | 19.7% | [-1.16%, 40.55%] | 0.137 | 17.00 | 0.39 |
| Perceived AI empathy | 22.58% | [8.7%, 36.45%] | 0.003 | 3.35 | 0.67 |
| Satisfaction with AI | 14.7% | [-4.13%, 33.53%] | 0.213 | 44.50 | 0.4 |
| Motivation for using AI (Entertainment) | 3.13% | [-7.57%, 13.83%] | 0.49 | 30.50 | 0.04 |
| Motivation for using AI (Escape) | 18.26% | [-11.17%, 47.69%] | 0.881 | 0.15 | 0.04 |
| Motivation for using AI (Social) | 20.37% | [2.48%, 38.27%] | 0.049 | 8.50 | 0.33 |
| Motivation for using AI (Instrumental) | -1.31% | [-11.66%, 9.05%] | 0.936 | 38.00 | 0.0 |
| Dependence on AI | 14.89% | [2.82%, 26.95%] | 0.047 | 2.11 | 0.43 |
| Dependence on AI (Over-reliance) | 32.58% | [1.94%, 63.21%] | 0.107 | 7.00 | 0.45 |
| Dependence on AI (Excessive Usage) | 21.21% | [-2.73%, 45.15%] | 0.366 | 24.00 | 0.24 |
| Dependence on AI (Jeopardization) | 4.55% | [-10.61%, 19.7%] | 1.0 | 5.00 | 0.0 |
| Dependence on AI (Withdrawal) | 21.21% | [1.57%, 40.85%] | 0.096 | 3.00 | 0.37 |
| Dependence on AI (Loss of Control) | 11.36% | [-2.2%, 24.93%] | 0.083 | 0.00 | 0.36 |
| Interpersonal Orientation | 3.16% | [-1.9%, 8.23%] | 0.162 | 1.45 | 0.14 |
| AI Helpfulness | 9.09% | [-6.29%, 24.47%] | 0.21 | 39.00 | 0.32 |
| Perceived Human-Like Behavior | 25.0% | [-6.93%, 56.93%] | 0.106 | 1.69 | 0.42 |
| Recommendation to use AI | 10.3% | [-6.79%, 27.4%] | 0.35 | 44.00 | 0.26 |
| Attitude towards AI | 2.08% | [-2.49%, 6.65%] | 0.291 | 1.08 | 0.12 |
| Attitude towards AI (Positive) | 0.06% | [-5.39%, 5.52%] | 0.772 | 0.29 | 0.03 |
| Attitude towards AI (Negative) | 4.48% | [-1.18%, 10.14%] | 0.154 | 1.48 | 0.2 |

Table 5: PI AI Relative Change

| Perception Variable | Relative Change | CI | p-value | w/t-stat | Effect size |
|---|---|---|---|---|---|
| Attachment towards AI | 108.7% | [46.25%, 171.14%] | 0.001 | 0.00 | 1.24 |
| Perceived AI empathy | 56.94% | [28.66%, 85.22%] | <0.001 | 5.77 | 1.5 |
| Satisfaction with AI | 15.58% | [5.37%, 25.79%] | 0.007 | 13.00 | 0.75 |
| Motivation for using AI (Entertainment) | 63.57% | [20.54%, 106.61%] | 0.004 | 9.00 | 0.74 |
| Motivation for using AI (Escape) | 44.2% | [7.74%, 80.67%] | 0.017 | 0.00 | 0.72 |
| Motivation for using AI (Social) | 64.73% | [31.17%, 98.28%] | 0.001 | 6.50 | 0.92 |
| Motivation for using AI (Instrumental) | 42.39% | [17.19%, 67.58%] | <0.001 | 2.50 | 1.3 |
| Dependence on AI | 8.52% | [-5.64%, 22.69%] | 0.44 | 20.00 | 0.25 |
| Dependence on AI (Over-reliance) | 19.57% | [-6.3%, 45.43%] | 0.366 | 12.00 | 0.29 |
| Dependence on AI (Excessive Usage) | 10.87% | [-8.64%, 30.38%] | 0.705 | 12.00 | 0.12 |
| Dependence on AI (Jeopardization) | 0.0% | [0.0%, 0.0%] | nan | NaN | nan |
| Dependence on AI (Withdrawal) | 13.04% | [-9.74%, 35.83%] | 0.48 | 5.00 | 0.22 |
| Dependence on AI (Loss of Control) | 6.52% | [-7.0%, 20.05%] | 0.564 | 2.00 | 0.18 |
| Interpersonal Orientation | 8.26% | [4.69%, 11.82%] | <0.001 | 4.35 | 0.34 |
| AI Helpfulness | 10.87% | [1.95%, 19.79%] | 0.029 | 21.00 | 0.55 |
| Perceived Human-Like Behavior | 44.57% | [5.41%, 83.72%] | 0.013 | 2.72 | 0.74 |
| Recommendation to use AI | 24.49% | [11.66%, 37.33%] | 0.002 | 5.50 | 0.83 |
| Attitude towards AI | 9.07% | [2.51%, 15.64%] | 0.003 | 3.37 | 0.48 |
| Attitude towards AI (Positive) | 9.54% | [3.51%, 15.58%] | 0.001 | 3.77 | 0.52 |
| Attitude towards AI (Negative) | 8.48% | [-0.02%, 16.97%] | 0.02 | 2.50 | 0.37 |

Table 6: ChatGPT Relative Change

| Perception Variable | DiD (Active - Baseline) | CI | p-value |
|---|---|---|---|
| Attachment towards AI | 32.99% | [2.32%, 63.66%] | 0.035 |
| Perceived AI empathy | 25.8% | [10.82%, 40.78%] | $<0.001$ |
| Satisfaction with AI | 11.25% | [0.19%, 22.32%] | 0.046 |
| Motivation for using AI (Entertainment) | 22.9% | [2.88%, 42.92%] | 0.025 |
| Motivation for using AI (Escape) | 14.89% | [-4.95%, 34.73%] | 0.141 |
| Motivation for using AI (Social) | 17.91% | [-3.24%, 39.06%] | 0.097 |
| Motivation for using AI (Instrumental) | 12.23% | [-0.45%, 24.91%] | 0.059 |
| Dependence on AI | -0.72% | [-11.69%, 10.25%] | 0.897 |
| Dependence on AI (Over-reliance) | 4.98% | [-11.69%, 21.65%] | 0.557 |
| Dependence on AI (Excessive Usage) | -1.11% | [-16.15%, 13.94%] | 0.885 |
| Dependence on AI (Jeopardization) | -0.23% | [-10.83%, 10.36%] | 0.965 |
| Dependence on AI (Withdrawal) | 2.24% | [-16.39%, 20.87%] | 0.813 |
| Dependence on AI (Loss of Control) | -9.34% | [-23.11%, 4.42%] | 0.183 |
| Interpersonal Orientation | 3.16% | [-0.89%, 7.2%] | 0.126 |
| AI Helpfulness | 7.74% | [-2.72%, 18.2%] | 0.146 |
| Perceived Human-Like Behavior | 14.68% | [-5.98%, 35.34%] | 0.163 |
| Recommendation to use AI | -3.25% | [-21.15%, 14.66%] | 0.721 |
| Attitude towards AI | 1.84% | [-1.91%, 5.58%] | 0.335 |
| Attitude towards AI (Positive) | 3.21% | [-0.9%, 7.32%] | 0.126 |
| Attitude towards AI (Negative) | -0.93% | [-6.85%, 4.98%] | 0.756 |

Table 7: DiD Active - Baseline

| Perception Variable | DiD (Copilot - Baseline) | CI | p-value |
|---|---|---|---|
| Attachment towards AI | 13.89% | [-22.33%, 50.11%] | 0.45 |
| Perceived AI empathy | 29.25% | [8.18%, 50.31%] | 0.007 |
| Satisfaction with AI | 11.14% | [-4.8%, 27.09%] | 0.17 |
| Motivation for using AI (Entertainment) | 19.72% | [-2.51%, 41.94%] | 0.082 |
| Motivation for using AI (Escape) | 1.12% | [-23.43%, 25.66%] | 0.928 |
| Motivation for using AI (Social) | -1.22% | [-31.19%, 28.74%] | 0.936 |
| Motivation for using AI (Instrumental) | 10.25% | [-4.87%, 25.36%] | 0.182 |
| Dependence on AI | -3.81% | [-21.4%, 13.78%] | 0.67 |
| Dependence on AI (Over-reliance) | -5.57% | [-27.76%, 16.63%] | 0.621 |
| Dependence on AI (Excessive Usage) | -11.9% | [-33.8%, 10.01%] | 0.285 |
| Dependence on AI (Jeopardization) | 2.36% | [-16.13%, 20.84%] | 0.802 |
| Dependence on AI (Withdrawal) | 8.53% | [-22.95%, 40.0%] | 0.593 |
| Dependence on AI (Loss of Control) | -9.64% | [-32.66%, 13.39%] | 0.41 |
| Interpersonal Orientation | 2.85% | [-3.86%, 9.56%] | 0.402 |
| AI Helpfulness | 14.07% | [-1.88%, 30.01%] | 0.083 |
| Perceived Human-Like Behavior | 7.5% | [-17.62%, 32.61%] | 0.556 |
| Recommendation to use AI | -10.79% | [-42.81%, 21.23%] | 0.507 |
| Attitude towards AI | -1.12% | [-6.3%, 4.06%] | 0.671 |
| Attitude towards AI (Positive) | 0.21% | [-5.8%, 6.21%] | 0.945 |
| Attitude towards AI (Negative) | -3.43% | [-12.95%, 6.09%] | 0.478 |

Table 8: DiD Copilot - Baseline

| Perception Variable | DiD (Gemini - Baseline) | CI | p-value |
|---|---|---|---|
| Attachment towards AI | 44.44% | [7.48%, 81.41%] | 0.019 |
| Perceived AI empathy | 10.43% | [-4.78%, 25.64%] | 0.177 |
| Satisfaction with AI | 17.2% | [2.68%, 31.72%] | 0.021 |
| Motivation for using AI (Entertainment) | 22.19% | [-4.0%, 48.38%] | 0.096 |
| Motivation for using AI (Escape) | 14.62% | [-12.8%, 42.04%] | 0.294 |
| Motivation for using AI (Social) | 28.54% | [-4.51%, 61.58%] | 0.09 |
| Motivation for using AI (Instrumental) | 6.98% | [-8.04%, 22.0%] | 0.36 |
| Dependence on AI | -3.06% | [-21.23%, 15.11%] | 0.74 |
| Dependence on AI (Over-reliance) | -6.31% | [-27.72%, 15.1%] | 0.561 |
| Dependence on AI (Excessive Usage) | -4.96% | [-28.13%, 18.21%] | 0.673 |
| Dependence on AI (Jeopardization) | 0.6% | [-18.59%, 19.78%] | 0.951 |
| Dependence on AI (Withdrawal) | -1.83% | [-30.87%, 27.22%] | 0.901 |
| Dependence on AI (Loss of Control) | -8.81% | [-33.56%, 15.94%] | 0.483 |
| Interpersonal Orientation | 2.64% | [-3.76%, 9.04%] | 0.417 |
| AI Helpfulness | 11.33% | [-3.14%, 25.79%] | 0.124 |
| Perceived Human-Like Behavior | -2.89% | [-23.91%, 18.13%] | 0.786 |
| Recommendation to use AI | 7.16% | [-25.55%, 39.87%] | 0.666 |
| Attitude towards AI | -2.17% | [-7.12%, 2.78%] | 0.388 |
| Attitude towards AI (Positive) | 0.5% | [-5.32%, 6.32%] | 0.865 |
| Attitude towards AI (Negative) | -6.76% | [-16.3%, 2.78%] | 0.163 |

Table 9: DiD Gemini - Baseline

| Perception Variable | DiD (PI - Baseline) | CI | p-value |
|---|---|---|---|
| Attachment towards AI | -8.08% | [-35.99%, 19.83%] | 0.568 |
| Perceived AI empathy | 13.65% | [-1.54%, 28.83%] | 0.078 |
| Satisfaction with AI | 8.09% | [-7.18%, 23.35%] | 0.297 |
| Motivation for using AI (Entertainment) | -6.04% | [-25.52%, 13.44%] | 0.541 |
| Motivation for using AI (Escape) | 8.8% | [-19.56%, 37.15%] | 0.541 |
| Motivation for using AI (Social) | 0.07% | [-29.08%, 29.21%] | 0.996 |
| Motivation for using AI (Instrumental) | -6.64% | [-19.12%, 5.84%] | 0.295 |
| Dependence on AI | 5.2% | [-12.47%, 22.87%] | 0.562 |
| Dependence on AI (Over-reliance) | 22.3% | [-3.99%, 48.58%] | 0.096 |
| Dependence on AI (Excessive Usage) | 11.49% | [-13.17%, 36.15%] | 0.359 |
| Dependence on AI (Jeopardization) | 0.38% | [-19.54%, 20.3%] | 0.97 |
| Dependence on AI (Withdrawal) | 5.1% | [-24.08%, 34.28%] | 0.73 |
| Dependence on AI (Loss of Control) | -6.97% | [-30.29%, 16.35%] | 0.556 |
| Interpersonal Orientation | 0.95% | [-5.45%, 7.34%] | 0.77 |
| AI Helpfulness | 1.92% | [-12.34%, 16.19%] | 0.79 |
| Perceived Human-Like Behavior | 16.56% | [-7.62%, 40.73%] | 0.178 |
| Recommendation to use AI | -11.5% | [-43.72%, 20.72%] | 0.482 |
| Attitude towards AI | 1.64% | [-3.59%, 6.87%] | 0.536 |
| Attitude towards AI (Positive) | 1.16% | [-4.99%, 7.31%] | 0.71 |
| Attitude towards AI (Negative) | 1.02% | [-8.42%, 10.46%] | 0.831 |

Table 10: DiD PI AI - Baseline

| Perception Variable | DiD (ChatGPT - Baseline) | CI | p-value |
|---|---|---|---|
| Attachment towards AI | 80.92% | [36.89%, 124.95%] | <0.001 |
| Perceived AI empathy | 48.01% | [27.2%, 68.83%] | <0.001 |
| Satisfaction with AI | 8.97% | [-3.22%, 21.16%] | 0.148 |
| Motivation for using AI (Entertainment) | 54.4% | [23.45%, 85.36%] | <0.001 |
| Motivation for using AI (Escape) | 34.74% | [3.86%, 65.62%] | 0.028 |
| Motivation for using AI (Social) | 44.42% | [11.31%, 77.53%] | 0.009 |
| Motivation for using AI (Instrumental) | 37.06% | [18.84%, 55.28%] | <0.001 |
| Dependence on AI | -1.16% | [-19.1%, 16.78%] | 0.898 |
| Dependence on AI (Over-reliance) | 9.29% | [-15.17%, 33.74%] | 0.454 |
| Dependence on AI (Excessive Usage) | 1.15% | [-21.96%, 24.25%] | 0.922 |
| Dependence on AI (Jeopardization) | -4.17% | [-21.72%, 13.39%] | 0.64 |
| Dependence on AI (Withdrawal) | -3.07% | [-32.59%, 26.46%] | 0.838 |
| Dependence on AI (Loss of Control) | -11.81% | [-34.73%, 11.1%] | 0.31 |
| Interpersonal Orientation | 6.04% | [0.08%, 12.0%] | 0.047 |
| AI Helpfulness | 3.7% | [-8.48%, 15.89%] | 0.549 |
| Perceived Human-Like Behavior | 36.12% | [8.45%, 63.8%] | 0.011 |
| Recommendation to use AI | 2.69% | [-28.27%, 33.64%] | 0.864 |
| Attitude towards AI | 8.64% | [2.77%, 14.5%] | 0.004 |
| Attitude towards AI (Positive) | 10.64% | [4.37%, 16.91%] | 0.001 |
| Attitude towards AI (Negative) | 5.01% | [-4.98%, 15.01%] | 0.323 |

Table 11: DiD ChatGPT - Baseline

## Temporal Analysis Results

| Predictors | Coef | CI | Std. Err. | p-value |
|---|---|---|---|---|
| Intercept | 2.16 | [1.73, 2.59] | 0.22 | 0.0 |
| **Group (reference=Baseline)** | | | | |
| Active | 0.05 | [-0.26, 0.37] | 0.16 | 0.735 |
| Week | 0.01 | [-0.06, 0.08] | 0.04 | 0.787 |
| Week:Active | 0.02 | [-0.07, 0.11] | 0.05 | 0.689 |
| AI Helpfulness at Intake | 0.48 | [0.39, 0.57] | 0.05 | 0.0 |

Table 12: Sensitivity Analysis Results for AI Helpfulness

| Predictors | Coef | CI | Std. Err. | p-value |
|---|---|---|---|---|
| Intercept | 0.96 | [0.66, 1.26] | 0.15 | 0.0 |
| **Group (reference=Baseline)** | | | | |
| Active | 0.31 | [-0.03, 0.66] | 0.18 | 0.078 |
| Week | 0.03 | [-0.06, 0.11] | 0.04 | 0.542 |
| Week:Active | 0.07 | [-0.03, 0.18] | 0.05 | 0.177 |
| Attachment towards AI at Intake | 0.53 | [0.46, 0.61] | 0.04 | 0.0 |

Table 13: Sensitivity Analysis Results for Attachment towards AI

| Predictors | Coef | CI | Std. Err. | p-value |
|---|---|---|---|---|
| Intercept | 0.39 | [0.14, 0.65] | 0.13 | 0.003 |
| **Group (reference=Baseline)** | | | | |
| Active | 0.04 | [-0.22, 0.29] | 0.13 | 0.767 |
| Week | 0.02 | [-0.04, 0.07] | 0.03 | 0.511 |
| Week:Active | -0.0 | [-0.07, 0.07] | 0.04 | 0.966 |
| Attitude towards AI (Negative) at Intake | 0.87 | [0.82, 0.92] | 0.03 | 0.0 |

Table 14: Sensitivity Analysis Results for Attitude towards AI (Negative)

| Predictors | Coef | CI | Std. Err. | p-value |
|---|---|---|---|---|
| Intercept | 0.37 | [0.18, 0.55] | 0.09 | 0.0 |
| **Group (reference=Baseline)** | | | | |
| Active | -0.01 | [-0.14, 0.12] | 0.07 | 0.824 |
| Week | -0.0 | [-0.03, 0.03] | 0.02 | 0.914 |
| Week:Active | 0.02 | [-0.02, 0.06] | 0.02 | 0.292 |
| Attitude towards AI (Positive) at Intake | 0.9 | [0.86, 0.94] | 0.02 | 0.0 |

Table 15: Sensitivity Analysis Results for Attitude towards AI (Positive)

| Predictors | Coef | CI | Std. Err. | p-value |
|---|---|---|---|---|
| Intercept | 0.62 | [0.3, 0.94] | 0.16 | 0.0 |
| **Group (reference=Baseline)** | | | | |
| Active | 0.07 | [-0.15, 0.29] | 0.11 | 0.54 |
| Week | 0.02 | [-0.03, 0.08] | 0.03 | 0.376 |
| Week:Active | 0.01 | [-0.06, 0.07] | 0.03 | 0.834 |
| Attitude towards AI at Intake | 0.9 | [0.86, 0.94] | 0.02 | 0.0 |

Table 16: Sensitivity Analysis Results for Attitude towards AI

| Predictors | Coef | CI | Std. Err. | p-value |
|---|---|---|---|---|
| Intercept | 2.66 | [1.94, 3.39] | 0.37 | 0.0 |
| **Group (reference=Baseline)** | | | | |
| Active | -0.37 | [-1.09, 0.34] | 0.37 | 0.307 |
| Week | -0.03 | [-0.19, 0.14] | 0.09 | 0.755 |
| Week:Active | 0.09 | [-0.13, 0.3] | 0.11 | 0.435 |
| Dependence on AI at Intake | 0.64 | [0.57, 0.72] | 0.04 | 0.0 |

Table 17: Sensitivity Analysis Results for Dependence on AI

| Predictors | Coef | CI | Std. Err. | p-value |
|---|---|---|---|---|
| Intercept | 0.68 | [0.51, 0.86] | 0.09 | 0.0 |
| **Group (reference=Baseline)** | | | | |
| Active | -0.03 | [-0.23, 0.17] | 0.1 | 0.752 |
| Week | -0.02 | [-0.06, 0.03] | 0.02 | 0.44 |
| Week:Active | 0.02 | [-0.04, 0.08] | 0.03 | 0.575 |
| Dependence on AI (Excessive Usage) at Intake | 0.55 | [0.48, 0.62] | 0.03 | 0.0 |

Table 18: Sensitivity Analysis Results for Dependence on AI (Excessive Usage)

## Linear Mixed Effects Model Results

### Baseline and active usage groups

| Predictors | Coef | CI | Std. Err. | p-value |
|---|---|---|---|---|
| Intercept | 0.52 | [0.36, 0.67] | 0.08 | 0.0 |
| **Group (reference=Baseline)** | | | | |
| Active | 0.01 | [-0.12, 0.13] | 0.06 | 0.932 |
| Week | 0.01 | [-0.02, 0.04] | 0.01 | 0.652 |
| Week:Active | 0.0 | [-0.04, 0.04] | 0.02 | 0.95 |
| Dependence on AI (Jeopardization) at Intake | 0.53 | [0.41, 0.64] | 0.06 | 0.0 |

Table 19: Sensitivity Analysis Results for Dependence on AI (Jeopardization)

| Predictors | Coef | CI | Std. Err. | p-value |
|---|---|---|---|---|
| Intercept | 0.81 | [0.63, 1.0] | 0.09 | 0.0 |
| **Group (reference=Baseline)** | | | | |
| Active | -0.18 | [-0.39, 0.03] | 0.11 | 0.087 |
| Week | -0.03 | [-0.07, 0.02] | 0.02 | 0.278 |
| Week:Active | 0.04 | [-0.02, 0.11] | 0.03 | 0.161 |
| Dependence on AI (Over-reliance) at Intake | 0.52 | [0.45, 0.59] | 0.04 | 0.0 |

Table 20: Sensitivity Analysis Results for Dependence on AI (Over-reliance)

| Predictors | Coef | CI | Std. Err. | p-value |
|---|---|---|---|---|
| Intercept | 0.68 | [0.5, 0.86] | 0.09 | 0.0 |
| **Group (reference=Baseline)** | | | | |
| Active | -0.11 | [-0.31, 0.09] | 0.1 | 0.277 |
| Week | -0.01 | [-0.05, 0.04] | 0.02 | 0.724 |
| Week:Active | 0.03 | [-0.03, 0.09] | 0.03 | 0.369 |
| Dependence on AI (Withdrawal) at Intake | 0.55 | [0.47, 0.64] | 0.04 | 0.0 |

Table 21: Sensitivity Analysis Results for Dependence on AI (Withdrawal)

| Predictors | Coef | CI | Std. Err. | p-value |
|---|---|---|---|---|
| Intercept | 0.48 | [0.3, 0.65] | 0.09 | 0.0 |
| **Group (reference=Baseline)** | | | | |
| Active | -0.05 | [-0.22, 0.12] | 0.09 | 0.588 |
| Week | 0.02 | [-0.02, 0.06] | 0.02 | 0.318 |
| Week:Active | -0.0 | [-0.06, 0.05] | 0.03 | 0.869 |
| Dependence on AI (Loss of Control) at Intake | 0.64 | [0.54, 0.74] | 0.05 | 0.0 |

Table 22: Sensitivity Analysis Results for Dependence on AI (Loss of Control)

| Predictors | Coef | CI | Std. Err. | p-value |
|---|---|---|---|---|
| Intercept | 1.91 | [-0.37, 4.19] | 1.16 | 0.1 |
| **Group (reference=Baseline)** | | | | |
| Active | 1.52 | [-0.26, 3.29] | 0.91 | 0.094 |
| Week | 0.16 | [-0.25, 0.57] | 0.21 | 0.449 |
| Week:Active | -0.04 | [-0.57, 0.5] | 0.27 | 0.894 |
| Interpersonal Orientation at Intake | 0.96 | [0.92, 1.0] | 0.02 | 0.0 |

Table 23: Sensitivity Analysis Results for Interpersonal Orientation

| Predictors | Coef | CI | Std. Err. | p-value |
|---|---|---|---|---|
| Intercept | 2.41 | [1.78, 3.04] | 0.32 | 0.0 |
| **Group (reference=Baseline)** | | | | |
| Active | 0.34 | [-0.35, 1.02] | 0.35 | 0.332 |
| Week | -0.02 | [-0.18, 0.13] | 0.08 | 0.758 |
| Week:Active | 0.15 | [-0.06, 0.35] | 0.11 | 0.158 |
| Motivation for using AI (Entertainment) at Intake | 0.66 | [0.61, 0.72] | 0.03 | 0.0 |

Table 24: Sensitivity Analysis Results for Motivation for using AI (Entertainment)

| Predictors | Coef | CI | Std. Err. | p-value |
|---|---|---|---|---|
| Intercept | 1.6 | [0.99, 2.21] | 0.31 | 0.0 |
| **Group (reference=Baseline)** | | | | |
| Active | 0.13 | [-0.56, 0.82] | 0.35 | 0.717 |
| Week | 0.01 | [-0.15, 0.17] | 0.08 | 0.919 |
| Week:Active | 0.11 | [-0.1, 0.32] | 0.11 | 0.296 |
| Motivation for using AI (Escape) at Intake | 0.64 | [0.58, 0.7] | 0.03 | 0.0 |

Table 25: Sensitivity Analysis Results for Motivation for using AI (Escape)

| Predictors | Coef | CI | Std. Err. | p-value |
|---|---|---|---|---|
| Intercept | 5.08 | [4.41, 5.76] | 0.35 | 0.0 |
| **Group (reference=Baseline)** | | | | |
| Active | 0.3 | [-0.24, 0.84] | 0.28 | 0.275 |
| Week | 0.06 | [-0.07, 0.18] | 0.06 | 0.377 |
| Week:Active | 0.06 | [-0.1, 0.22] | 0.08 | 0.468 |
| Motivation for using AI (Instrumental) at Intake | 0.48 | [0.43, 0.53] | 0.03 | 0.0 |

Table 26: Sensitivity Analysis Results for Motivation for using AI (Instrumental)

| Predictors | Coef | CI | Std. Err. | p-value |
|---|---|---|---|---|
| Intercept | 1.36 | [0.77, 1.95] | 0.3 | 0.0 |
| **Group (reference=Baseline)** | | | | |
| Active | 0.12 | [-0.55, 0.79] | 0.34 | 0.716 |
| Week | 0.03 | [-0.12, 0.19] | 0.08 | 0.691 |
| Week:Active | 0.11 | [-0.09, 0.32] | 0.1 | 0.272 |
| Motivation for using AI (Social) at Intake | 0.78 | [0.71, 0.84] | 0.03 | 0.0 |

Table 27: Sensitivity Analysis Results for Motivation for using AI (Social)

| Predictors | Coef | CI | Std. Err. | p-value |
|---|---|---|---|---|
| Intercept | 0.81 | [0.53, 1.1] | 0.15 | 0.0 |
| **Group (reference=Baseline)** | | | | |
| Active | 0.52 | [0.25, 0.78] | 0.13 | 0.0 |
| Week | 0.03 | [-0.03, 0.09] | 0.03 | 0.339 |
| Week:Active | 0.03 | [-0.05, 0.11] | 0.04 | 0.489 |
| Perceived AI empathy at Intake | 0.73 | [0.66, 0.8] | 0.03 | 0.0 |

Table 28: Sensitivity Analysis Results for Perceived AI empathy

| Predictors | Coef | CI | Std. Err. | p-value |
|---|---|---|---|---|
| Intercept | 1.34 | [0.96, 1.72] | 0.19 | 0.0 |
| **Group (reference=Baseline)** | | | | |
| Active | -0.15 | [-0.52, 0.23] | 0.19 | 0.444 |
| Week | -0.01 | [-0.1, 0.08] | 0.04 | 0.792 |
| Week:Active | 0.08 | [-0.03, 0.19] | 0.06 | 0.161 |
| Perceived Human-Like Behavior at Intake | 0.61 | [0.53, 0.69] | 0.04 | 0.0 |

Table 29: Sensitivity Analysis Results for Perceived Human-Like Behavior

| Predictors | Coef | CI | Std. Err. | p-value |
|---|---|---|---|---|
| Intercept | 1.76 | [1.38, 2.14] | 0.19 | 0.0 |
| **Group (reference=Baseline)** | | | | |
| Active | 0.25 | [-0.09, 0.59] | 0.17 | 0.145 |
| Week | 0.06 | [-0.01, 0.14] | 0.04 | 0.108 |
| Week:Active | -0.02 | [-0.13, 0.08] | 0.05 | 0.654 |
| Recommendation to use AI at Intake | 0.5 | [0.42, 0.58] | 0.04 | 0.0 |

Table 30: Sensitivity Analysis Results for Recommendation to use AI

| Predictors | Coef | CI | Std. Err. | p-value |
|---|---|---|---|---|
| Intercept | 1.27 | [0.86, 1.67] | 0.21 | 0.0 |
| **Group (reference=Baseline)** | | | | |
| Active | 0.58 | [0.27, 0.89] | 0.16 | 0.0 |
| Week | 0.06 | [-0.01, 0.13] | 0.04 | 0.102 |
| Week:Active | -0.07 | [-0.16, 0.03] | 0.05 | 0.16 |
| Satisfaction with AI at Intake | 0.62 | [0.53, 0.71] | 0.05 | 0.0 |

Table 31: Sensitivity Analysis Results for Satisfaction with AI

| Predictors | Coef | CI | Std. Err. | p-value |
|---|---|---|---|---|
| Intercept | 0.45 | [-0.35, 1.24] | 0.41 | 0.27 |
| **Group (reference=Baseline)** | | | | |
| Active | -0.05 | [-1.06, 0.96] | 0.51 | 0.919 |
| **Gender Identity (reference=Male)** | | | | |
| Female | -0.16 | [-1.27, 0.95] | 0.57 | 0.78 |
| Gender (Female):Active | 0.1 | [-1.33, 1.54] | 0.73 | 0.887 |

Table 32: Linear Mixed Effect Model with 2 groups for Dependence on AI and Gender Identity

| Predictors | Coef | CI | Std. Err. | p-value |
|---|---|---|---|---|
| Intercept | 0.1 | [-0.14, 0.34] | 0.12 | 0.401 |
| **Group (reference=Baseline)** | | | | |
| Active | -0.06 | [-0.37, 0.24] | 0.16 | 0.692 |
| **Gender Identity (reference=Male)** | | | | |
| Female | -0.1 | [-0.44, 0.23] | 0.17 | 0.546 |
| Gender (Female):Active | 0.21 | [-0.23, 0.64] | 0.22 | 0.348 |

Table 33: Linear Mixed Effect Model with 2 groups for Dependence on AI (Over-reliance) and Gender Identity

| Predictors | Coef | CI | Std. Err. | p-value |
|---|---|---|---|---|
| Intercept | 0.03 | [-0.2, 0.27] | 0.12 | 0.776 |
| **Group (reference=Baseline)** | | | | |
| Active | 0.03 | [-0.27, 0.33] | 0.15 | 0.855 |
| **Gender Identity (reference=Male)** | | | | |
| Female | -0.03 | [-0.36, 0.3] | 0.17 | 0.838 |
| Gender (Female):Active | -0.08 | [-0.5, 0.35] | 0.22 | 0.725 |

Table 34: Linear Mixed Effect Model with 2 groups for Dependence on AI (Excessive Usage) and Gender Identity

| Predictors | Coef | CI | Std. Err. | p-value |
|---|---|---|---|---|
| Intercept | -0.0 | [-0.13, 0.13] | 0.07 | 1.0 |
| **Group (reference=Baseline)** | | | | |
| Active | 0.06 | [-0.11, 0.23] | 0.09 | 0.472 |
| **Gender Identity (reference=Male)** | | | | |
| Female | 0.03 | [-0.15, 0.22] | 0.1 | 0.735 |
| Gender (Female):Active | -0.09 | [-0.34, 0.15] | 0.12 | 0.443 |

Table 35: Linear Mixed Effect Model with 2 groups for Dependence on AI (Jeopardization) and Gender Identity

| Predictors | Coef | CI | Std. Err. | p-value |
|---|---|---|---|---|
| Intercept | 0.14 | [-0.1, 0.38] | 0.12 | 0.262 |
| **Group (reference=Baseline)** | | | | |
| Active | -0.03 | [-0.34, 0.27] | 0.16 | 0.828 |
| **Gender Identity (reference=Male)** | | | | |
| Female | -0.04 | [-0.38, 0.29] | 0.17 | 0.81 |
| Gender (Female):Active | 0.16 | [-0.28, 0.59] | 0.22 | 0.48 |

Table 36: Linear Mixed Effect Model with 2 groups for Dependence on AI (Withdrawal) and Gender Identity

| Predictors | Coef | CI | Std. Err. | p-value |
|---|---|---|---|---|
| Intercept | 0.17 | [-0.01, 0.36] | 0.09 | 0.064 |
| **Group (reference=Baseline)** | | | | |
| Active | -0.05 | [-0.28, 0.18] | 0.12 | 0.688 |
| **Gender Identity (reference=Male)** | | | | |
| Female | -0.01 | [-0.27, 0.24] | 0.13 | 0.932 |
| Gender (Female):Active | -0.09 | [-0.42, 0.24] | 0.17 | 0.594 |

Table 37: Linear Mixed Effect Model with 2 groups for Dependence on AI (Loss of Control) and Gender Identity

| Predictors | Coef | CI | Std. Err. | p-value |
|---|---|---|---|---|
| Intercept | 0.15 | [-0.12, 0.41] | 0.14 | 0.276 |
| **Group (reference=Baseline)** | | | | |
| Active | -0.05 | [-0.39, 0.29] | 0.17 | 0.774 |
| **Gender Identity (reference=Male)** | | | | |
| Female | -0.25 | [-0.62, 0.12] | 0.19 | 0.186 |
| Gender (Female):Active | 0.36 | [-0.12, 0.84] | 0.24 | 0.141 |

Table 38: Linear Mixed Effect Model with 2 groups for Attitude towards AI and Gender Identity

| Predictors | Coef | CI | Std. Err. | p-value |
|---|---|---|---|---|
| Intercept | 0.09 | [-0.07, 0.25] | 0.08 | 0.251 |
| **Group (reference=Baseline)** | | | | |
| Active | -0.07 | [-0.27, 0.13] | 0.1 | 0.498 |
| **Gender Identity (reference=Male)** | | | | |
| Female | -0.27 | [-0.49, -0.06] | 0.11 | 0.014 |
| Gender (Female):Active | 0.38 | [0.1, 0.67] | 0.14 | 0.008 |

Table 39: Linear Mixed Effect Model with 2 groups for Attitude towards AI (Positive) and Gender Identity

| Predictors | Coef | CI | Std. Err. | p-value |
|---|---|---|---|---|
| Intercept | 0.06 | [-0.13, 0.24] | 0.09 | 0.555 |
| **Group (reference=Baseline)** | | | | |
| Active | 0.02 | [-0.22, 0.25] | 0.12 | 0.871 |
| **Gender Identity (reference=Male)** | | | | |
| Female | 0.02 | [-0.23, 0.28] | 0.13 | 0.852 |
| Gender (Female):Active | -0.02 | [-0.36, 0.31] | 0.17 | 0.889 |

Table 40: Linear Mixed Effect Model with 2 groups for Attitude towards AI (Negative) and Gender Identity

| Predictors | Coef | CI | Std. Err. | p-value |
|---|---|---|---|---|
| Intercept | 1.62 | [-0.35, 3.59] | 1.0 | 0.106 |
| **Group (reference=Baseline)** | | | | |
| Active | 0.9 | [-1.59, 3.39] | 1.27 | 0.479 |
| **Gender Identity (reference=Male)** | | | | |
| Female | -1.56 | [-4.29, 1.18] | 1.4 | 0.265 |
| Gender (Female):Active | 1.3 | [-2.24, 4.85] | 1.81 | 0.471 |

Table 41: Linear Mixed Effect Model with 2 groups for Interpersonal Orientation and Gender Identity

| Predictors | Coef | CI | Std. Err. | p-value |
|---|---|---|---|---|
| Intercept | 0.52 | [-0.4, 1.43] | 0.47 | 0.267 |
| **Group (reference=Baseline)** | | | | |
| Active | -0.23 | [-1.38, 0.93] | 0.59 | 0.702 |
| **Gender Identity (reference=Male)** | | | | |
| Female | -0.78 | [-2.05, 0.49] | 0.65 | 0.231 |
| Gender (Female):Active | 1.46 | [-0.19, 3.1] | 0.84 | 0.082 |

Table 42: Linear Mixed Effect Model with 2 groups for Motivation for using AI (Escape) and Gender Identity

| Predictors | Coef | CI | Std. Err. | p-value |
|---|---|---|---|---|
| Intercept | 1.1 | [0.29, 1.92] | 0.41 | 0.008 |
| **Group (reference=Baseline)** | | | | |
| Active | 0.13 | [-0.9, 1.15] | 0.52 | 0.811 |
| **Gender Identity (reference=Male)** | | | | |
| Female | -0.94 | [-2.07, 0.19] | 0.58 | 0.102 |
| Gender (Female):Active | 0.91 | [-0.56, 2.37] | 0.75 | 0.224 |

Table 43: Linear Mixed Effect Model with 2 groups for Motivation for using AI (Social) and Gender Identity

| Predictors | Coef | CI | Std. Err. | p-value |
|---|---|---|---|---|
| Intercept | 0.38 | [-0.34, 1.1] | 0.37 | 0.301 |
| **Group (reference=Baseline)** | | | | |
| Active | 0.5 | [-0.41, 1.41] | 0.46 | 0.286 |
| **Gender Identity (reference=Male)** | | | | |
| Female | -0.22 | [-1.22, 0.78] | 0.51 | 0.669 |
| Gender (Female):Active | 0.42 | [-0.88, 1.71] | 0.66 | 0.529 |

Table 44: Linear Mixed Effect Model with 2 groups for Motivation for using AI (Instrumental) and Gender Identity

| Predictors | Coef | CI | Std. Err. | p-value |
|---|---|---|---|---|
| Intercept | 0.38 | [-0.44, 1.2] | 0.42 | 0.366 |
| **Group (reference=Baseline)** | | | | |
| Active | 0.5 | [-0.55, 1.54] | 0.53 | 0.351 |
| **Gender Identity (reference=Male)** | | | | |
| Female | -0.35 | [-1.49, 0.8] | 0.58 | 0.552 |
| Gender (Female):Active | 0.74 | [-0.74, 2.22] | 0.76 | 0.328 |

Table 45: Linear Mixed Effect Model with 2 groups for Motivation for using AI (Entertainment) and Gender Identity

| Predictors | Coef | CI | Std. Err. | p-value |
|---|---|---|---|---|
| Intercept | 0.34 | [-0.12, 0.81] | 0.24 | 0.147 |
| **Group (reference=Baseline)** | | | | |
| Active | 0.32 | [-0.27, 0.91] | 0.3 | 0.285 |
| **Gender Identity (reference=Male)** | | | | |
| Female | -0.28 | [-0.93, 0.37] | 0.33 | 0.397 |
| Gender (Female):Active | 0.49 | [-0.35, 1.33] | 0.43 | 0.251 |

Table 46: Linear Mixed Effect Model with 2 groups for Attachment towards AI and Gender Identity

| Predictors | Coef | CI | Std. Err. | p-value |
|---|---|---|---|---|
| Intercept | 0.76 | [0.34, 1.17] | 0.21 | 0.0 |
| **Group (reference=Baseline)** | | | | |
| Active | -0.2 | [-0.72, 0.33] | 0.27 | 0.465 |
| **Gender Identity (reference=Male)** | | | | |
| Female | -0.76 | [-1.34, -0.18] | 0.3 | 0.01 |
| Gender (Female):Active | 0.61 | [-0.14, 1.36] | 0.38 | 0.11 |

Table 47: Linear Mixed Effect Model with 2 groups for Recommendation to use AI and Gender Identity

| Predictors | Coef | CI | Std. Err. | p-value |
|---|---|---|---|---|
| Intercept | 0.17 | [-0.2, 0.54] | 0.19 | 0.358 |
| **Group (reference=Baseline)** | | | | |
| Active | 0.27 | [-0.2, 0.73] | 0.24 | 0.264 |
| **Gender Identity (reference=Male)** | | | | |
| Female | -0.01 | [-0.52, 0.5] | 0.26 | 0.966 |
| Gender (Female):Active | 0.18 | [-0.48, 0.85] | 0.34 | 0.587 |

Table 48: Linear Mixed Effect Model with 2 groups for Satisfaction with AI and Gender Identity

| Predictors | Coef | CI | Std. Err. | p-value |
|---|---|---|---|---|
| Intercept | 0.14 | [-0.22, 0.5] | 0.18 | 0.451 |
| **Group (reference=Baseline)** | | | | |
| Active | 0.22 | [-0.24, 0.67] | 0.23 | 0.35 |
| **Gender Identity (reference=Male)** | | | | |
| Female | 0.12 | [-0.38, 0.62] | 0.25 | 0.637 |
| Gender (Female):Active | 0.06 | [-0.58, 0.71] | 0.33 | 0.85 |

Table 49: Linear Mixed Effect Model with 2 groups for AI Helpfulness and Gender Identity

| Predictors | Coef | CI | Std. Err. | p-value |
|---|---|---|---|---|
| Intercept | 0.07 | [-0.38, 0.51] | 0.23 | 0.762 |
| **Group (reference=Baseline)** | | | | |
| Active | 0.1 | [-0.47, 0.66] | 0.29 | 0.735 |
| **Gender Identity (reference=Male)** | | | | |
| Female | 0.06 | [-0.56, 0.68] | 0.32 | 0.85 |
| Gender (Female):Active | 0.38 | [-0.42, 1.19] | 0.41 | 0.35 |

Table 50: Linear Mixed Effect Model with 2 groups for Perceived Human-Like Behavior and Gender Identity

| Predictors | Coef | CI | Std. Err. | p-value |
|---|---|---|---|---|
| Intercept | 0.18 | [-0.12, 0.48] | 0.15 | 0.246 |
| **Group (reference=Baseline)** | | | | |
| Active | 0.41 | [0.03, 0.79] | 0.19 | 0.033 |
| **Gender Identity (reference=Male)** | | | | |
| Female | -0.08 | [-0.49, 0.34] | 0.21 | 0.72 |
| Gender (Female):Active | 0.58 | [0.04, 1.12] | 0.27 | 0.035 |

Table 51: Linear Mixed Effect Model with 2 groups for Perceived AI empathy and Gender Identity

| Predictors | Coef | CI | Std. Err. | p-value |
|---|---|---|---|---|
| Intercept | 0.29 | [-0.48, 1.06] | 0.39 | 0.459 |
| **Group (reference=Baseline)** | | | | |
| Active | 0.29 | [-0.75, 1.32] | 0.53 | 0.585 |
| **Mental Health Status (reference=No)** | | | | |
| Yes | 0.16 | [-0.95, 1.26] | 0.56 | 0.779 |
| Mental Health Status (Yes):Active | -0.52 | [-1.96, 0.92] | 0.73 | 0.477 |

Table 52: Linear Mixed Effect Model with 2 groups for Dependence on AI and Mental Health Status

| Predictors | Coef | CI | Std. Err. | p-value |
|---|---|---|---|---|
| Intercept | 0.06 | [-0.17, 0.3] | 0.12 | 0.587 |
| **Group (reference=Baseline)** | | | | |
| Active | 0.12 | [-0.19, 0.43] | 0.16 | 0.455 |
| **Mental Health Status (reference=No)** | | | | |
| Yes | -0.03 | [-0.37, 0.31] | 0.17 | 0.861 |
| Mental Health Status (Yes):Active | -0.13 | [-0.57, 0.3] | 0.22 | 0.545 |

Table 53: Linear Mixed Effect Model with 2 groups for Dependence on AI (Over-reliance) and Mental Health Status

| Predictors | Coef | CI | Std. Err. | p-value |
|---|---|---|---|---|
| Intercept | 0.03 | [-0.2, 0.26] | 0.12 | 0.783 |
| **Group (reference=Baseline)** | | | | |
| Active | 0.02 | [-0.29, 0.33] | 0.16 | 0.897 |
| **Mental Health Status (reference=No)** | | | | |
| Yes | -0.03 | [-0.36, 0.3] | 0.17 | 0.848 |
| Mental Health Status (Yes):Active | -0.04 | [-0.47, 0.39] | 0.22 | 0.855 |

Table 54: Linear Mixed Effect Model with 2 groups for Dependence on AI (Excessive Usage) and Mental Health Status

| Predictors | Coef | CI | Std. Err. | p-value |
|---|---|---|---|---|
| Intercept | -0.06 | [-0.19, 0.06] | 0.07 | 0.327 |
| **Group (reference=Baseline)** | | | | |
| Active | 0.09 | [-0.08, 0.26] | 0.09 | 0.306 |
| **Mental Health Status (reference=No)** | | | | |
| Yes | 0.17 | [-0.02, 0.35] | 0.09 | 0.076 |
| Mental Health Status (Yes):Active | -0.16 | [-0.4, 0.09] | 0.12 | 0.207 |

Table 55: Linear Mixed Effect Model with 2 groups for Dependence on AI (Jeopardization) and Mental Health Status

| Predictors | Coef | CI | Std. Err. | p-value |
|---|---|---|---|---|
| Intercept | 0.1 | [-0.14, 0.33] | 0.12 | 0.416 |
| **Group (reference=Baseline)** | | | | |
| Active | 0.14 | [-0.17, 0.45] | 0.16 | 0.382 |
| **Mental Health Status (reference=No)** | | | | |
| Yes | 0.04 | [-0.29, 0.38] | 0.17 | 0.81 |
| Mental Health Status (Yes):Active | -0.18 | [-0.62, 0.26] | 0.22 | 0.418 |

Table 56: Linear Mixed Effect Model with 2 groups for Dependence on AI (Withdrawal) and Mental Health Status

| Predictors | Coef | CI | Std. Err. | p-value |
|---|---|---|---|---|
| Intercept | 0.16 | [-0.02, 0.34] | 0.09 | 0.075 |
| **Group (reference=Baseline)** | | | | |
| Active | -0.08 | [-0.32, 0.16] | 0.12 | 0.499 |
| **Mental Health Status (reference=No)** | | | | |
| Yes | 0.01 | [-0.24, 0.27] | 0.13 | 0.932 |
| Mental Health Status (Yes):Active | -0.01 | [-0.34, 0.32] | 0.17 | 0.945 |

Table 57: Linear Mixed Effect Model with 2 groups for Dependence on AI (Loss of Control) and Mental Health Status

| Predictors | Coef | CI | Std. Err. | p-value |
|---|---|---|---|---|
| Intercept | -0.03 | [-0.28, 0.23] | 0.13 | 0.84 |
| **Group (reference=Baseline)** | | | | |
| Active | 0.33 | [-0.02, 0.67] | 0.18 | 0.065 |
| **Mental Health Status (reference=No)** | | | | |
| Yes | 0.09 | [-0.28, 0.46] | 0.19 | 0.62 |
| Mental Health Status (Yes):Active | -0.35 | [-0.84, 0.13] | 0.24 | 0.147 |

Table 58: Linear Mixed Effect Model with 2 groups for Attitude towards AI and Mental Health Status

| Predictors | Coef | CI | Std. Err. | p-value |
|---|---|---|---|---|
| Intercept | -0.05 | [-0.2, 0.11] | 0.08 | 0.554 |
| **Group (reference=Baseline)** | | | | |
| Active | 0.2 | [-0.0, 0.41] | 0.11 | 0.054 |
| **Mental Health Status (reference=No)** | | | | |
| Yes | -0.01 | [-0.23, 0.22] | 0.11 | 0.95 |
| Mental Health Status (Yes):Active | -0.14 | [-0.43, 0.15] | 0.15 | 0.342 |

Table 59: Linear Mixed Effect Model with 2 groups for Attitude towards AI (Positive) and Mental Health Status

| Predictors | Coef | CI | Std. Err. | p-value |
|---|---|---|---|---|
| Intercept | 0.02 | [-0.16, 0.2] | 0.09 | 0.825 |
| **Group (reference=Baseline)** | | | | |
| Active | 0.12 | [-0.12, 0.36] | 0.12 | 0.324 |
| **Mental Health Status (reference=No)** | | | | |
| Yes | 0.1 | [-0.16, 0.36] | 0.13 | 0.443 |
| Mental Health Status (Yes):Active | -0.22 | [-0.55, 0.12] | 0.17 | 0.207 |

Table 60: Linear Mixed Effect Model with 2 groups for Attitude towards AI (Negative) and Mental Health Status

| Predictors | Coef | CI | Std. Err. | p-value |
|---|---|---|---|---|
| Intercept | 0.35 | [-1.55, 2.26] | 0.97 | 0.715 |
| **Group (reference=Baseline)** | | | | |
| Active | 1.96 | [-0.61, 4.53] | 1.31 | 0.135 |
| **Mental Health Status (reference=No)** | | | | |
| Yes | 0.96 | [-1.79, 3.7] | 1.4 | 0.495 |
| Mental Health Status (Yes):Active | -0.8 | [-4.37, 2.77] | 1.82 | 0.66 |

Table 61: Linear Mixed Effect Model with 2 groups for Interpersonal Orientation and Mental Health Status

| Predictors | Coef | CI | Std. Err. | p-value |
|---|---|---|---|---|
| Intercept | 0.06 | [-0.83, 0.96] | 0.45 | 0.887 |
| **Group (reference=Baseline)** | | | | |
| Active | 0.38 | [-0.82, 1.58] | 0.61 | 0.532 |
| **Mental Health Status (reference=No)** | | | | |
| Yes | 0.11 | [-1.17, 1.39] | 0.65 | 0.869 |
| Mental Health Status (Yes):Active | 0.17 | [-1.5, 1.84] | 0.85 | 0.841 |

Table 62: Linear Mixed Effect Model with 2 groups for Motivation for using AI (Escape) and Mental Health Status

| Predictors | Coef | CI | Std. Err. | p-value |
|---|---|---|---|---|
| Intercept | 0.55 | [-0.24, 1.34] | 0.4 | 0.173 |
| **Group (reference=Baseline)** | | | | |
| Active | 0.37 | [-0.69, 1.44] | 0.54 | 0.492 |
| **Mental Health Status (reference=No)** | | | | |
| Yes | 0.14 | [-0.99, 1.28] | 0.58 | 0.807 |
| Mental Health Status (Yes):Active | 0.37 | [-1.11, 1.84] | 0.75 | 0.624 |

Table 63: Linear Mixed Effect Model with 2 groups for Motivation for using AI (Social) and Mental Health Status

| Predictors | Coef | CI | Std. Err. | p-value |
|---|---|---|---|---|
| Intercept | 0.65 | [-0.04, 1.33] | 0.35 | 0.065 |
| **Group (reference=Baseline)** | | | | |
| Active | 0.7 | [-0.23, 1.62] | 0.47 | 0.139 |
| **Mental Health Status (reference=No)** | | | | |
| Yes | -0.78 | [-1.77, 0.2] | 0.5 | 0.119 |
| Mental Health Status (Yes):Active | 0.13 | [-1.15, 1.41] | 0.65 | 0.845 |

Table 64: Linear Mixed Effect Model with 2 groups for Motivation for using AI (Instrumental) and Mental Health Status

| Predictors | Coef | CI | Std. Err. | p-value |
|---|---|---|---|---|
| Intercept | 0.61 | [-0.17, 1.4] | 0.4 | 0.126 |
| **Group (reference=Baseline)** | | | | |
| Active | 0.89 | [-0.17, 1.95] | 0.54 | 0.101 |
| **Mental Health Status (reference=No)** | | | | |
| Yes | -0.85 | [-1.98, 0.28] | 0.58 | 0.138 |
| Mental Health Status (Yes):Active | 0.08 | [-1.39, 1.55] | 0.75 | 0.915 |

Table 65: Linear Mixed Effect Model with 2 groups for Motivation for using AI (Entertainment) and Mental Health Status

| Predictors | Coef | CI | Std. Err. | p-value |
|---|---|---|---|---|
| Intercept | 0.19 | [-0.26, 0.65] | 0.23 | 0.401 |
| **Group (reference=Baseline)** | | | | |
| Active | 0.67 | [0.07, 1.28] | 0.31 | 0.03 |
| **Mental Health Status (reference=No)** | | | | |
| Yes | 0.01 | [-0.64, 0.66] | 0.33 | 0.968 |
| Mental Health Status (Yes):Active | -0.2 | [-1.04, 0.65] | 0.43 | 0.65 |

Table 66: Linear Mixed Effect Model with 2 groups for Attachment towards AI and Mental Health Status

| Predictors | Coef | CI | Std. Err. | p-value |
|---|---|---|---|---|
| Intercept | 0.26 | [-0.15, 0.67] | 0.21 | 0.218 |
| **Group (reference=Baseline)** | | | | |
| Active | 0.22 | [-0.34, 0.77] | 0.28 | 0.445 |
| **Mental Health Status (reference=No)** | | | | |
| Yes | 0.22 | [-0.37, 0.82] | 0.3 | 0.456 |
| Mental Health Status (Yes):Active | -0.19 | [-0.96, 0.58] | 0.39 | 0.63 |

Table 67: Linear Mixed Effect Model with 2 groups for Recommendation to use AI and Mental Health Status

| Predictors | Coef | CI | Std. Err. | p-value |
|---|---|---|---|---|
| Intercept | 0.19 | [-0.16, 0.55] | 0.18 | 0.282 |
| **Group (reference=Baseline)** | | | | |
| Active | 0.54 | [0.07, 1.02] | 0.24 | 0.025 |
| **Mental Health Status (reference=No)** | | | | |
| Yes | -0.06 | [-0.56, 0.45] | 0.26 | 0.83 |
| Mental Health Status (Yes):Active | -0.33 | [-0.99, 0.33] | 0.34 | 0.329 |

Table 68: Linear Mixed Effect Model with 2 groups for Satisfaction with AI and Mental Health Status

| Predictors | Coef | CI | Std. Err. | p-value |
|---|---|---|---|---|
| Intercept | 0.13 | [-0.22, 0.48] | 0.18 | 0.466 |
| **Group (reference=Baseline)** | | | | |
| Active | 0.4 | [-0.07, 0.86] | 0.24 | 0.096 |
| **Mental Health Status (reference=No)** | | | | |
| Yes | 0.15 | [-0.35, 0.65] | 0.25 | 0.564 |
| Mental Health Status (Yes):Active | -0.3 | [-0.95, 0.35] | 0.33 | 0.363 |

Table 69: Linear Mixed Effect Model with 2 groups for AI Helpfulness and Mental Health Status

**Baseline and platform sub-groups**

| Predictors | Coef | CI | Std. Err. | p-value |
|---|---|---|---|---|
| Intercept | 0.26 | [-0.18, 0.69] | 0.22 | 0.244 |
| **Group (reference=Baseline)** | | | | |
| Active | 0.08 | [-0.5, 0.67] | 0.3 | 0.778 |
| **Mental Health Status (reference=No)** | | | | |
| Yes | -0.33 | [-0.95, 0.3] | 0.32 | 0.305 |
| Mental Health Status (Yes):Active | 0.38 | [-0.43, 1.19] | 0.41 | 0.362 |

Table 70: Linear Mixed Effect Model with 2 groups for Perceived Human-Like Behavior and Mental Health Status

| Predictors | Coef | CI | Std. Err. | p-value |
|---|---|---|---|---|
| Intercept | 0.16 | [-0.14, 0.45] | 0.15 | 0.297 |
| **Group (reference=Baseline)** | | | | |
| Active | 0.52 | [0.13, 0.92] | 0.2 | 0.01 |
| **Mental Health Status (reference=No)** | | | | |
| Yes | -0.04 | [-0.47, 0.38] | 0.22 | 0.85 |
| Mental Health Status (Yes):Active | 0.28 | [-0.27, 0.84] | 0.28 | 0.313 |

Table 71: Linear Mixed Effect Model with 2 groups for Perceived AI empathy and Mental Health Status

| Predictors | Coef | CI | Std. Err. | p-value |
|---|---|---|---|---|
| Intercept | 0.81 | [0.23, 1.39] | 0.3 | 0.006 |
| **Group (reference=Baseline)** | | | | |
| Active | -0.27 | [-1.18, 0.64] | 0.46 | 0.56 |
| **AI Usage Label (reference=Cold)** | | | | |
| Hot | -1.16 | [-2.24, -0.08] | 0.55 | 0.035 |
| AI Usage (Hot):Active | 0.77 | [-0.67, 2.21] | 0.73 | 0.292 |

Table 72: Linear Mixed Effect Model with 2 groups for Dependence on AI and AI Usage Label

| Predictors | Coef | CI | Std. Err. | p-value |
|---|---|---|---|---|
| Intercept | 0.11 | [0.05, 0.16] | 0.03 | 0.0 |
| **Group (reference=Baseline)** | | | | |
| Active | 0.07 | [-0.14, 0.28] | 0.11 | 0.503 |
| **AI Usage Label (reference=Cold)** | | | | |
| Hot | -0.15 | [-0.42, 0.12] | 0.14 | 0.271 |
| AI Usage (Hot):Active | -0.05 | [-0.47, 0.36] | 0.21 | 0.799 |

Table 73: Linear Mixed Effect Model with 2 groups for Dependence on AI (Over-reliance) and AI Usage Label

| Predictors | Coef | CI | Std. Err. | p-value |
|---|---|---|---|---|
| Intercept | 0.11 | [-0.1, 0.31] | 0.1 | 0.3 |
| **Group (reference=Baseline)** | | | | |
| Active | 0.01 | [-0.26, 0.28] | 0.14 | 0.932 |
| **AI Usage Label (reference=Cold)** | | | | |
| Hot | -0.24 | [-0.5, 0.02] | 0.13 | 0.074 |
| AI Usage (Hot):Active | -0.01 | [-0.31, 0.29] | 0.15 | 0.949 |

Table 74: Linear Mixed Effect Model with 2 groups for Dependence on AI (Excessive Usage) and AI Usage Label

| Predictors | Coef | CI | Std. Err. | p-value |
|---|---|---|---|---|
| Intercept | 0.05 | [-0.0, 0.11] | 0.03 | 0.056 |
| **Group (reference=Baseline)** | | | | |
| Active | -0.05 | [-0.18, 0.08] | 0.07 | 0.413 |
| **AI Usage Label (reference=Cold)** | | | | |
| Hot | -0.1 | [-0.24, 0.04] | 0.07 | 0.174 |
| AI Usage (Hot):Active | 0.17 | [-0.01, 0.36] | 0.1 | 0.067 |

Table 75: Linear Mixed Effect Model with 2 groups for Dependence on AI (Jeopardization) and AI Usage Label

| Predictors | Coef | CI | Std. Err. | p-value |
|---|---|---|---|---|
| Intercept | 0.3 | [0.12, 0.48] | 0.09 | 0.001 |
| **Group (reference=Baseline)** | | | | |
| Active | -0.16 | [-0.38, 0.07] | 0.12 | 0.172 |
| **AI Usage Label (reference=Cold)** | | | | |
| Hot | -0.47 | [-0.61, -0.33] | 0.07 | 0.0 |
| AI Usage (Hot):Active | 0.51 | [0.19, 0.83] | 0.16 | 0.002 |

Table 76: Linear Mixed Effect Model with 2 groups for Dependence on AI (Withdrawal) and AI Usage Label

| Predictors | Coef | CI | Std. Err. | p-value |
|---|---|---|---|---|
| Intercept | 0.24 | [0.23, 0.26] | 0.01 | 0.0 |
| **Group (reference=Baseline)** | | | | |
| Active | -0.14 | [-0.27, -0.02] | 0.06 | 0.023 |
| **AI Usage Label (reference=Cold)** | | | | |
| Hot | -0.2 | [-0.41, 0.01] | 0.11 | 0.066 |
| AI Usage (Hot):Active | 0.15 | [-0.14, 0.45] | 0.15 | 0.314 |

Table 77: Linear Mixed Effect Model with 2 groups for Dependence on AI (Loss of Control) and AI Usage Label

| Predictors | Coef | CI | Std. Err. | p-value |
|---|---|---|---|---|
| Intercept | -0.01 | [-0.08, 0.06] | 0.04 | 0.732 |
| **Group (reference=Baseline)** | | | | |
| Active | 0.16 | [0.04, 0.29] | 0.06 | 0.011 |
| **AI Usage Label (reference=Cold)** | | | | |
| Hot | 0.08 | [-0.22, 0.38] | 0.15 | 0.599 |
| AI Usage (Hot):Active | -0.08 | [-0.47, 0.31] | 0.2 | 0.676 |

Table 78: Linear Mixed Effect Model with 2 groups for Attitude towards AI and AI Usage Label

| Predictors | Coef | CI | Std. Err. | p-value |
|---|---|---|---|---|
| Intercept | -0.06 | [-0.1, -0.02] | 0.02 | 0.001 |
| **Group (reference=Baseline)** | | | | |
| Active | 0.14 | [0.01, 0.28] | 0.07 | 0.042 |
| **AI Usage Label (reference=Cold)** | | | | |
| Hot | 0.03 | [-0.11, 0.17] | 0.07 | 0.632 |
| AI Usage (Hot):Active | -0.04 | [-0.27, 0.19] | 0.12 | 0.711 |

Table 79: Linear Mixed Effect Model with 2 groups for Attitude towards AI (Positive) and AI Usage Label

| Predictors | Coef | CI | Std. Err. | p-value |
|---|---|---|---|---|
| Intercept | 0.05 | [0.0, 0.1] | 0.02 | 0.032 |
| **Group (reference=Baseline)** | | | | |
| Active | 0.02 | [-0.15, 0.2] | 0.09 | 0.806 |
| **AI Usage Label (reference=Cold)** | | | | |
| Hot | 0.05 | [-0.17, 0.27] | 0.11 | 0.672 |
| AI Usage (Hot):Active | -0.04 | [-0.34, 0.26] | 0.16 | 0.799 |

Table 80: Linear Mixed Effect Model with 2 groups for Attitude towards AI (Negative) and AI Usage Label

| Predictors | Coef | CI | Std. Err. | p-value |
|---|---|---|---|---|
| Intercept | 0.97 | [0.14, 1.81] | 0.43 | 0.022 |
| **Group (reference=Baseline)** | | | | |
| Active | 0.93 | [-0.5, 2.35] | 0.73 | 0.201 |
| **AI Usage Label (reference=Cold)** | | | | |
| Hot | -0.41 | [-3.04, 2.22] | 1.34 | 0.761 |
| AI Usage (Hot):Active | 1.56 | [-1.51, 4.63] | 1.57 | 0.32 |

Table 81: Linear Mixed Effect Model with 2 groups for Interpersonal Orientation and AI Usage Label

| Predictors | Coef | CI | Std. Err. | p-value |
|---|---|---|---|---|
| Intercept | 0.49 | [0.14, 0.83] | 0.17 | 0.005 |
| **Group (reference=Baseline)** | | | | |
| Active | 0.63 | [0.32, 0.95] | 0.16 | 0.0 |
| **AI Usage Label (reference=Cold)** | | | | |
| Hot | -0.96 | [-2.07, 0.14] | 0.56 | 0.086 |
| AI Usage (Hot):Active | -0.21 | [-1.61, 1.2] | 0.72 | 0.773 |

Table 82: Linear Mixed Effect Model with 2 groups for Motivation for using AI (Escape) and AI Usage Label

| Predictors | Coef | CI | Std. Err. | p-value |
|---|---|---|---|---|
| Intercept | 0.59 | [0.11, 1.08] | 0.25 | 0.015 |
| **Group (reference=Baseline)** | | | | |
| Active | 0.81 | [0.5, 1.11] | 0.16 | 0.0 |
| **AI Usage Label (reference=Cold)** | | | | |
| Hot | 0.06 | [-0.8, 0.91] | 0.44 | 0.895 |
| AI Usage (Hot):Active | -0.48 | [-1.55, 0.58] | 0.54 | 0.375 |

Table 83: Linear Mixed Effect Model with 2 groups for Motivation for using AI (Social) and AI Usage Label

| Predictors | Coef | CI | Std. Err. | p-value |
|---|---|---|---|---|
| Intercept | 0.59 | [0.12, 1.07] | 0.24 | 0.013 |
| **Group (reference=Baseline)** | | | | |
| Active | 0.85 | [0.57, 1.12] | 0.14 | 0.0 |
| **AI Usage Label (reference=Cold)** | | | | |
| Hot | -0.86 | [-1.84, 0.12] | 0.5 | 0.087 |
| AI Usage (Hot):Active | -0.23 | [-1.33, 0.88] | 0.57 | 0.69 |

Table 84: Linear Mixed Effect Model with 2 groups for Motivation for using AI (Instrumental) and AI Usage Label

| Predictors | Coef | CI | Std. Err. | p-value |
|---|---|---|---|---|
| Intercept | 0.38 | [-0.2, 0.96] | 0.3 | 0.203 |
| **Group (reference=Baseline)** | | | | |
| Active | 0.88 | [-0.08, 1.84] | 0.49 | 0.072 |
| **AI Usage Label (reference=Cold)** | | | | |
| Hot | -0.47 | [-1.37, 0.44] | 0.46 | 0.312 |
| AI Usage (Hot):Active | 0.0 | [-1.47, 1.47] | 0.75 | 1.0 |

Table 85: Linear Mixed Effect Model with 2 groups for Motivation for using AI (Entertainment) and AI Usage Label

| Predictors | Coef | CI | Std. Err. | p-value |
|---|---|---|---|---|
| Intercept | 0.05 | [-0.23, 0.33] | 0.14 | 0.705 |
| **Group (reference=Baseline)** | | | | |
| Active | 0.89 | [0.82, 0.96] | 0.04 | 0.0 |
| **AI Usage Label (reference=Cold)** | | | | |
| Hot | 0.38 | [-0.23, 0.99] | 0.31 | 0.218 |
| AI Usage (Hot):Active | -0.78 | [-1.5, -0.07] | 0.36 | 0.032 |

Table 86: Linear Mixed Effect Model with 2 groups for Attachment towards AI and AI Usage Label

| Predictors | Coef | CI | Std. Err. | p-value |
|---|---|---|---|---|
| Intercept | 0.38 | [0.19, 0.57] | 0.1 | 0.0 |
| **Group (reference=Baseline)** | | | | |
| Active | 0.24 | [0.04, 0.45] | 0.1 | 0.02 |
| **AI Usage Label (reference=Cold)** | | | | |
| Hot | -0.03 | [-0.43, 0.37] | 0.21 | 0.882 |
| AI Usage (Hot):Active | -0.26 | [-0.83, 0.32] | 0.3 | 0.386 |

Table 87: Linear Mixed Effect Model with 2 groups for Recommendation to use AI and AI Usage Label

| Predictors | Coef | CI | Std. Err. | p-value |
|---|---|---|---|---|
| Intercept | 0.16 | [-0.15, 0.47] | 0.16 | 0.304 |
| **Group (reference=Baseline)** | | | | |
| Active | 0.36 | [-0.02, 0.73] | 0.19 | 0.063 |
| **AI Usage Label (reference=Cold)** | | | | |
| Hot | 0.01 | [-0.35, 0.37] | 0.18 | 0.949 |
| AI Usage (Hot):Active | -0.02 | [-0.62, 0.58] | 0.31 | 0.951 |

Table 88: Linear Mixed Effect Model with 2 groups for Satisfaction with AI and AI Usage Label

| Predictors | Coef | CI | Std. Err. | p-value |
|---|---|---|---|---|
| Intercept | 0.16 | [-0.11, 0.43] | 0.14 | 0.237 |
| **Group (reference=Baseline)** | | | | |
| Active | 0.32 | [-0.1, 0.73] | 0.21 | 0.134 |
| **AI Usage Label (reference=Cold)** | | | | |
| Hot | 0.1 | [-0.41, 0.6] | 0.26 | 0.702 |
| AI Usage (Hot):Active | -0.19 | [-0.83, 0.44] | 0.33 | 0.551 |

Table 89: Linear Mixed Effect Model with 2 groups for AI Helpfulness and AI Usage Label

| Predictors | Coef | CI | Std. Err. | p-value |
|---|---|---|---|---|
| Intercept | 0.14 | [-0.21, 0.48] | 0.18 | 0.444 |
| **Group (reference=Baseline)** | | | | |
| Active | 0.52 | [0.26, 0.79] | 0.13 | 0.0 |
| **AI Usage Label (reference=Cold)** | | | | |
| Hot | -0.09 | [-0.72, 0.54] | 0.32 | 0.775 |
| AI Usage (Hot):Active | -0.57 | [-1.34, 0.2] | 0.39 | 0.15 |

Table 90: Linear Mixed Effect Model with 2 groups for Perceived Human-Like Behavior and AI Usage Label

| Predictors | Coef | CI | Std. Err. | p-value |
|---|---|---|---|---|
| Intercept | 0.1 | [-0.13, 0.33] | 0.12 | 0.405 |
| **Group (reference=Baseline)** | | | | |
| Active | 0.75 | [0.63, 0.87] | 0.06 | 0.0 |
| **AI Usage Label (reference=Cold)** | | | | |
| Hot | 0.1 | [-0.33, 0.53] | 0.22 | 0.638 |
| AI Usage (Hot):Active | -0.16 | [-0.63, 0.31] | 0.24 | 0.506 |

Table 91: Linear Mixed Effect Model with 2 groups for Perceived AI empathy and AI Usage Label

| Predictors | Coef | CI | Std. Err. | p-value |
|---|---|---|---|---|
| Intercept | 0.45 | [-0.32, 1.22] | 0.39 | 0.252 |
| **Group (reference=Baseline)** | | | | |
| Copilot | -0.27 | [-1.73, 1.19] | 0.75 | 0.721 |
| Gemini | 0.19 | [-1.2, 1.59] | 0.71 | 0.784 |
| PI | 0.24 | [-1.19, 1.68] | 0.73 | 0.739 |
| ChatGPT | -0.55 | [-1.64, 0.55] | 0.56 | 0.327 |
| **Gender Identity (reference=Male)** | | | | |
| Female | -0.16 | [-1.18, 0.87] | 0.52 | 0.762 |
| Gender (Female):Copilot | 0.14 | [-1.8, 2.09] | 0.99 | 0.886 |
| Gender (Female):Gemini | -1.06 | [-3.34, 1.23] | 1.17 | 0.365 |
| Gender (Female):PI | 0.35 | [-1.83, 2.54] | 1.11 | 0.75 |
| Gender (Female):ChatGPT | 0.87 | [-0.09, 1.84] | 0.49 | 0.075 |

Table 92: Linear Mixed Effect Model with 5 groups for Dependence on AI and Gender Identity

| Predictors | Coef | CI | Std. Err. | p-value |
|---|---|---|---|---|
| Intercept | 0.1 | [0.01, 0.2] | 0.05 | 0.027 |
| **Group (reference=Baseline)** | | | | |
| Copilot | -0.19 | [-0.57, 0.18] | 0.19 | 0.31 |
| Gemini | 0.04 | [-0.33, 0.41] | 0.19 | 0.834 |
| PI | -0.03 | [-0.36, 0.31] | 0.17 | 0.878 |
| ChatGPT | -0.1 | [-0.53, 0.33] | 0.22 | 0.638 |
| **Gender Identity (reference=Male)** | | | | |
| Female | -0.1 | [-0.4, 0.2] | 0.15 | 0.499 |
| Gender (Female):Copilot | 0.19 | [-0.41, 0.8] | 0.31 | 0.529 |
| Gender (Female):Gemini | -0.33 | [-1.0, 0.35] | 0.35 | 0.347 |
| Gender (Female):PI | 0.58 | [-0.04, 1.21] | 0.32 | 0.068 |
| Gender (Female):ChatGPT | 0.33 | [-0.29, 0.96] | 0.32 | 0.297 |

Table 93: Linear Mixed Effect Model with 5 groups for Dependence on AI (Over-reliance) and Gender Identity

| Predictors | Coef | CI | Std. Err. | p-value |
|---|---|---|---|---|
| Intercept | 0.03 | [-0.1, 0.17] | 0.07 | 0.609 |
| **Group (reference=Baseline)** | | | | |
| Copilot | -0.13 | [-0.56, 0.31] | 0.22 | 0.57 |
| Gemini | 0.11 | [-0.23, 0.45] | 0.17 | 0.529 |
| PI | 0.2 | [-0.1, 0.49] | 0.15 | 0.193 |
| ChatGPT | -0.13 | [-0.53, 0.26] | 0.2 | 0.503 |
| **Gender Identity (reference=Male)** | | | | |
| Female | -0.03 | [-0.33, 0.27] | 0.15 | 0.822 |
| Gender (Female):Copilot | -0.04 | [-0.67, 0.59] | 0.32 | 0.898 |
| Gender (Female):Gemini | -0.39 | [-1.04, 0.25] | 0.33 | 0.234 |
| Gender (Female):PI | -0.2 | [-0.8, 0.41] | 0.31 | 0.523 |
| Gender (Female):ChatGPT | 0.29 | [-0.33, 0.9] | 0.31 | 0.359 |

Table 94: Linear Mixed Effect Model with 5 groups for Dependence on AI (Excessive Usage) and Gender Identity

| Predictors | Coef | CI | Std. Err. | p-value |
|---|---|---|---|---|
| Intercept | 0.0 | [-0.1, 0.1] | 0.05 | 1.0 |
| **Group (reference=Baseline)** | | | | |
| Copilot | 0.09 | [-0.16, 0.34] | 0.13 | 0.479 |
| Gemini | 0.07 | [-0.12, 0.27] | 0.1 | 0.47 |
| PI | 0.08 | [-0.1, 0.26] | 0.09 | 0.404 |
| ChatGPT | -0.0 | [-0.26, 0.26] | 0.13 | 1.0 |
| **Gender Identity (reference=Male)** | | | | |
| Female | 0.03 | [-0.08, 0.14] | 0.06 | 0.573 |
| Gender (Female):Copilot | -0.04 | [-0.35, 0.27] | 0.16 | 0.801 |
| Gender (Female):Gemini | -0.1 | [-0.39, 0.18] | 0.15 | 0.48 |
| Gender (Female):PI | -0.22 | [-0.5, 0.06] | 0.14 | 0.122 |
| Gender (Female):ChatGPT | -0.03 | [-0.37, 0.3] | 0.17 | 0.851 |

Table 95: Linear Mixed Effect Model with 5 groups for Dependence on AI (Jeopardization) and Gender Identity

| Predictors | Coef | CI | Std. Err. | p-value |
|---|---|---|---|---|
| Intercept | 0.14 | [-0.02, 0.3] | 0.08 | 0.095 |
| **Group (reference=Baseline)** | | | | |
| Copilot | -0.05 | [-0.42, 0.33] | 0.19 | 0.805 |
| Gemini | 0.0 | [-0.36, 0.37] | 0.19 | 0.979 |
| PI | 0.02 | [-0.3, 0.33] | 0.16 | 0.922 |
| ChatGPT | -0.14 | [-0.48, 0.21] | 0.18 | 0.431 |
| **Gender Identity (reference=Male)** | | | | |
| Female | -0.04 | [-0.3, 0.22] | 0.13 | 0.759 |
| Gender (Female):Copilot | 0.2 | [-0.37, 0.77] | 0.29 | 0.489 |
| Gender (Female):Gemini | 0.04 | [-0.63, 0.71] | 0.34 | 0.904 |
| Gender (Female):PI | 0.22 | [-0.38, 0.82] | 0.31 | 0.47 |
| Gender (Female):ChatGPT | 0.2 | [-0.26, 0.65] | 0.23 | 0.396 |

Table 96: Linear Mixed Effect Model with 5 groups for Dependence on AI (Withdrawal) and Gender Identity

| Predictors | Coef | CI | Std. Err. | p-value |
|---|---|---|---|---|
| Intercept | 0.17 | [0.04, 0.31] | 0.07 | 0.012 |
| **Group (reference=Baseline)** | | | | |
| Copilot | 0.01 | [-0.29, 0.31] | 0.15 | 0.951 |
| Gemini | -0.03 | [-0.32, 0.26] | 0.15 | 0.843 |
| PI | -0.02 | [-0.3, 0.27] | 0.15 | 0.899 |
| ChatGPT | -0.17 | [-0.5, 0.15] | 0.17 | 0.302 |
| **Gender Identity (reference=Male)** | | | | |
| Female | -0.01 | [-0.08, 0.06] | 0.04 | 0.765 |
| Gender (Female):Copilot | -0.17 | [-0.56, 0.21] | 0.2 | 0.385 |
| Gender (Female):Gemini | -0.27 | [-0.75, 0.2] | 0.24 | 0.256 |
| Gender (Female):PI | -0.03 | [-0.44, 0.38] | 0.21 | 0.879 |
| Gender (Female):ChatGPT | 0.09 | [-0.32, 0.5] | 0.21 | 0.672 |

Table 97: Linear Mixed Effect Model with 5 groups for Dependence on AI (Loss of Control) and Gender Identity

| Predictors | Coef | CI | Std. Err. | p-value |
|---|---|---|---|---|
| Intercept | 0.15 | [0.11, 0.19] | 0.02 | 0.0 |
| **Group (reference=Baseline)** | | | | |
| Copilot | -0.2 | [-0.61, 0.2] | 0.21 | 0.323 |
| Gemini | -0.21 | [-0.57, 0.16] | 0.19 | 0.262 |
| PI | 0.05 | [-0.31, 0.42] | 0.19 | 0.782 |
| ChatGPT | 0.21 | [-0.23, 0.65] | 0.23 | 0.347 |
| **Gender Identity (reference=Male)** | | | | |
| Female | -0.25 | [-0.47, -0.03] | 0.11 | 0.023 |
| Gender (Female):Copilot | 0.19 | [-0.42, 0.79] | 0.31 | 0.547 |
| Gender (Female):Gemini | 0.03 | [-0.65, 0.71] | 0.35 | 0.929 |
| Gender (Female):PI | 0.16 | [-0.47, 0.79] | 0.32 | 0.625 |
| Gender (Female):ChatGPT | 0.74 | [0.11, 1.36] | 0.32 | 0.021 |

Table 98: Linear Mixed Effect Model with 5 groups for Attitude towards AI and Gender Identity

| Predictors | Coef | CI | Std. Err. | p-value |
|---|---|---|---|---|
| Intercept | 0.09 | [-0.05, 0.23] | 0.07 | 0.195 |
| **Group (reference=Baseline)** | | | | |
| Copilot | -0.19 | [-0.48, 0.09] | 0.14 | 0.18 |
| Gemini | -0.11 | [-0.37, 0.16] | 0.14 | 0.428 |
| PI | -0.07 | [-0.33, 0.18] | 0.13 | 0.563 |
| ChatGPT | 0.13 | [0.02, 0.24] | 0.06 | 0.022 |
| **Gender Identity (reference=Male)** | | | | |
| Female | -0.27 | [-0.47, -0.07] | 0.1 | 0.007 |
| Gender (Female):Copilot | 0.34 | [-0.06, 0.74] | 0.2 | 0.094 |
| Gender (Female):Gemini | 0.24 | [-0.19, 0.67] | 0.22 | 0.266 |
| Gender (Female):PI | 0.29 | [-0.1, 0.69] | 0.2 | 0.141 |
| Gender (Female):ChatGPT | 0.51 | [0.25, 0.76] | 0.13 | 0.0 |

Table 99: Linear Mixed Effect Model with 5 groups for Attitude towards AI (Positive) and Gender Identity

| Predictors | Coef | CI | Std. Err. | p-value |
|---|---|---|---|---|
| Intercept | 0.06 | [-0.04, 0.16] | 0.05 | 0.268 |
| **Group (reference=Baseline)** | | | | |
| Copilot | -0.01 | [-0.32, 0.29] | 0.16 | 0.946 |
| Gemini | -0.1 | [-0.39, 0.19] | 0.15 | 0.493 |
| PI | 0.13 | [-0.1, 0.36] | 0.12 | 0.278 |
| ChatGPT | 0.08 | [-0.21, 0.37] | 0.15 | 0.579 |
| **Gender Identity (reference=Male)** | | | | |
| Female | 0.02 | [-0.11, 0.15] | 0.07 | 0.711 |
| Gender (Female):Copilot | -0.15 | [-0.58, 0.27] | 0.22 | 0.477 |
| Gender (Female):Gemini | -0.21 | [-0.67, 0.25] | 0.24 | 0.368 |
| Gender (Female):PI | -0.14 | [-0.55, 0.27] | 0.21 | 0.509 |
| Gender (Female):ChatGPT | 0.23 | [-0.18, 0.64] | 0.21 | 0.268 |

Table 100: Linear Mixed Effect Model with 5 groups for Attitude towards AI (Negative) and Gender Identity

| Predictors | Coef | CI | Std. Err. | p-value |
|---|---|---|---|---|
| Intercept | 1.62 | [0.43, 2.81] | 0.61 | 0.008 |
| **Group (reference=Baseline)** | | | | |
| Copilot | -0.89 | [-4.5, 2.71] | 1.84 | 0.627 |
| Gemini | -0.05 | [-2.91, 2.81] | 1.46 | 0.973 |
| PI | 0.46 | [-2.71, 3.63] | 1.62 | 0.778 |
| ChatGPT | 4.78 | [1.18, 8.38] | 1.84 | 0.009 |
| **Gender Identity (reference=Male)** | | | | |
| Female | -1.56 | [-2.99, -0.12] | 0.73 | 0.034 |
| Gender (Female):Copilot | 4.5 | [-0.59, 9.58] | 2.59 | 0.083 |
| Gender (Female):Gemini | 2.41 | [-2.31, 7.13] | 2.41 | 0.316 |
| Gender (Female):PI | 0.48 | [-4.22, 5.18] | 2.4 | 0.842 |
| Gender (Female):ChatGPT | -3.07 | [-8.09, 1.94] | 2.56 | 0.229 |

Table 101: Linear Mixed Effect Model with 5 groups for Interpersonal Orientation and Gender Identity

| Predictors | Coef | CI | Std. Err. | p-value |
|---|---|---|---|---|
| Intercept | 0.52 | [-0.33, 1.37] | 0.43 | 0.232 |
| **Group (reference=Baseline)** | | | | |
| Copilot | -0.24 | [-1.97, 1.48] | 0.88 | 0.781 |
| Gemini | -0.02 | [-1.58, 1.55] | 0.8 | 0.983 |
| PI | -0.59 | [-2.23, 1.04] | 0.83 | 0.476 |
| ChatGPT | -0.02 | [-0.83, 0.8] | 0.42 | 0.967 |
| **Gender Identity (reference=Male)** | | | | |
| Female | -0.78 | [-1.92, 0.37] | 0.59 | 0.186 |
| Gender (Female):Copilot | 0.5 | [-1.86, 2.87] | 1.21 | 0.677 |
| Gender (Female):Gemini | 1.7 | [-0.8, 4.21] | 1.28 | 0.182 |
| Gender (Female):PI | 1.19 | [-1.22, 3.59] | 1.23 | 0.334 |
| Gender (Female):ChatGPT | 2.35 | [1.41, 3.3] | 0.48 | 0.0 |

Table 102: Linear Mixed Effect Model with 5 groups for Motivation for using AI (Escape) and Gender Identity

| Predictors | Coef | CI | Std. Err. | p-value |
|---|---|---|---|---|
| Intercept | 1.1 | [0.39, 1.82] | 0.37 | 0.003 |
| **Group (reference=Baseline)** | | | | |
| Copilot | -0.74 | [-1.96, 0.48] | 0.62 | 0.235 |
| Gemini | 0.54 | [-0.84, 1.92] | 0.7 | 0.443 |
| PI | -0.26 | [-1.65, 1.14] | 0.71 | 0.718 |
| ChatGPT | 1.0 | [-0.3, 2.29] | 0.66 | 0.132 |
| **Gender Identity (reference=Male)** | | | | |
| Female | -0.94 | [-2.05, 0.16] | 0.56 | 0.095 |
| Gender (Female):Copilot | 1.0 | [-0.91, 2.9] | 0.97 | 0.306 |
| Gender (Female):Gemini | 0.87 | [-1.4, 3.14] | 1.16 | 0.452 |
| Gender (Female):PI | 0.87 | [-1.31, 3.06] | 1.12 | 0.433 |
| Gender (Female):ChatGPT | 0.84 | [-1.17, 2.85] | 1.03 | 0.412 |

Table 103: Linear Mixed Effect Model with 5 groups for Motivation for using AI (Social) and Gender Identity

| Predictors | Coef | CI | Std. Err. | p-value |
|---|---|---|---|---|
| Intercept | 0.38 | [-0.16, 0.92] | 0.28 | 0.168 |
| **Group (reference=Baseline)** | | | | |
| Copilot | 0.44 | [-0.77, 1.65] | 0.62 | 0.477 |
| Gemini | 0.05 | [-0.99, 1.08] | 0.53 | 0.926 |
| PI | 0.08 | [-1.0, 1.16] | 0.55 | 0.881 |
| ChatGPT | 1.72 | [1.1, 2.34] | 0.32 | 0.0 |
| **Gender Identity (reference=Male)** | | | | |
| Female | -0.22 | [-0.92, 0.48] | 0.36 | 0.542 |
| Gender (Female):Copilot | 0.23 | [-1.38, 1.85] | 0.82 | 0.777 |
| Gender (Female):Gemini | 0.36 | [-1.34, 2.06] | 0.87 | 0.678 |
| Gender (Female):PI | -0.91 | [-2.61, 0.79] | 0.87 | 0.294 |
| Gender (Female):ChatGPT | 0.89 | [-0.31, 2.08] | 0.61 | 0.146 |

Table 104: Linear Mixed Effect Model with 5 groups for Motivation for using AI (Instrumental) and Gender Identity

| Predictors | Coef | CI | Std. Err. | p-value |
|---|---|---|---|---|
| Intercept | 0.38 | [-0.36, 1.11] | 0.37 | 0.311 |
| **Group (reference=Baseline)** | | | | |
| Copilot | 0.35 | [-1.19, 1.89] | 0.79 | 0.658 |
| Gemini | 0.19 | [-1.22, 1.6] | 0.72 | 0.789 |
| PI | -0.23 | [-1.65, 1.2] | 0.73 | 0.757 |
| ChatGPT | 2.02 | [0.46, 3.58] | 0.8 | 0.011 |
| **Gender Identity (reference=Male)** | | | | |
| Female | -0.35 | [-1.43, 0.74] | 0.55 | 0.532 |
| Gender (Female):Copilot | 1.04 | [-1.08, 3.15] | 1.08 | 0.337 |
| Gender (Female):Gemini | 0.92 | [-1.39, 3.22] | 1.18 | 0.435 |
| Gender (Female):PI | 0.19 | [-2.0, 2.39] | 1.12 | 0.863 |
| Gender (Female):ChatGPT | 0.02 | [-2.12, 2.17] | 1.09 | 0.983 |

Table 105: Linear Mixed Effect Model with 5 groups for Motivation for using AI (Entertainment) and Gender Identity

| Predictors | Coef | CI | Std. Err. | p-value |
|---|---|---|---|---|
| Intercept | 0.34 | [-0.06, 0.75] | 0.21 | 0.097 |
| **Group (reference=Baseline)** | | | | |
| Copilot | 0.02 | [-0.76, 0.8] | 0.4 | 0.962 |
| Gemini | 0.44 | [-0.35, 1.23] | 0.4 | 0.272 |
| PI | 0.04 | [-0.78, 0.86] | 0.42 | 0.924 |
| ChatGPT | 0.86 | [0.48, 1.23] | 0.19 | 0.0 |
| **Gender Identity (reference=Male)** | | | | |
| Female | -0.28 | [-0.84, 0.28] | 0.29 | 0.327 |
| Gender (Female):Copilot | 0.17 | [-0.94, 1.27] | 0.56 | 0.767 |
| Gender (Female):Gemini | 0.64 | [-0.65, 1.93] | 0.66 | 0.333 |
| Gender (Female):PI | 0.34 | [-0.89, 1.57] | 0.63 | 0.588 |
| Gender (Female):ChatGPT | 0.7 | [-0.02, 1.41] | 0.37 | 0.058 |

Table 106: Linear Mixed Effect Model with 5 groups for Attachment towards AI and Gender Identity

| Predictors | Coef | CI | Std. Err. | p-value |
|---|---|---|---|---|
| Intercept | 0.76 | [0.53, 0.98] | 0.11 | 0.0 |
| **Group (reference=Baseline)** | | | | |
| Copilot | -0.49 | [-1.17, 0.2] | 0.35 | 0.166 |
| Gemini | 0.1 | [-0.56, 0.76] | 0.34 | 0.77 |
| PI | -0.3 | [-0.85, 0.26] | 0.28 | 0.294 |
| ChatGPT | -0.16 | [-0.91, 0.59] | 0.38 | 0.68 |
| **Gender Identity (reference=Male)** | | | | |
| Female | -0.76 | [-1.18, -0.34] | 0.21 | 0.0 |
| Gender (Female):Copilot | 0.65 | [-0.26, 1.56] | 0.46 | 0.16 |
| Gender (Female):Gemini | 0.62 | [-0.49, 1.72] | 0.56 | 0.276 |
| Gender (Female):PI | 0.3 | [-0.63, 1.22] | 0.47 | 0.529 |
| Gender (Female):ChatGPT | 0.93 | [-0.02, 1.87] | 0.48 | 0.054 |

Table 107: Linear Mixed Effect Model with 5 groups for Recommendation to use AI and Gender Identity

| Predictors | Coef | CI | Std. Err. | p-value |
|---|---|---|---|---|
| Intercept | 0.17 | [-0.13, 0.48] | 0.15 | 0.265 |
| **Group (reference=Baseline)** | | | | |
| Copilot | 0.01 | [-0.44, 0.46] | 0.23 | 0.967 |
| Gemini | 0.47 | [-0.17, 1.11] | 0.33 | 0.15 |
| PI | 0.37 | [-0.24, 0.98] | 0.31 | 0.239 |
| ChatGPT | 0.13 | [-0.51, 0.77] | 0.33 | 0.695 |
| **Gender Identity (reference=Male)** | | | | |
| Female | -0.01 | [-0.4, 0.37] | 0.2 | 0.955 |
| Gender (Female):Copilot | 0.5 | [-0.08, 1.07] | 0.29 | 0.089 |
| Gender (Female):Gemini | 0.23 | [-0.82, 1.28] | 0.54 | 0.674 |
| Gender (Female):PI | -0.31 | [-1.29, 0.67] | 0.5 | 0.542 |
| Gender (Female):ChatGPT | 0.4 | [-0.48, 1.29] | 0.45 | 0.372 |

Table 108: Linear Mixed Effect Model with 5 groups for Satisfaction with AI and Gender Identity

| Predictors | Coef | CI | Std. Err. | p-value |
|---|---|---|---|---|
| Intercept | 0.14 | [-0.03, 0.31] | 0.09 | 0.112 |
| **Group (reference=Baseline)** | | | | |
| Copilot | 0.23 | [-0.43, 0.89] | 0.34 | 0.502 |
| Gemini | 0.22 | [-0.37, 0.81] | 0.3 | 0.468 |
| PI | 0.25 | [-0.32, 0.81] | 0.29 | 0.393 |
| ChatGPT | 0.16 | [-0.51, 0.83] | 0.34 | 0.635 |
| **Gender Identity (reference=Male)** | | | | |
| Female | 0.12 | [-0.24, 0.48] | 0.18 | 0.516 |
| Gender (Female):Copilot | 0.18 | [-0.69, 1.06] | 0.45 | 0.683 |
| Gender (Female):Gemini | 0.38 | [-0.62, 1.38] | 0.51 | 0.458 |
| Gender (Female):PI | -0.28 | [-1.15, 0.59] | 0.44 | 0.525 |
| Gender (Female):ChatGPT | 0.04 | [-0.83, 0.92] | 0.45 | 0.926 |

Table 109: Linear Mixed Effect Model with 5 groups for AI Helpfulness and Gender Identity

| Predictors | Coef | CI | Std. Err. | p-value |
|---|---|---|---|---|
| Intercept | 0.07 | [-0.34, 0.48] | 0.21 | 0.744 |
| **Group (reference=Baseline)** | | | | |
| Copilot | 0.11 | [-0.73, 0.96] | 0.43 | 0.793 |
| Gemini | 0.0 | [-0.73, 0.73] | 0.37 | 0.995 |
| PI | -0.07 | [-0.85, 0.71] | 0.4 | 0.863 |
| ChatGPT | 0.43 | [-0.34, 1.21] | 0.4 | 0.275 |
| **Gender Identity (reference=Male)** | | | | |
| Female | 0.06 | [-0.56, 0.68] | 0.31 | 0.848 |
| Gender (Female):Copilot | -0.16 | [-1.33, 1.01] | 0.6 | 0.791 |
| Gender (Female):Gemini | 0.01 | [-1.23, 1.26] | 0.64 | 0.986 |
| Gender (Female):PI | 1.05 | [-0.16, 2.26] | 0.62 | 0.088 |
| Gender (Female):ChatGPT | 0.44 | [-0.46, 1.34] | 0.46 | 0.337 |

Table 110: Linear Mixed Effect Model with 5 groups for Perceived Human-Like Behavior and Gender Identity

| Predictors | Coef | CI | Std. Err. | p-value |
|---|---|---|---|---|
| Intercept | 0.18 | [-0.08, 0.44] | 0.13 | 0.182 |
| **Group (reference=Baseline)** | | | | |
| Copilot | 0.38 | [-0.18, 0.94] | 0.29 | 0.185 |
| Gemini | 0.2 | [-0.3, 0.7] | 0.25 | 0.436 |
| PI | 0.18 | [-0.35, 0.71] | 0.27 | 0.507 |
| ChatGPT | 1.05 | [0.62, 1.48] | 0.22 | 0.0 |
| **Gender Identity (reference=Male)** | | | | |
| Female | -0.08 | [-0.42, 0.27] | 0.18 | 0.666 |
| Gender (Female):Copilot | 0.55 | [-0.21, 1.31] | 0.39 | 0.154 |
| Gender (Female):Gemini | 0.61 | [-0.18, 1.4] | 0.4 | 0.128 |
| Gender (Female):PI | 0.69 | [-0.09, 1.47] | 0.4 | 0.083 |
| Gender (Female):ChatGPT | 0.18 | [-0.27, 0.62] | 0.23 | 0.432 |

Table 111: Linear Mixed Effect Model with 5 groups for Perceived AI empathy and Gender Identity

| Predictors | Coef | CI | Std. Err. | p-value |
|---|---|---|---|---|
| Intercept | 0.29 | [-0.1, 0.68] | 0.2 | 0.141 |
| **Group (reference=Baseline)** | | | | |
| Copilot | -0.29 | [-1.65, 1.07] | 0.69 | 0.675 |
| Gemini | 0.15 | [-1.41, 1.72] | 0.8 | 0.847 |
| PI | 1.38 | [-0.2, 2.95] | 0.8 | 0.087 |
| ChatGPT | 0.04 | [-1.2, 1.28] | 0.63 | 0.946 |
| **Mental Health Status (reference=No)** | | | | |
| Yes | 0.16 | [-0.54, 0.86] | 0.36 | 0.659 |
| Mental Health Status (Yes):Copilot | 0.18 | [-1.66, 2.01] | 0.93 | 0.851 |
| Mental Health Status (Yes):Gemini | -0.52 | [-2.62, 1.58] | 1.07 | 0.628 |
| Mental Health Status (Yes):PI | -1.67 | [-3.81, 0.47] | 1.09 | 0.126 |
| Mental Health Status (Yes):ChatGPT | -0.21 | [-1.89, 1.48] | 0.86 | 0.811 |

Table 112: Linear Mixed Effect Model with 5 groups for Dependence on AI and Mental Health Status

| Predictors | Coef | CI | Std. Err. | p-value |
|---|---|---|---|---|
| Intercept | 0.06 | [-0.16, 0.29] | 0.11 | 0.567 |
| **Group (reference=Baseline)** | | | | |
| Copilot | -0.16 | [-0.6, 0.29] | 0.23 | 0.49 |
| Gemini | 0.05 | [-0.44, 0.53] | 0.25 | 0.851 |
| PI | 0.49 | [0.01, 0.97] | 0.25 | 0.046 |
| ChatGPT | 0.16 | [-0.33, 0.64] | 0.25 | 0.525 |
| **Mental Health Status (reference=No)** | | | | |
| Yes | -0.03 | [-0.35, 0.29] | 0.16 | 0.852 |
| Mental Health Status (Yes):Copilot | 0.12 | [-0.51, 0.75] | 0.32 | 0.708 |
| Mental Health Status (Yes):Gemini | -0.16 | [-0.81, 0.49] | 0.33 | 0.62 |
| Mental Health Status (Yes):PI | -0.45 | [-1.05, 0.15] | 0.31 | 0.144 |
| Mental Health Status (Yes):ChatGPT | -0.12 | [-0.77, 0.52] | 0.33 | 0.714 |

Table 113: Linear Mixed Effect Model with 5 groups for Dependence on AI (Over-reliance) and Mental Health Status

| Predictors | Coef | CI | Std. Err. | p-value |
|---|---|---|---|---|
| Intercept | 0.03 | [-0.2, 0.26] | 0.12 | 0.782 |
| **Group (reference=Baseline)** | | | | |
| Copilot | -0.21 | [-0.64, 0.21] | 0.22 | 0.328 |
| Gemini | -0.03 | [-0.52, 0.46] | 0.25 | 0.897 |
| PI | 0.3 | [-0.09, 0.7] | 0.2 | 0.136 |
| ChatGPT | 0.08 | [-0.41, 0.57] | 0.25 | 0.751 |
| **Mental Health Status (reference=No)** | | | | |
| Yes | -0.03 | [-0.36, 0.3] | 0.17 | 0.849 |
| Mental Health Status (Yes):Copilot | 0.13 | [-0.41, 0.67] | 0.28 | 0.637 |
| Mental Health Status (Yes):Gemini | 0.03 | [-0.63, 0.69] | 0.34 | 0.924 |
| Mental Health Status (Yes):PI | -0.3 | [-0.85, 0.25] | 0.28 | 0.286 |
| Mental Health Status (Yes):ChatGPT | -0.08 | [-0.72, 0.57] | 0.33 | 0.81 |

Table 114: Linear Mixed Effect Model with 5 groups for Dependence on AI (Excessive Usage) and Mental Health Status

| Predictors | Coef | CI | Std. Err. | p-value |
|---|---|---|---|---|
| Intercept | -0.06 | [-0.17, 0.04] | 0.05 | 0.21 |
| **Group (reference=Baseline)** | | | | |
| Copilot | 0.06 | [-0.13, 0.26] | 0.1 | 0.52 |
| Gemini | 0.06 | [-0.16, 0.29] | 0.11 | 0.572 |
| PI | 0.18 | [-0.04, 0.39] | 0.11 | 0.104 |
| ChatGPT | 0.06 | [-0.19, 0.32] | 0.13 | 0.62 |
| **Mental Health Status (reference=No)** | | | | |
| Yes | 0.17 | [-0.01, 0.34] | 0.09 | 0.062 |
| Mental Health Status (Yes):Copilot | -0.0 | [-0.31, 0.3] | 0.16 | 0.993 |
| Mental Health Status (Yes):Gemini | -0.08 | [-0.42, 0.25] | 0.17 | 0.618 |
| Mental Health Status (Yes):PI | -0.36 | [-0.65, -0.07] | 0.15 | 0.016 |
| Mental Health Status (Yes):ChatGPT | -0.17 | [-0.53, 0.19] | 0.18 | 0.359 |

Table 115: Linear Mixed Effect Model with 5 groups for Dependence on AI (Jeopardization) and Mental Health Status

| Predictors | Coef | CI | Std. Err. | p-value |
|---|---|---|---|---|
| Intercept | 0.1 | [-0.05, 0.24] | 0.07 | 0.187 |
| **Group (reference=Baseline)** | | | | |
| Copilot | 0.18 | [-0.09, 0.44] | 0.14 | 0.194 |
| Gemini | 0.13 | [-0.29, 0.54] | 0.21 | 0.554 |
| PI | 0.35 | [-0.08, 0.78] | 0.22 | 0.112 |
| ChatGPT | -0.1 | [-0.55, 0.35] | 0.23 | 0.672 |
| **Mental Health Status (reference=No)** | | | | |
| Yes | 0.04 | [-0.24, 0.32] | 0.14 | 0.771 |
| Mental Health Status (Yes):Copilot | -0.23 | [-0.67, 0.21] | 0.22 | 0.303 |
| Mental Health Status (Yes):Gemini | -0.18 | [-0.77, 0.41] | 0.3 | 0.548 |
| Mental Health Status (Yes):PI | -0.41 | [-1.02, 0.21] | 0.31 | 0.192 |
| Mental Health Status (Yes):ChatGPT | 0.1 | [-0.52, 0.73] | 0.32 | 0.75 |

Table 116: Linear Mixed Effect Model with 5 groups for Dependence on AI (Withdrawal) and Mental Health Status

| Predictors | Coef | CI | Std. Err. | p-value |
|---|---|---|---|---|
| Intercept | 0.16 | [-0.02, 0.34] | 0.09 | 0.077 |
| **Group (reference=Baseline)** | | | | |
| Copilot | -0.16 | [-0.51, 0.19] | 0.18 | 0.368 |
| Gemini | -0.05 | [-0.43, 0.33] | 0.19 | 0.795 |
| PI | 0.06 | [-0.32, 0.44] | 0.19 | 0.752 |
| ChatGPT | -0.16 | [-0.54, 0.22] | 0.19 | 0.404 |
| **Mental Health Status (reference=No)** | | | | |
| Yes | 0.01 | [-0.19, 0.21] | 0.1 | 0.915 |
| Mental Health Status (Yes):Copilot | 0.16 | [-0.29, 0.6] | 0.23 | 0.493 |
| Mental Health Status (Yes):Gemini | -0.12 | [-0.61, 0.37] | 0.25 | 0.624 |
| Mental Health Status (Yes):PI | -0.16 | [-0.64, 0.32] | 0.25 | 0.524 |
| Mental Health Status (Yes):ChatGPT | 0.06 | [-0.42, 0.54] | 0.24 | 0.804 |

Table 117: Linear Mixed Effect Model with 5 groups for Dependence on AI (Loss of Control) and Mental Health Status

| Predictors | Coef | CI | Std. Err. | p-value |
|---|---|---|---|---|
| Intercept | -0.03 | [-0.21, 0.16] | 0.1 | 0.783 |
| **Group (reference=Baseline)** | | | | |
| Copilot | 0.25 | [-0.18, 0.67] | 0.22 | 0.254 |
| Gemini | 0.18 | [-0.26, 0.62] | 0.23 | 0.418 |
| PI | 0.38 | [-0.13, 0.88] | 0.26 | 0.143 |
| ChatGPT | 0.51 | [0.0, 1.02] | 0.26 | 0.05 |
| **Mental Health Status (reference=No)** | | | | |
| Yes | 0.09 | [-0.26, 0.44] | 0.18 | 0.599 |
| Mental Health Status (Yes):Copilot | -0.69 | [-1.35, -0.03] | 0.34 | 0.041 |
| Mental Health Status (Yes):Gemini | -0.6 | [-1.28, 0.08] | 0.35 | 0.082 |
| Mental Health Status (Yes):PI | -0.42 | [-1.09, 0.26] | 0.34 | 0.227 |
| Mental Health Status (Yes):ChatGPT | 0.15 | [-0.49, 0.79] | 0.32 | 0.641 |

Table 118: Linear Mixed Effect Model with 5 groups for Attitude towards AI and Mental Health Status

| Predictors | Coef | CI | Std. Err. | p-value |
|---|---|---|---|---|
| Intercept | -0.05 | [-0.17, 0.07] | 0.06 | 0.446 |
| **Group (reference=Baseline)** | | | | |
| Copilot | 0.01 | [-0.28, 0.29] | 0.14 | 0.966 |
| Gemini | 0.24 | [-0.01, 0.5] | 0.13 | 0.058 |
| PI | 0.23 | [-0.08, 0.54] | 0.16 | 0.141 |
| ChatGPT | 0.38 | [0.2, 0.56] | 0.09 | 0.0 |
| **Mental Health Status (reference=No)** | | | | |
| Yes | -0.01 | [-0.21, 0.19] | 0.1 | 0.945 |
| Mental Health Status (Yes):Copilot | -0.05 | [-0.44, 0.35] | 0.2 | 0.822 |
| Mental Health Status (Yes):Gemini | -0.38 | [-0.74, -0.03] | 0.18 | 0.035 |
| Mental Health Status (Yes):PI | -0.26 | [-0.68, 0.15] | 0.21 | 0.212 |
| Mental Health Status (Yes):ChatGPT | 0.04 | [-0.27, 0.35] | 0.16 | 0.807 |

Table 119: Linear Mixed Effect Model with 5 groups for Attitude towards AI (Positive) and Mental Health Status

| Predictors | Coef | CI | Std. Err. | p-value |
|---|---|---|---|---|
| Intercept | 0.02 | [-0.15, 0.19] | 0.09 | 0.82 |
| **Group (reference=Baseline)** | | | | |
| Copilot | 0.24 | [-0.1, 0.58] | 0.17 | 0.162 |
| Gemini | -0.06 | [-0.43, 0.3] | 0.19 | 0.74 |
| PI | 0.15 | [-0.22, 0.51] | 0.19 | 0.432 |
| ChatGPT | 0.13 | [-0.23, 0.5] | 0.19 | 0.477 |
| **Mental Health Status (reference=No)** | | | | |
| Yes | 0.1 | [-0.15, 0.35] | 0.13 | 0.429 |
| Mental Health Status (Yes):Copilot | -0.64 | [-1.12, -0.17] | 0.24 | 0.008 |
| Mental Health Status (Yes):Gemini | -0.22 | [-0.71, 0.28] | 0.25 | 0.392 |
| Mental Health Status (Yes):PI | -0.15 | [-0.64, 0.33] | 0.25 | 0.541 |
| Mental Health Status (Yes):ChatGPT | 0.11 | [-0.37, 0.59] | 0.25 | 0.646 |

Table 120: Linear Mixed Effect Model with 5 groups for Attitude towards AI (Negative) and Mental Health Status

| Predictors | Coef | CI | Std. Err. | p-value |
|---|---|---|---|---|
| Intercept | 0.35 | [-1.47, 2.18] | 0.93 | 0.703 |
| **Group (reference=Baseline)** | | | | |
| Copilot | 3.37 | [-0.2, 6.94] | 1.82 | 0.064 |
| Gemini | -0.13 | [-3.91, 3.65] | 1.93 | 0.945 |
| PI | 0.42 | [-3.59, 4.44] | 2.05 | 0.836 |
| ChatGPT | 3.87 | [0.3, 7.43] | 1.82 | 0.034 |
| **Mental Health Status (reference=No)** | | | | |
| Yes | 0.96 | [-1.49, 3.4] | 1.25 | 0.443 |
| Mental Health Status (Yes):Copilot | -3.77 | [-8.12, 0.59] | 2.22 | 0.09 |
| Mental Health Status (Yes):Gemini | 1.91 | [-3.25, 7.06] | 2.63 | 0.469 |
| Mental Health Status (Yes):PI | 0.5 | [-4.87, 5.87] | 2.74 | 0.856 |
| Mental Health Status (Yes):ChatGPT | -1.68 | [-6.74, 3.39] | 2.58 | 0.516 |

Table 121: Linear Mixed Effect Model with 5 groups for Interpersonal Orientation and Mental Health Status

| Predictors | Coef | CI | Std. Err. | p-value |
|---|---|---|---|---|
| Intercept | 0.06 | [-0.63, 0.76] | 0.35 | 0.855 |
| **Group (reference=Baseline)** | | | | |
| Copilot | -0.34 | [-1.84, 1.16] | 0.77 | 0.66 |
| Gemini | 0.49 | [-1.13, 2.11] | 0.83 | 0.552 |
| PI | -0.06 | [-1.68, 1.55] | 0.83 | 0.938 |
| ChatGPT | 1.6 | [-0.2, 3.4] | 0.92 | 0.081 |
| **Mental Health Status (reference=No)** | | | | |
| Yes | 0.11 | [-1.18, 1.4] | 0.66 | 0.87 |
| Mental Health Status (Yes):Copilot | 0.66 | [-1.76, 3.09] | 1.24 | 0.591 |
| Mental Health Status (Yes):Gemini | 0.34 | [-2.2, 2.87] | 1.3 | 0.795 |
| Mental Health Status (Yes):PI | 0.05 | [-2.47, 2.56] | 1.28 | 0.971 |
| Mental Health Status (Yes):ChatGPT | -0.56 | [-3.05, 1.93] | 1.27 | 0.659 |

Table 122: Linear Mixed Effect Model with 5 groups for Motivation for using AI (Escape) and Mental Health Status

| Predictors | Coef | CI | Std. Err. | p-value |
|---|---|---|---|---|
| Intercept | 0.55 | [-0.05, 1.15] | 0.31 | 0.073 |
| **Group (reference=Baseline)** | | | | |
| Copilot | -0.28 | [-1.7, 1.14] | 0.72 | 0.704 |
| Gemini | 0.56 | [-1.09, 2.21] | 0.84 | 0.503 |
| PI | 0.01 | [-1.63, 1.65] | 0.84 | 0.993 |
| ChatGPT | 1.34 | [0.01, 2.67] | 0.68 | 0.048 |
| **Mental Health Status (reference=No)** | | | | |
| Yes | 0.14 | [-0.73, 1.01] | 0.44 | 0.75 |
| Mental Health Status (Yes):Copilot | 0.09 | [-1.86, 2.03] | 0.99 | 0.931 |
| Mental Health Status (Yes):Gemini | 0.75 | [-1.44, 2.94] | 1.12 | 0.504 |
| Mental Health Status (Yes):PI | 0.3 | [-1.83, 2.44] | 1.09 | 0.781 |
| Mental Health Status (Yes):ChatGPT | 0.11 | [-1.1, 1.32] | 0.62 | 0.855 |

Table 123: Linear Mixed Effect Model with 5 groups for Motivation for using AI (Social) and Mental Health Status

| Predictors | Coef | CI | Std. Err. | p-value |
|---|---|---|---|---|
| Intercept | 0.65 | [0.01, 1.28] | 0.32 | 0.045 |
| **Group (reference=Baseline)** | | | | |
| Copilot | -0.1 | [-1.25, 1.05] | 0.59 | 0.866 |
| Gemini | -0.09 | [-1.42, 1.24] | 0.68 | 0.895 |
| PI | 0.47 | [-0.86, 1.79] | 0.68 | 0.492 |
| ChatGPT | 2.69 | [1.7, 3.68] | 0.5 | 0.0 |
| **Mental Health Status (reference=No)** | | | | |
| Yes | -0.78 | [-1.66, 0.1] | 0.45 | 0.081 |
| Mental Health Status (Yes):Copilot | 1.32 | [-0.37, 3.01] | 0.86 | 0.126 |
| Mental Health Status (Yes):Gemini | 0.64 | [-1.15, 2.44] | 0.92 | 0.482 |
| Mental Health Status (Yes):PI | -1.1 | [-2.87, 0.67] | 0.9 | 0.224 |
| Mental Health Status (Yes):ChatGPT | -0.62 | [-1.94, 0.69] | 0.67 | 0.355 |

Table 124: Linear Mixed Effect Model with 5 groups for Motivation for using AI (Instrumental) and Mental Health Status

| Predictors | Coef | CI | Std. Err. | p-value |
|---|---|---|---|---|
| Intercept | 0.61 | [-0.13, 1.36] | 0.38 | 0.108 |
| **Group (reference=Baseline)** | | | | |
| Copilot | 0.3 | [-1.2, 1.79] | 0.76 | 0.697 |
| Gemini | 0.94 | [-0.62, 2.51] | 0.8 | 0.238 |
| PI | 0.28 | [-1.25, 1.8] | 0.78 | 0.723 |
| ChatGPT | 2.16 | [0.76, 3.57] | 0.72 | 0.003 |
| **Mental Health Status (reference=No)** | | | | |
| Yes | -0.85 | [-1.96, 0.25] | 0.56 | 0.128 |
| Mental Health Status (Yes):Copilot | 1.2 | [-0.9, 3.29] | 1.07 | 0.263 |
| Mental Health Status (Yes):Gemini | -0.53 | [-2.66, 1.6] | 1.09 | 0.623 |
| Mental Health Status (Yes):PI | -0.5 | [-2.6, 1.61] | 1.07 | 0.644 |
| Mental Health Status (Yes):ChatGPT | -0.07 | [-1.46, 1.33] | 0.71 | 0.926 |

Table 125: Linear Mixed Effect Model with 5 groups for Motivation for using AI (Entertainment) and Mental Health Status

| Predictors | Coef | CI | Std. Err. | p-value |
|---|---|---|---|---|
| Intercept | 0.19 | [-0.22, 0.6] | 0.21 | 0.353 |
| **Group (reference=Baseline)** | | | | |
| Copilot | -0.28 | [-1.07, 0.5] | 0.4 | 0.479 |
| Gemini | 1.36 | [0.53, 2.19] | 0.42 | 0.001 |
| PI | 0.58 | [-0.32, 1.49] | 0.46 | 0.205 |
| ChatGPT | 1.25 | [0.34, 2.16] | 0.46 | 0.007 |
| **Mental Health Status (reference=No)** | | | | |
| Yes | 0.01 | [-0.59, 0.62] | 0.31 | 0.965 |
| Mental Health Status (Yes):Copilot | 0.74 | [-0.43, 1.92] | 0.6 | 0.215 |
| Mental Health Status (Yes):Gemini | -1.15 | [-2.36, 0.06] | 0.62 | 0.062 |
| Mental Health Status (Yes):PI | -0.64 | [-1.79, 0.52] | 0.59 | 0.281 |
| Mental Health Status (Yes):ChatGPT | -0.03 | [-1.22, 1.16] | 0.61 | 0.962 |

Table 126: Linear Mixed Effect Model with 5 groups for Attachment towards AI and Mental Health Status

| Predictors | Coef | CI | Std. Err. | p-value |
|---|---|---|---|---|
| Intercept | 0.26 | [0.01, 0.51] | 0.13 | 0.042 |
| **Group (reference=Baseline)** | | | | |
| Copilot | -0.53 | [-1.16, 0.1] | 0.32 | 0.1 |
| Gemini | 0.41 | [-0.41, 1.22] | 0.42 | 0.327 |
| PI | 0.52 | [-0.29, 1.33] | 0.41 | 0.208 |
| ChatGPT | 0.63 | [-0.0, 1.26] | 0.32 | 0.051 |
| **Mental Health Status (reference=No)** | | | | |
| Yes | 0.22 | [-0.24, 0.69] | 0.24 | 0.345 |
| Mental Health Status (Yes):Copilot | 0.71 | [-0.22, 1.64] | 0.47 | 0.132 |
| Mental Health Status (Yes):Gemini | 0.03 | [-1.12, 1.17] | 0.58 | 0.965 |
| Mental Health Status (Yes):PI | -1.08 | [-2.21, 0.05] | 0.57 | 0.06 |
| Mental Health Status (Yes):ChatGPT | -0.54 | [-1.41, 0.33] | 0.44 | 0.221 |

Table 127: Linear Mixed Effect Model with 5 groups for Recommendation to use AI and Mental Health Status

| Predictors | Coef | CI | Std. Err. | p-value |
|---|---|---|---|---|
| Intercept | 0.19 | [-0.12, 0.51] | 0.16 | 0.224 |
| **Group (reference=Baseline)** | | | | |
| Copilot | 0.17 | [-0.5, 0.84] | 0.34 | 0.621 |
| Gemini | 0.47 | [-0.25, 1.2] | 0.37 | 0.199 |
| PI | 1.14 | [0.62, 1.66] | 0.26 | 0.0 |
| ChatGPT | 0.47 | [-0.24, 1.19] | 0.37 | 0.196 |
| **Mental Health Status (reference=No)** | | | | |
| Yes | -0.06 | [-0.55, 0.44] | 0.25 | 0.826 |
| Mental Health Status (Yes):Copilot | 0.19 | [-0.74, 1.13] | 0.48 | 0.687 |
| Mental Health Status (Yes):Gemini | 0.14 | [-0.84, 1.12] | 0.5 | 0.781 |
| Mental Health Status (Yes):PI | -1.51 | [-2.43, -0.58] | 0.47 | 0.001 |
| Mental Health Status (Yes):ChatGPT | -0.18 | [-1.06, 0.69] | 0.45 | 0.682 |

Table 128: Linear Mixed Effect Model with 5 groups for Satisfaction with AI and Mental Health Status

| Predictors | Coef | CI | Std. Err. | p-value |
|---|---|---|---|---|
| Intercept | 0.13 | [-0.18, 0.44] | 0.16 | 0.412 |
| **Group (reference=Baseline)** | | | | |
| Copilot | 0.14 | [-0.32, 0.61] | 0.24 | 0.545 |
| Gemini | 0.2 | [-0.46, 0.87] | 0.34 | 0.547 |
| PI | 0.76 | [0.06, 1.46] | 0.36 | 0.033 |
| ChatGPT | 0.54 | [-0.1, 1.18] | 0.33 | 0.1 |
| **Mental Health Status (reference=No)** | | | | |
| Yes | 0.15 | [-0.21, 0.5] | 0.18 | 0.421 |
| Mental Health Status (Yes):Copilot | 0.33 | [-0.33, 0.99] | 0.33 | 0.323 |
| Mental Health Status (Yes):Gemini | 0.19 | [-0.72, 1.09] | 0.46 | 0.686 |
| Mental Health Status (Yes):PI | -1.11 | [-2.02, -0.2] | 0.46 | 0.016 |
| Mental Health Status (Yes):ChatGPT | -0.6 | [-1.35, 0.15] | 0.38 | 0.117 |

Table 129: Linear Mixed Effect Model with 5 groups for AI Helpfulness and Mental Health Status

| Predictors | Coef | CI | Std. Err. | p-value |
|---|---|---|---|---|
| Intercept | 0.26 | [-0.16, 0.67] | 0.21 | 0.222 |
| **Group (reference=Baseline)** | | | | |
| Copilot | -0.44 | [-1.23, 0.35] | 0.4 | 0.276 |
| Gemini | -0.26 | [-1.14, 0.63] | 0.45 | 0.567 |
| PI | 0.63 | [-0.11, 1.37] | 0.38 | 0.095 |
| ChatGPT | 0.52 | [-0.37, 1.41] | 0.46 | 0.253 |
| **Mental Health Status (reference=No)** | | | | |
| Yes | -0.33 | [-0.83, 0.17] | 0.26 | 0.201 |
| Mental Health Status (Yes):Copilot | 0.93 | [-0.04, 1.89] | 0.49 | 0.061 |
| Mental Health Status (Yes):Gemini | 0.49 | [-0.67, 1.65] | 0.59 | 0.404 |
| Mental Health Status (Yes):PI | -0.41 | [-1.25, 0.43] | 0.43 | 0.34 |
| Mental Health Status (Yes):ChatGPT | 0.33 | [-0.84, 1.51] | 0.6 | 0.575 |

Table 130: Linear Mixed Effect Model with 5 groups for Perceived Human-Like Behavior and Mental Health Status

| Predictors | Coef | CI | Std. Err. | p-value |
|---|---|---|---|---|
| Intercept | 0.16 | [-0.13, 0.44] | 0.15 | 0.279 |
| **Group (reference=Baseline)** | | | | |
| Copilot | 0.3 | [-0.26, 0.86] | 0.28 | 0.296 |
| Gemini | 0.13 | [-0.46, 0.73] | 0.31 | 0.66 |
| PI | 0.66 | [0.08, 1.24] | 0.3 | 0.025 |
| ChatGPT | 1.05 | [0.57, 1.53] | 0.24 | 0.0 |
| **Mental Health Status (reference=No)** | | | | |
| Yes | -0.04 | [-0.45, 0.37] | 0.21 | 0.844 |
| Mental Health Status (Yes):Copilot | 0.71 | [-0.07, 1.49] | 0.4 | 0.074 |
| Mental Health Status (Yes):Gemini | 0.5 | [-0.3, 1.3] | 0.41 | 0.221 |
| Mental Health Status (Yes):PI | -0.32 | [-1.11, 0.48] | 0.41 | 0.434 |
| Mental Health Status (Yes):ChatGPT | 0.16 | [-0.46, 0.78] | 0.32 | 0.606 |

Table 131: Linear Mixed Effect Model with 5 groups for Perceived AI empathy and Mental Health Status

| Predictors | Coef | CI | Std. Err. | p-value |
|---|---|---|---|---|
| Intercept | 0.81 | [0.11, 1.51] | 0.36 | 0.023 |
| **Group (reference=Baseline)** | | | | |
| Copilot | -0.41 | [-1.92, 1.1] | 0.77 | 0.595 |
| Gemini | -0.9 | [-2.36, 0.56] | 0.74 | 0.225 |
| PI | 0.19 | [-1.27, 1.65] | 0.74 | 0.799 |
| ChatGPT | -0.09 | [-1.31, 1.13] | 0.62 | 0.887 |
| **AI Usage Label (reference=Cold)** | | | | |
| Hot | -1.16 | [-2.29, -0.03] | 0.57 | 0.044 |
| AI Usage (Hot):Copilot | 0.76 | [-1.35, 2.87] | 1.08 | 0.481 |
| AI Usage (Hot):Gemini | 1.85 | [-0.32, 4.02] | 1.11 | 0.095 |
| AI Usage (Hot):PI | 0.7 | [-1.43, 2.84] | 1.09 | 0.517 |
| AI Usage (Hot):ChatGPT | -0.76 | [-3.19, 1.66] | 1.24 | 0.537 |

Table 132: Linear Mixed Effect Model with 5 groups for Dependence on AI and AI Usage Label

| Predictors | Coef | CI | Std. Err. | p-value |
|---|---|---|---|---|
| Intercept | 0.11 | [-0.1, 0.32] | 0.11 | 0.319 |
| **Group (reference=Baseline)** | | | | |
| Copilot | -0.11 | [-0.57, 0.35] | 0.24 | 0.646 |
| Gemini | -0.11 | [-0.55, 0.34] | 0.23 | 0.633 |
| PI | 0.26 | [-0.19, 0.7] | 0.23 | 0.259 |
| ChatGPT | 0.17 | [-0.2, 0.54] | 0.19 | 0.371 |
| **AI Usage Label (reference=Cold)** | | | | |
| Hot | -0.15 | [-0.49, 0.19] | 0.18 | 0.387 |
| AI Usage (Hot):Copilot | 0.07 | [-0.57, 0.72] | 0.33 | 0.82 |
| AI Usage (Hot):Gemini | 0.15 | [-0.51, 0.81] | 0.34 | 0.653 |
| AI Usage (Hot):PI | -0.03 | [-0.68, 0.62] | 0.33 | 0.927 |
| AI Usage (Hot):ChatGPT | -0.53 | [-1.26, 0.21] | 0.38 | 0.162 |

Table 133: Linear Mixed Effect Model with 5 groups for Dependence on AI (Over-reliance) and AI Usage Label

| Predictors | Coef | CI | Std. Err. | p-value |
|---|---|---|---|---|
| Intercept | 0.11 | [-0.1, 0.31] | 0.11 | 0.304 |
| **Group (reference=Baseline)** | | | | |
| Copilot | 0.09 | [-0.36, 0.54] | 0.23 | 0.687 |
| Gemini | -0.2 | [-0.63, 0.23] | 0.22 | 0.365 |
| PI | 0.07 | [-0.36, 0.5] | 0.22 | 0.737 |
| ChatGPT | 0.06 | [-0.3, 0.42] | 0.18 | 0.75 |
| **AI Usage Label (reference=Cold)** | | | | |
| Hot | -0.24 | [-0.57, 0.09] | 0.17 | 0.16 |
| AI Usage (Hot):Copilot | -0.35 | [-0.97, 0.28] | 0.32 | 0.277 |
| AI Usage (Hot):Gemini | 0.43 | [-0.21, 1.07] | 0.33 | 0.189 |
| AI Usage (Hot):PI | 0.15 | [-0.48, 0.78] | 0.32 | 0.646 |
| AI Usage (Hot):ChatGPT | -0.33 | [-1.04, 0.39] | 0.37 | 0.369 |

Table 134: Linear Mixed Effect Model with 5 groups for Dependence on AI (Excessive Usage) and AI Usage Label

| Predictors | Coef | CI | Std. Err. | p-value |
|---|---|---|---|---|
| Intercept | 0.05 | [-0.07, 0.17] | 0.06 | 0.379 |
| **Group (reference=Baseline)** | | | | |
| Copilot | -0.05 | [-0.32, 0.21] | 0.13 | 0.685 |
| Gemini | -0.05 | [-0.31, 0.2] | 0.13 | 0.674 |
| PI | -0.05 | [-0.31, 0.2] | 0.13 | 0.674 |
| ChatGPT | -0.05 | [-0.26, 0.16] | 0.11 | 0.615 |
| **AI Usage Label (reference=Cold)** | | | | |
| Hot | -0.1 | [-0.29, 0.1] | 0.1 | 0.326 |
| AI Usage (Hot):Copilot | 0.25 | [-0.11, 0.62] | 0.19 | 0.177 |
| AI Usage (Hot):Gemini | 0.2 | [-0.18, 0.57] | 0.19 | 0.302 |
| AI Usage (Hot):PI | 0.1 | [-0.27, 0.47] | 0.19 | 0.604 |
| AI Usage (Hot):ChatGPT | 0.1 | [-0.32, 0.52] | 0.21 | 0.648 |

Table 135: Linear Mixed Effect Model with 5 groups for Dependence on AI (Jeopardization) and AI Usage Label

| Predictors | Coef | CI | Std. Err. | p-value |
|---|---|---|---|---|
| Intercept | 0.3 | [0.09, 0.51] | 0.11 | 0.006 |
| **Group (reference=Baseline)** | | | | |
| Copilot | -0.2 | [-0.65, 0.26] | 0.23 | 0.397 |
| Gemini | -0.3 | [-0.74, 0.14] | 0.22 | 0.186 |
| PI | -0.02 | [-0.46, 0.42] | 0.22 | 0.913 |
| ChatGPT | -0.13 | [-0.5, 0.24] | 0.19 | 0.487 |
| **AI Usage Label (reference=Cold)** | | | | |
| Hot | -0.47 | [-0.81, -0.13] | 0.17 | 0.007 |
| AI Usage (Hot):Copilot | 0.6 | [-0.04, 1.24] | 0.33 | 0.064 |
| AI Usage (Hot):Gemini | 0.77 | [0.12, 1.43] | 0.33 | 0.021 |
| AI Usage (Hot):PI | 0.38 | [-0.26, 1.02] | 0.33 | 0.247 |
| AI Usage (Hot):ChatGPT | 0.1 | [-0.63, 0.84] | 0.37 | 0.78 |

Table 136: Linear Mixed Effect Model with 5 groups for Dependence on AI (Withdrawal) and AI Usage Label

| Predictors | Coef | CI | Std. Err. | p-value |
|---|---|---|---|---|
| Intercept | 0.24 | [0.08, 0.41] | 0.08 | 0.003 |
| **Group (reference=Baseline)** | | | | |
| Copilot | -0.14 | [-0.5, 0.21] | 0.18 | 0.427 |
| Gemini | -0.24 | [-0.58, 0.1] | 0.17 | 0.162 |
| PI | -0.06 | [-0.4, 0.28] | 0.17 | 0.724 |
| ChatGPT | -0.13 | [-0.42, 0.15] | 0.15 | 0.364 |
| **AI Usage Label (reference=Cold)** | | | | |
| Hot | -0.2 | [-0.46, 0.06] | 0.13 | 0.137 |
| AI Usage (Hot):Copilot | 0.18 | [-0.32, 0.67] | 0.25 | 0.483 |
| AI Usage (Hot):Gemini | 0.3 | [-0.21, 0.81] | 0.26 | 0.247 |
| AI Usage (Hot):PI | 0.11 | [-0.39, 0.61] | 0.25 | 0.669 |
| AI Usage (Hot):ChatGPT | -0.11 | [-0.68, 0.46] | 0.29 | 0.7 |

Table 137: Linear Mixed Effect Model with 5 groups for Dependence on AI (Loss of Control) and AI Usage Label

| Predictors | Coef | CI | Std. Err. | p-value |
|---|---|---|---|---|
| Intercept | -0.01 | [-0.24, 0.21] | 0.11 | 0.913 |
| **Group (reference=Baseline)** | | | | |
| Copilot | -0.22 | [-0.7, 0.27] | 0.25 | 0.377 |
| Gemini | -0.22 | [-0.68, 0.25] | 0.24 | 0.363 |
| PI | -0.11 | [-0.58, 0.35] | 0.24 | 0.64 |
| ChatGPT | 0.77 | [0.38, 1.16] | 0.2 | 0.0 |
| **AI Usage Label (reference=Cold)** | | | | |
| Hot | 0.08 | [-0.28, 0.44] | 0.18 | 0.659 |
| AI Usage (Hot):Copilot | 0.17 | [-0.51, 0.84] | 0.34 | 0.625 |
| AI Usage (Hot):Gemini | 0.12 | [-0.58, 0.81] | 0.35 | 0.739 |
| AI Usage (Hot):PI | 0.49 | [-0.19, 1.17] | 0.35 | 0.159 |
| AI Usage (Hot):ChatGPT | -0.66 | [-1.43, 0.12] | 0.4 | 0.096 |

Table 138: Linear Mixed Effect Model with 5 groups for Attitude towards AI and AI Usage Label

| Predictors | Coef | CI | Std. Err. | p-value |
|---|---|---|---|---|
| Intercept | -0.06 | [-0.2, 0.07] | 0.07 | 0.353 |
| **Group (reference=Baseline)** | | | | |
| Copilot | -0.19 | [-0.48, 0.1] | 0.15 | 0.191 |
| Gemini | -0.02 | [-0.3, 0.26] | 0.14 | 0.9 |
| PI | -0.04 | [-0.32, 0.24] | 0.14 | 0.789 |
| ChatGPT | 0.53 | [0.3, 0.76] | 0.12 | 0.0 |
| **AI Usage Label (reference=Cold)** | | | | |
| Hot | 0.03 | [-0.18, 0.25] | 0.11 | 0.756 |
| AI Usage (Hot):Copilot | 0.3 | [-0.1, 0.7] | 0.21 | 0.146 |
| AI Usage (Hot):Gemini | 0.08 | [-0.33, 0.49] | 0.21 | 0.704 |
| AI Usage (Hot):PI | 0.22 | [-0.19, 0.62] | 0.21 | 0.292 |
| AI Usage (Hot):ChatGPT | -0.57 | [-1.03, -0.11] | 0.24 | 0.016 |

Table 139: Linear Mixed Effect Model with 5 groups for Attitude towards AI (Positive) and AI Usage Label

| Predictors | Coef | CI | Std. Err. | p-value |
|---|---|---|---|---|
| Intercept | 0.05 | [-0.11, 0.21] | 0.08 | 0.54 |
| **Group (reference=Baseline)** | | | | |
| Copilot | -0.03 | [-0.38, 0.33] | 0.18 | 0.886 |
| Gemini | -0.2 | [-0.54, 0.14] | 0.17 | 0.251 |
| PI | -0.07 | [-0.41, 0.27] | 0.17 | 0.671 |
| ChatGPT | 0.24 | [-0.04, 0.52] | 0.14 | 0.095 |
| **AI Usage Label (reference=Cold)** | | | | |
| Hot | 0.05 | [-0.21, 0.31] | 0.13 | 0.724 |
| AI Usage (Hot):Copilot | -0.13 | [-0.62, 0.36] | 0.25 | 0.604 |
| AI Usage (Hot):Gemini | 0.04 | [-0.47, 0.54] | 0.26 | 0.882 |
| AI Usage (Hot):PI | 0.27 | [-0.22, 0.77] | 0.25 | 0.283 |
| AI Usage (Hot):ChatGPT | -0.09 | [-0.65, 0.47] | 0.29 | 0.757 |

Table 140: Linear Mixed Effect Model with 5 groups for Attitude towards AI (Negative) and AI Usage Label

| Predictors | Coef | CI | Std. Err. | p-value |
|---|---|---|---|---|
| Intercept | 0.97 | [-0.77, 2.71] | 0.89 | 0.273 |
| **Group (reference=Baseline)** | | | | |
| Copilot | -1.17 | [-4.94, 2.6] | 1.92 | 0.542 |
| Gemini | -0.06 | [-3.7, 3.57] | 1.85 | 0.973 |
| PI | 1.48 | [-2.15, 5.11] | 1.85 | 0.424 |
| ChatGPT | 2.36 | [-0.68, 5.4] | 1.55 | 0.128 |
| **AI Usage Label (reference=Cold)** | | | | |
| Hot | -0.41 | [-3.22, 2.4] | 1.43 | 0.776 |
| AI Usage (Hot):Copilot | 4.76 | [-0.5, 10.02] | 2.68 | 0.076 |
| AI Usage (Hot):Gemini | 2.4 | [-3.01, 7.81] | 2.76 | 0.385 |
| AI Usage (Hot):PI | -1.23 | [-6.54, 4.09] | 2.71 | 0.65 |
| AI Usage (Hot):ChatGPT | 2.47 | [-3.57, 8.52] | 3.08 | 0.422 |

Table 141: Linear Mixed Effect Model with 5 groups for Interpersonal Orientation and AI Usage Label

| Predictors | Coef | CI | Std. Err. | p-value |
|---|---|---|---|---|
| Intercept | 0.49 | [-0.32, 1.29] | 0.41 | 0.236 |
| **Group (reference=Baseline)** | | | | |
| Copilot | 0.51 | [-1.23, 2.26] | 0.89 | 0.564 |
| Gemini | 0.42 | [-1.26, 2.1] | 0.86 | 0.622 |
| PI | -0.03 | [-1.71, 1.65] | 0.86 | 0.97 |
| ChatGPT | 1.24 | [-0.17, 2.64] | 0.72 | 0.085 |
| **AI Usage Label (reference=Cold)** | | | | |
| Hot | -0.96 | [-2.26, 0.33] | 0.66 | 0.146 |
| AI Usage (Hot):Copilot | -0.57 | [-3.01, 1.86] | 1.24 | 0.644 |
| AI Usage (Hot):Gemini | 0.76 | [-1.75, 3.26] | 1.28 | 0.554 |
| AI Usage (Hot):PI | 0.24 | [-2.22, 2.7] | 1.25 | 0.85 |
| AI Usage (Hot):ChatGPT | -0.56 | [-3.35, 2.24] | 1.43 | 0.696 |

Table 142: Linear Mixed Effect Model with 5 groups for Motivation for using AI (Escape) and AI Usage Label

| Predictors | Coef | CI | Std. Err. | p-value |
|---|---|---|---|---|
| Intercept | 0.59 | [-0.12, 1.3] | 0.36 | 0.101 |
| **Group (reference=Baseline)** | | | | |
| Copilot | 0.21 | [-1.33, 1.74] | 0.79 | 0.794 |
| Gemini | 0.31 | [-1.17, 1.8] | 0.76 | 0.678 |
| PI | 0.31 | [-1.17, 1.8] | 0.76 | 0.678 |
| ChatGPT | 1.74 | [0.5, 2.98] | 0.63 | 0.006 |
| **AI Usage Label (reference=Cold)** | | | | |
| Hot | 0.06 | [-1.09, 1.2] | 0.59 | 0.922 |
| AI Usage (Hot):Copilot | -0.78 | [-2.93, 1.37] | 1.1 | 0.476 |
| AI Usage (Hot):Gemini | 1.43 | [-0.78, 3.64] | 1.13 | 0.203 |
| AI Usage (Hot):PI | -0.24 | [-2.41, 1.93] | 1.11 | 0.829 |
| AI Usage (Hot):ChatGPT | -1.39 | [-3.86, 1.08] | 1.26 | 0.269 |

Table 143: Linear Mixed Effect Model with 5 groups for Motivation for using AI (Social) and AI Usage Label

| Predictors | Coef | CI | Std. Err. | p-value |
|---|---|---|---|---|
| Intercept | 0.59 | [0.02, 1.17] | 0.29 | 0.042 |
| **Group (reference=Baseline)** | | | | |
| Copilot | 1.31 | [0.06, 2.55] | 0.63 | 0.039 |
| Gemini | 0.13 | [-1.06, 1.33] | 0.61 | 0.828 |
| PI | -1.14 | [-2.34, 0.06] | 0.61 | 0.062 |
| ChatGPT | 2.24 | [1.24, 3.24] | 0.51 | 0.0 |
| **AI Usage Label (reference=Cold)** | | | | |
| Hot | -0.86 | [-1.78, 0.07] | 0.47 | 0.07 |
| AI Usage (Hot):Copilot | -1.04 | [-2.78, 0.69] | 0.88 | 0.237 |
| AI Usage (Hot):Gemini | 0.33 | [-1.45, 2.11] | 0.91 | 0.718 |
| AI Usage (Hot):PI | 1.95 | [0.2, 3.7] | 0.89 | 0.029 |
| AI Usage (Hot):ChatGPT | -0.78 | [-2.77, 1.21] | 1.01 | 0.443 |

Table 144: Linear Mixed Effect Model with 5 groups for Motivation for using AI (Instrumental) and AI Usage Label

| Predictors | Coef | CI | Std. Err. | p-value |
|---|---|---|---|---|
| Intercept | 0.38 | [-0.33, 1.08] | 0.36 | 0.293 |
| **Group (reference=Baseline)** | | | | |
| Copilot | 0.42 | [-1.11, 1.95] | 0.78 | 0.589 |
| Gemini | 0.35 | [-1.12, 1.82] | 0.75 | 0.642 |
| PI | -0.56 | [-2.03, 0.91] | 0.75 | 0.456 |
| ChatGPT | 2.34 | [1.11, 3.58] | 0.63 | 0.0 |
| **AI Usage Label (reference=Cold)** | | | | |
| Hot | -0.47 | [-1.6, 0.67] | 0.58 | 0.423 |
| AI Usage (Hot):Copilot | 0.97 | [-1.16, 3.11] | 1.09 | 0.371 |
| AI Usage (Hot):Gemini | 0.54 | [-1.65, 2.73] | 1.12 | 0.631 |
| AI Usage (Hot):PI | 1.01 | [-1.14, 3.17] | 1.1 | 0.358 |
| AI Usage (Hot):ChatGPT | -1.86 | [-4.31, 0.59] | 1.25 | 0.137 |

Table 145: Linear Mixed Effect Model with 5 groups for Motivation for using AI (Entertainment) and AI Usage Label

| Predictors | Coef | CI | Std. Err. | p-value |
|---|---|---|---|---|
| Intercept | 0.05 | [-0.34, 0.45] | 0.2 | 0.788 |
| **Group (reference=Baseline)** | | | | |
| Copilot | 0.55 | [-0.31, 1.4] | 0.44 | 0.21 |
| Gemini | 0.86 | [0.03, 1.68] | 0.42 | 0.041 |
| PI | -0.05 | [-0.88, 0.77] | 0.42 | 0.897 |
| ChatGPT | 1.67 | [0.98, 2.36] | 0.35 | 0.0 |
| **AI Usage Label (reference=Cold)** | | | | |
| Hot | 0.38 | [-0.25, 1.02] | 0.32 | 0.24 |
| AI Usage (Hot):Copilot | -0.9 | [-2.09, 0.29] | 0.61 | 0.137 |
| AI Usage (Hot):Gemini | -0.39 | [-1.61, 0.83] | 0.62 | 0.532 |
| AI Usage (Hot):PI | 0.44 | [-0.76, 1.64] | 0.61 | 0.476 |
| AI Usage (Hot):ChatGPT | -1.7 | [-3.07, -0.34] | 0.7 | 0.015 |

Table 146: Linear Mixed Effect Model with 5 groups for Attachment towards AI and AI Usage Label

| Predictors | Coef | CI | Std. Err. | p-value |
|---|---|---|---|---|
| Intercept | 0.38 | [0.01, 0.75] | 0.19 | 0.043 |
| **Group (reference=Baseline)** | | | | |
| Copilot | 0.42 | [-0.37, 1.22] | 0.41 | 0.299 |
| Gemini | 0.35 | [-0.42, 1.12] | 0.39 | 0.372 |
| PI | -0.47 | [-1.24, 0.3] | 0.39 | 0.23 |
| ChatGPT | 0.51 | [-0.13, 1.15] | 0.33 | 0.119 |
| **AI Usage Label (reference=Cold)** | | | | |
| Hot | -0.03 | [-0.62, 0.56] | 0.3 | 0.919 |
| AI Usage (Hot):Copilot | -1.0 | [-2.11, 0.11] | 0.57 | 0.077 |
| AI Usage (Hot):Gemini | 0.2 | [-0.94, 1.34] | 0.58 | 0.727 |
| AI Usage (Hot):PI | 0.76 | [-0.36, 1.88] | 0.57 | 0.185 |
| AI Usage (Hot):ChatGPT | -0.86 | [-2.13, 0.42] | 0.65 | 0.187 |

Table 147: Linear Mixed Effect Model with 5 groups for Recommendation to use AI and AI Usage Label

| Predictors | Coef | CI | Std. Err. | p-value |
|---|---|---|---|---|
| Intercept | 0.16 | [-0.16, 0.49] | 0.17 | 0.327 |
| **Group (reference=Baseline)** | | | | |
| Copilot | 0.54 | [-0.16, 1.24] | 0.36 | 0.133 |
| Gemini | 0.47 | [-0.2, 1.15] | 0.35 | 0.17 |
| PI | -0.16 | [-0.84, 0.51] | 0.35 | 0.639 |
| ChatGPT | 0.5 | [-0.06, 1.07] | 0.29 | 0.081 |
| **AI Usage Label (reference=Cold)** | | | | |
| Hot | 0.01 | [-0.51, 0.54] | 0.27 | 0.965 |
| AI Usage (Hot):Copilot | -0.48 | [-1.46, 0.5] | 0.5 | 0.336 |
| AI Usage (Hot):Gemini | 0.15 | [-0.86, 1.16] | 0.51 | 0.768 |
| AI Usage (Hot):PI | 0.81 | [-0.18, 1.8] | 0.51 | 0.11 |
| AI Usage (Hot):ChatGPT | -0.68 | [-1.8, 0.45] | 0.57 | 0.237 |

Table 148: Linear Mixed Effect Model with 5 groups for Satisfaction with AI and AI Usage Label

| Predictors | Coef | CI | Std. Err. | p-value |
|---|---|---|---|---|
| Intercept | 0.16 | [-0.16, 0.48] | 0.16 | 0.318 |
| **Group (reference=Baseline)** | | | | |
| Copilot | 0.64 | [-0.05, 1.33] | 0.35 | 0.07 |
| Gemini | 0.29 | [-0.37, 0.96] | 0.34 | 0.389 |
| PI | -0.07 | [-0.74, 0.59] | 0.34 | 0.834 |
| ChatGPT | 0.39 | [-0.16, 0.95] | 0.28 | 0.166 |
| **AI Usage Label (reference=Cold)** | | | | |
| Hot | 0.1 | [-0.42, 0.61] | 0.26 | 0.707 |
| AI Usage (Hot):Copilot | -0.59 | [-1.55, 0.37] | 0.49 | 0.229 |
| AI Usage (Hot):Gemini | 0.05 | [-0.94, 1.04] | 0.51 | 0.926 |
| AI Usage (Hot):PI | 0.36 | [-0.62, 1.33] | 0.5 | 0.474 |
| AI Usage (Hot):ChatGPT | -0.85 | [-1.96, 0.25] | 0.56 | 0.13 |

Table 149: Linear Mixed Effect Model with 5 groups for AI Helpfulness and AI Usage Label

| Predictors | Coef | CI | Std. Err. | p-value |
|---|---|---|---|---|
| Intercept | 0.14 | [-0.26, 0.53] | 0.2 | 0.499 |
| **Group (reference=Baseline)** | | | | |
| Copilot | 0.36 | [-0.48, 1.21] | 0.43 | 0.4 |
| Gemini | 0.14 | [-0.68, 0.96] | 0.42 | 0.742 |
| PI | 0.41 | [-0.41, 1.23] | 0.42 | 0.326 |
| ChatGPT | 0.92 | [0.24, 1.61] | 0.35 | 0.008 |
| **AI Usage Label (reference=Cold)** | | | | |
| Hot | -0.09 | [-0.72, 0.54] | 0.32 | 0.777 |
| AI Usage (Hot):Copilot | -0.56 | [-1.75, 0.62] | 0.6 | 0.353 |
| AI Usage (Hot):Gemini | -0.28 | [-1.5, 0.94] | 0.62 | 0.651 |
| AI Usage (Hot):PI | -0.09 | [-1.29, 1.11] | 0.61 | 0.883 |
| AI Usage (Hot):ChatGPT | -1.16 | [-2.52, 0.2] | 0.69 | 0.094 |

Table 150: Linear Mixed Effect Model with 5 groups for Perceived Human-Like Behavior and AI Usage Label

| Predictors | Coef | CI | Std. Err. | p-value |
|---|---|---|---|---|
| Intercept | 0.1 | [-0.16, 0.35] | 0.13 | 0.455 |
| **Group (reference=Baseline)** | | | | |
| Copilot | 0.48 | [-0.08, 1.03] | 0.28 | 0.093 |
| Gemini | 0.11 | [-0.43, 0.64] | 0.27 | 0.697 |
| PI | 0.57 | [0.04, 1.11] | 0.27 | 0.037 |
| ChatGPT | 1.4 | [0.95, 1.84] | 0.23 | 0.0 |
| **AI Usage Label (reference=Cold)** | | | | |
| Hot | 0.1 | [-0.31, 0.52] | 0.21 | 0.626 |
| AI Usage (Hot):Copilot | 0.3 | [-0.47, 1.08] | 0.4 | 0.445 |
| AI Usage (Hot):Gemini | 0.63 | [-0.17, 1.43] | 0.41 | 0.122 |
| AI Usage (Hot):PI | -0.23 | [-1.01, 0.56] | 0.4 | 0.569 |
| AI Usage (Hot):ChatGPT | -1.07 | [-1.96, -0.18] | 0.46 | 0.019 |

Table 151: Linear Mixed Effect Model with 5 groups for Perceived AI empathy and AI Usage Label

## Usefulness of AI

Figure 29: Agreement rating (1=Strongly disagree; 5=Strongly agree) to usefulness of AI for eight scenarios across baseline and active usage groups. Bars represent average, and the error bars indicate 95% confidence intervals. Dotted line is drawn at 3=Neutral for ease of reading.

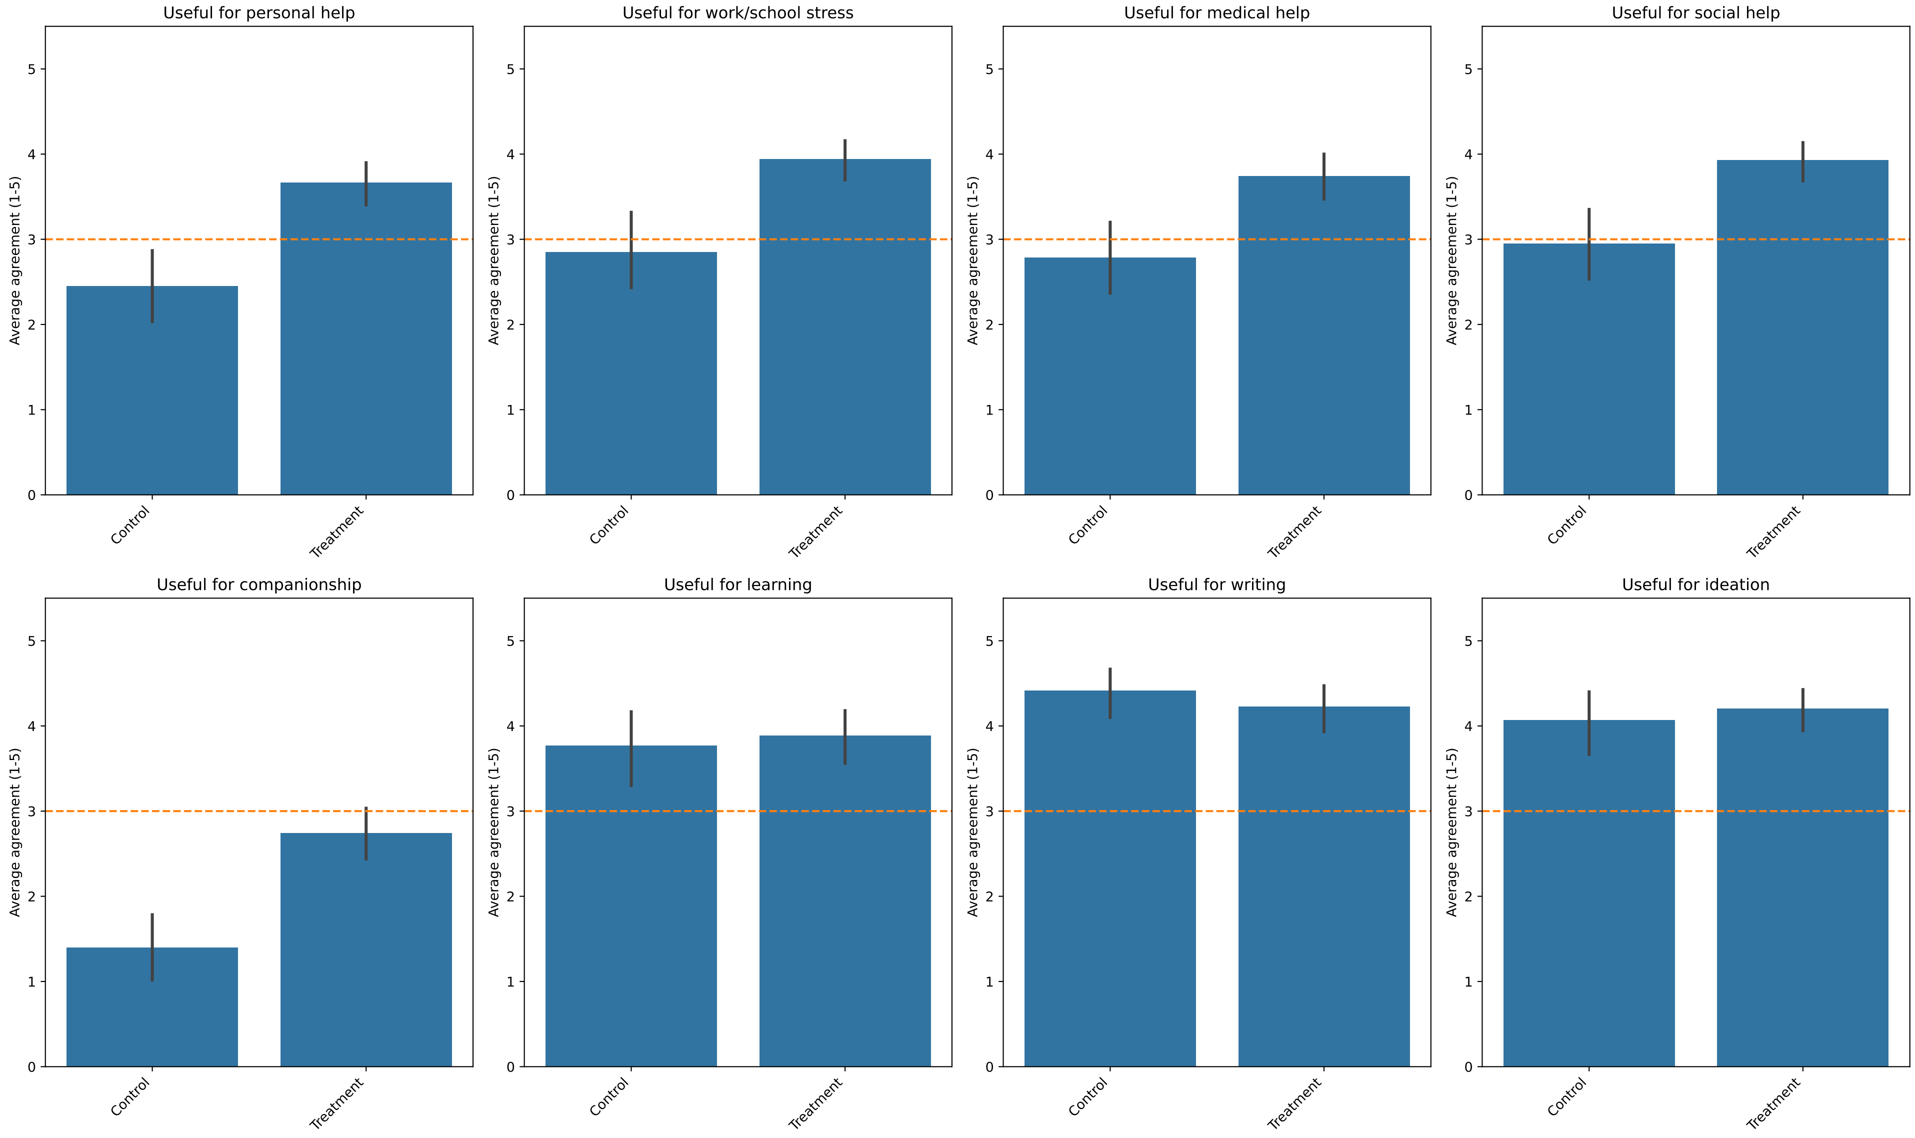

Figure 30: Agreement rating (1=Strongly disagree; 5=Strongly agree) to usefulness of AI for eight scenarios across Platform groups. Bars represent average, and the error bars indicate 95% confidence intervals. Dotted line is drawn at 3=Neutral for ease of reading.

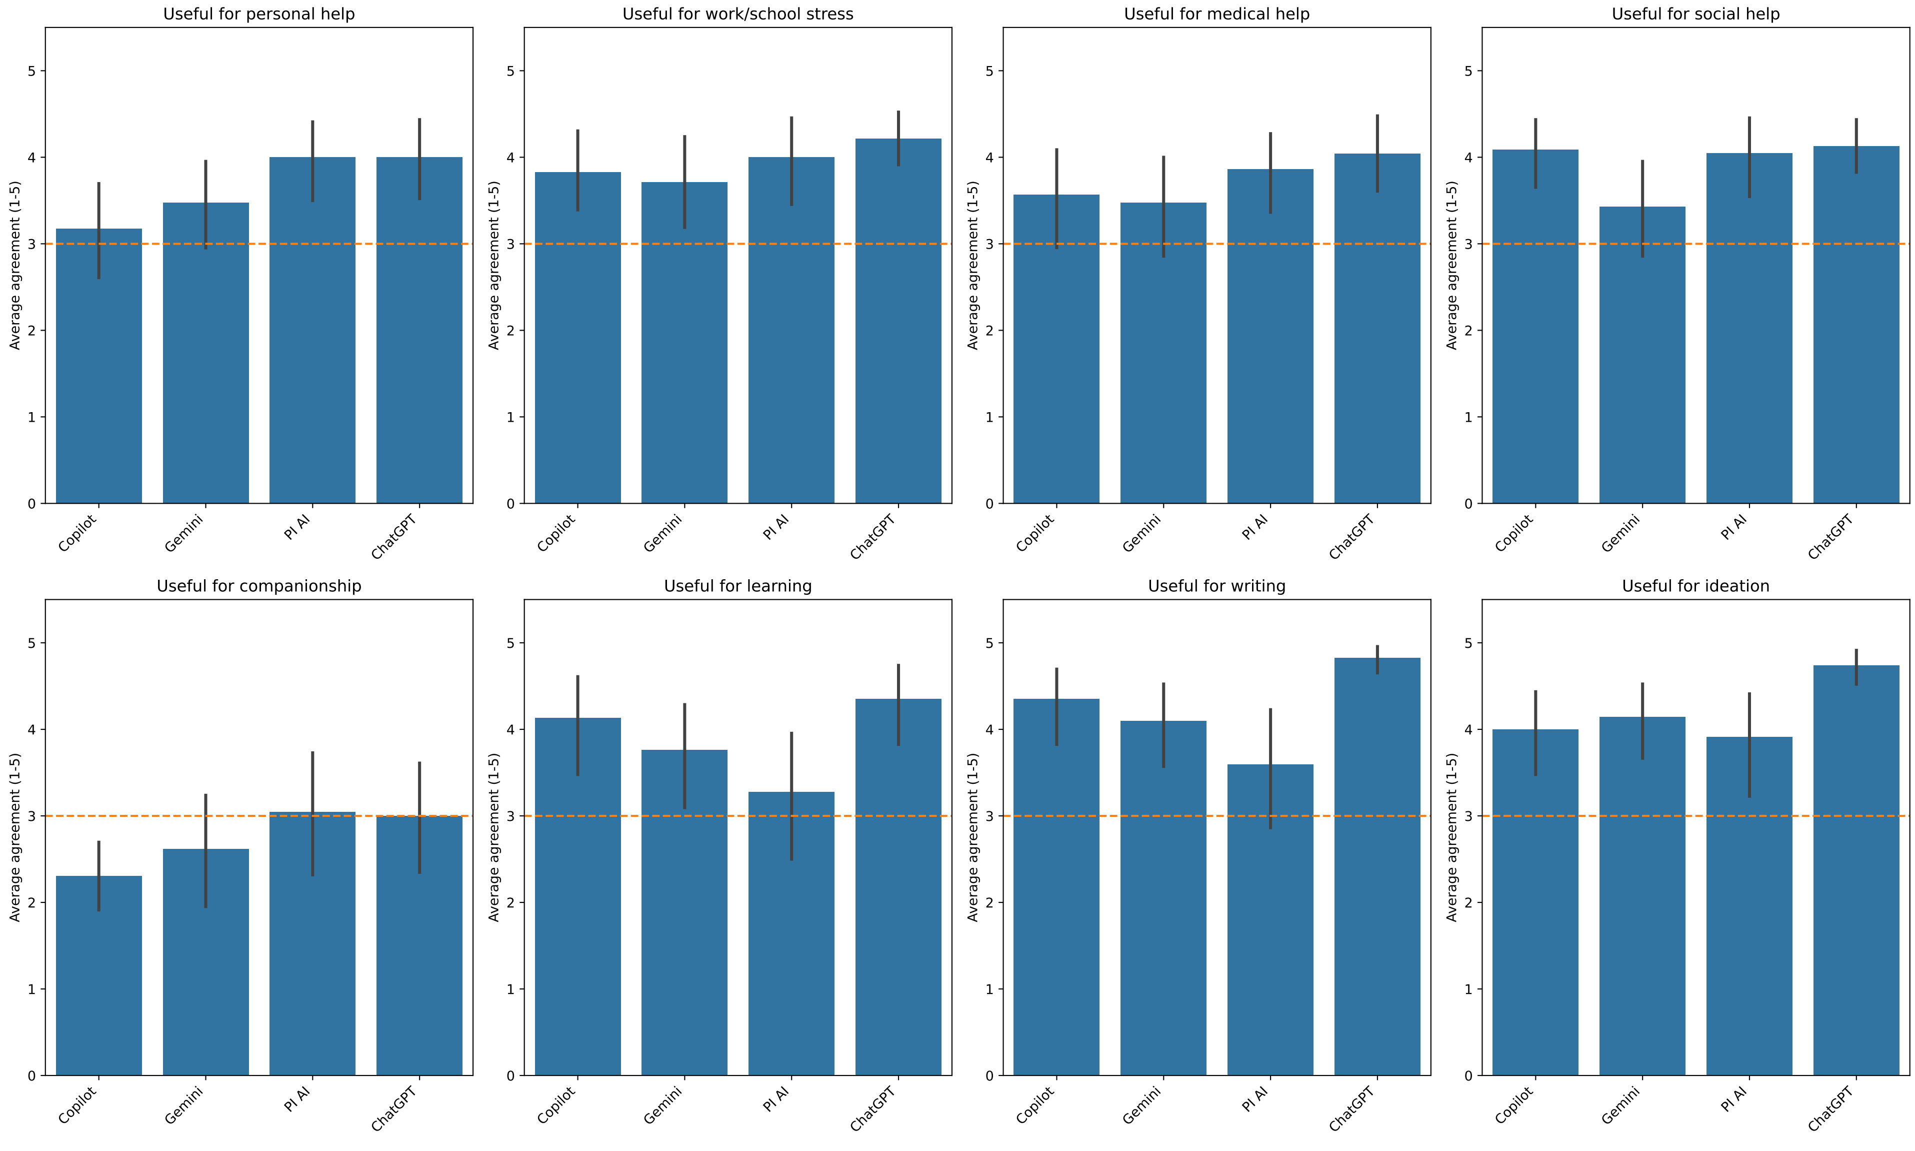

## Negative Consequences of Using AI

Figure 31: Agreement rating (1=Strongly disagree; 5=Strongly agree) to ten statements that potentially indicate negative consequences of using AI across baseline and active usage groups. Bars represent average, and the error bars indicate 95% confidence intervals. Dotted line is drawn at 3=Neutral for ease of reading.

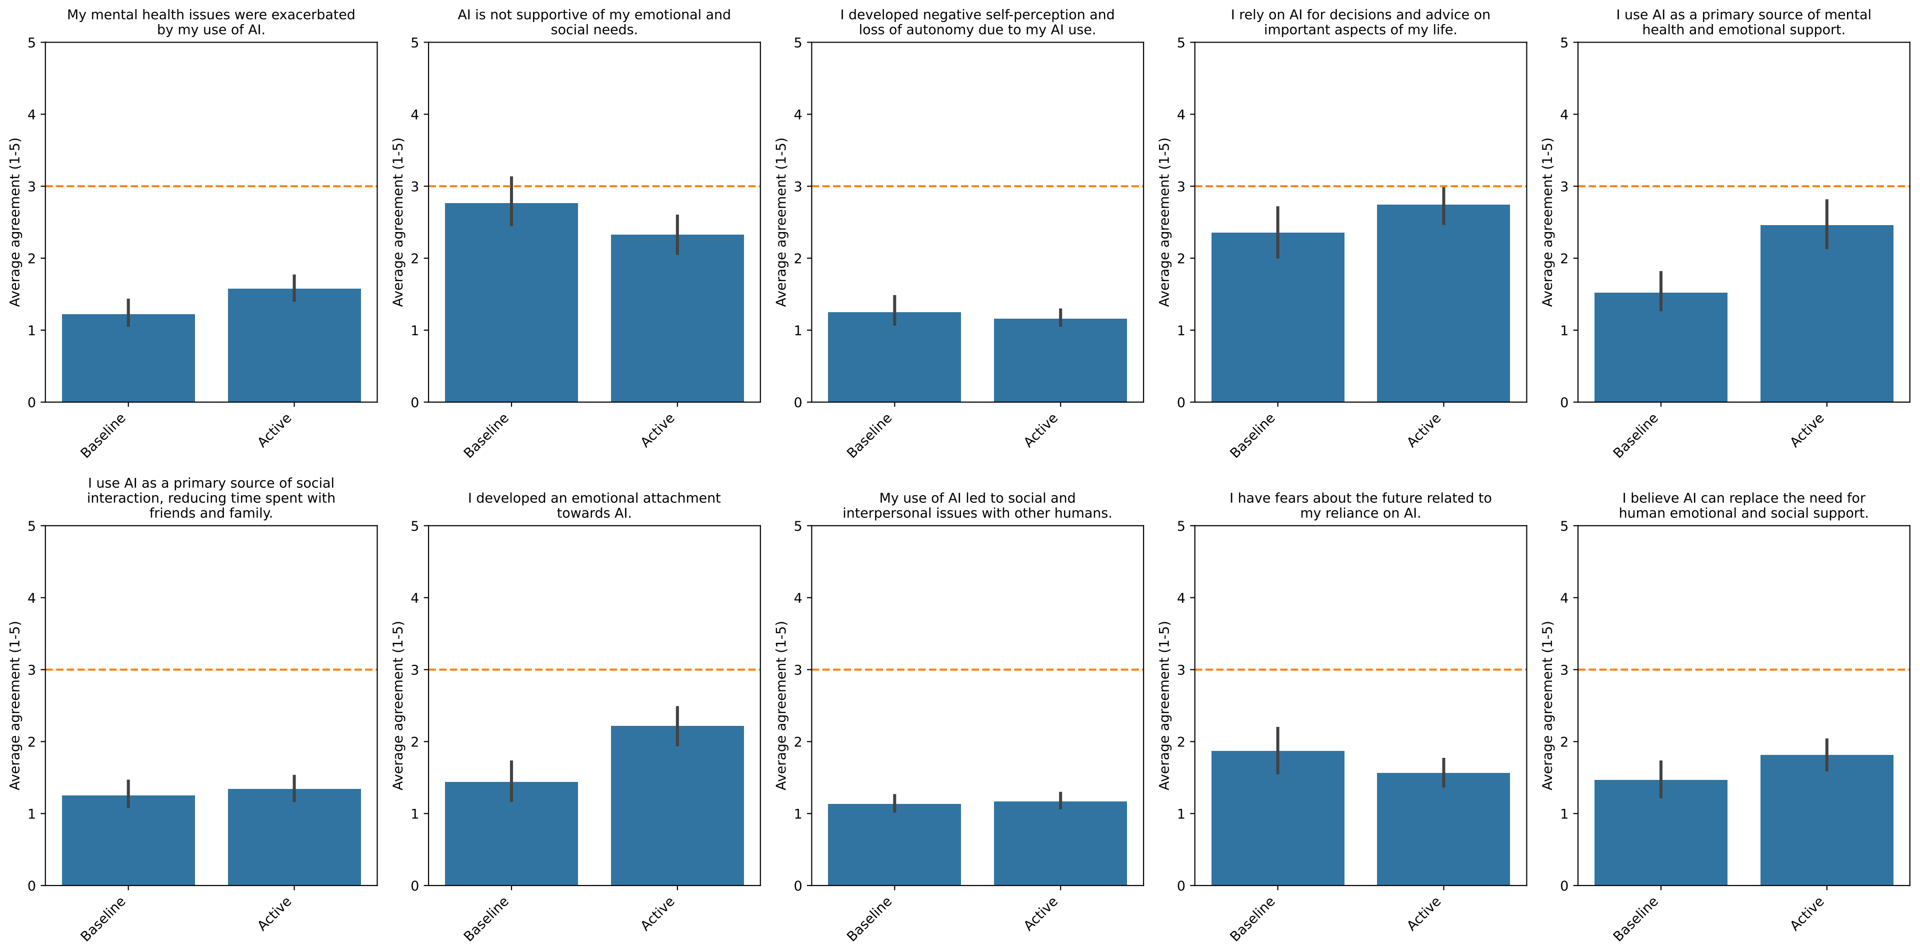

Figure 32: Agreement rating (1=Strongly disagree; 5=Strongly agree) to ten statements that potentially indicate negative consequences of using AI across Platform groups. Bars represent average, and the error bars indicate 95% confidence intervals. Dotted line is drawn at 3=Neutral for ease of reading.

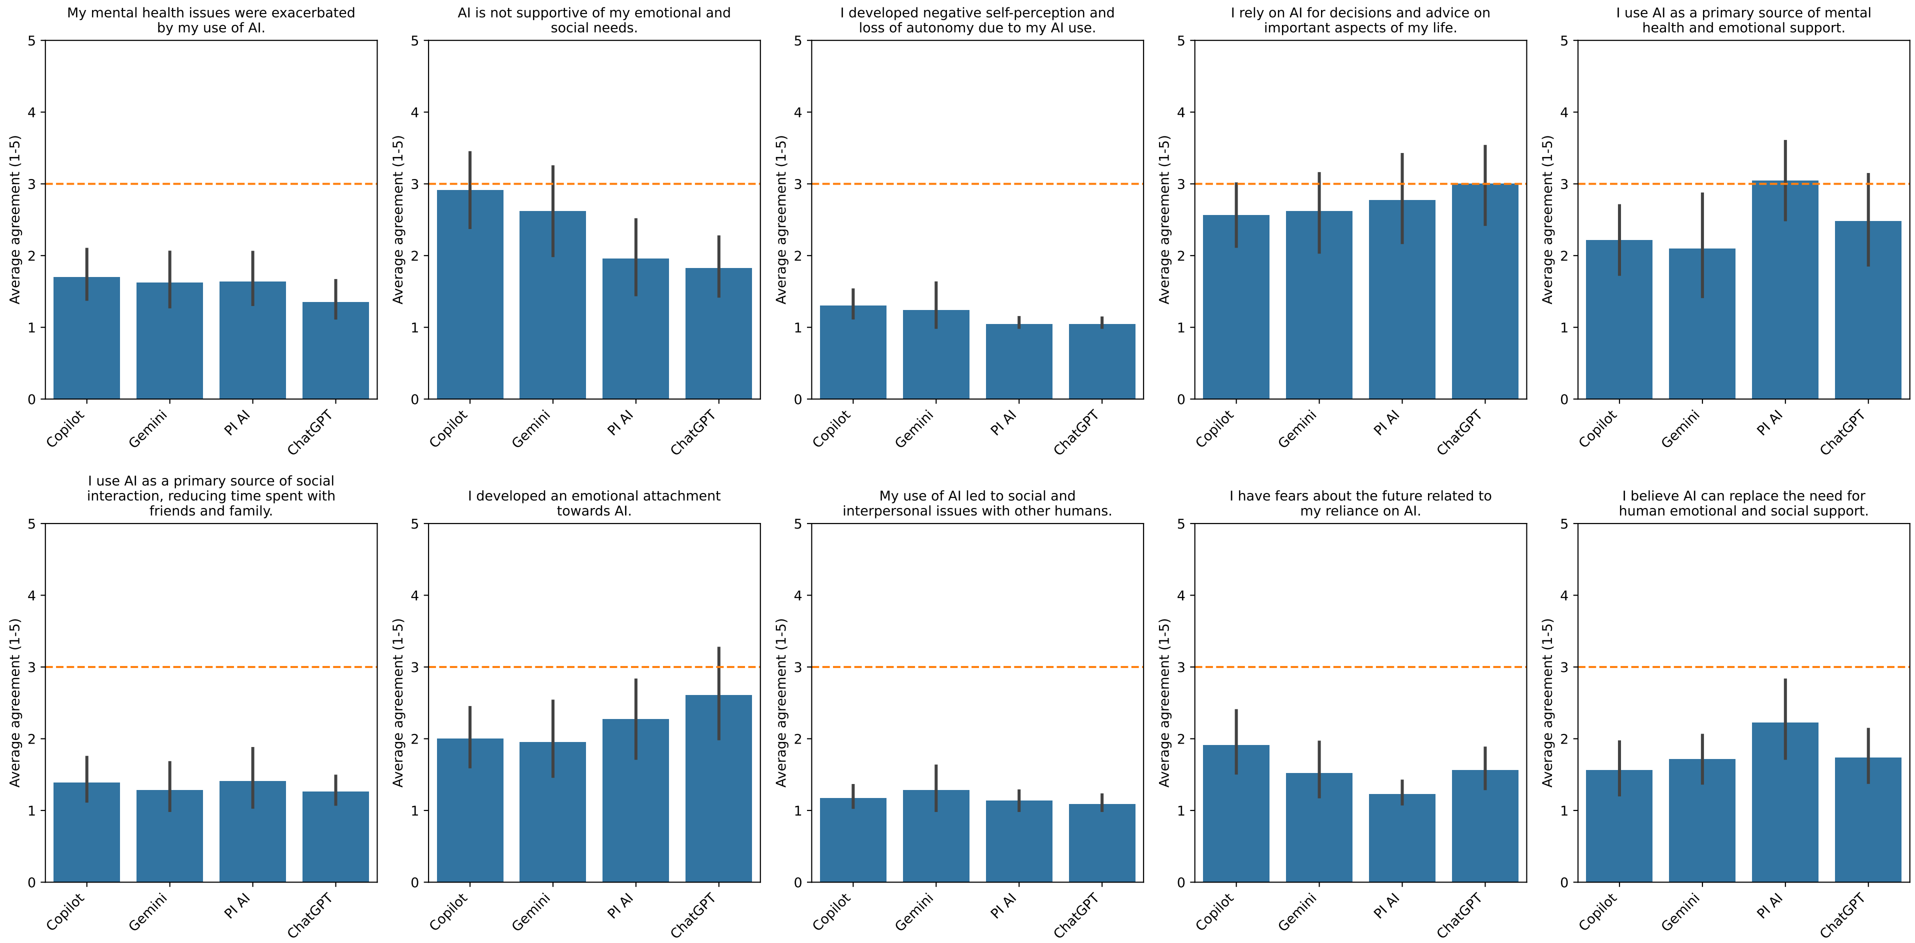

# Plan to Use or Avoid Using AI

Figure 33: Percentage of times participants indicated that they plan to use AI (blue) or avoid using AI (orange) for 13 usage scenarios across baseline and active usage groups.

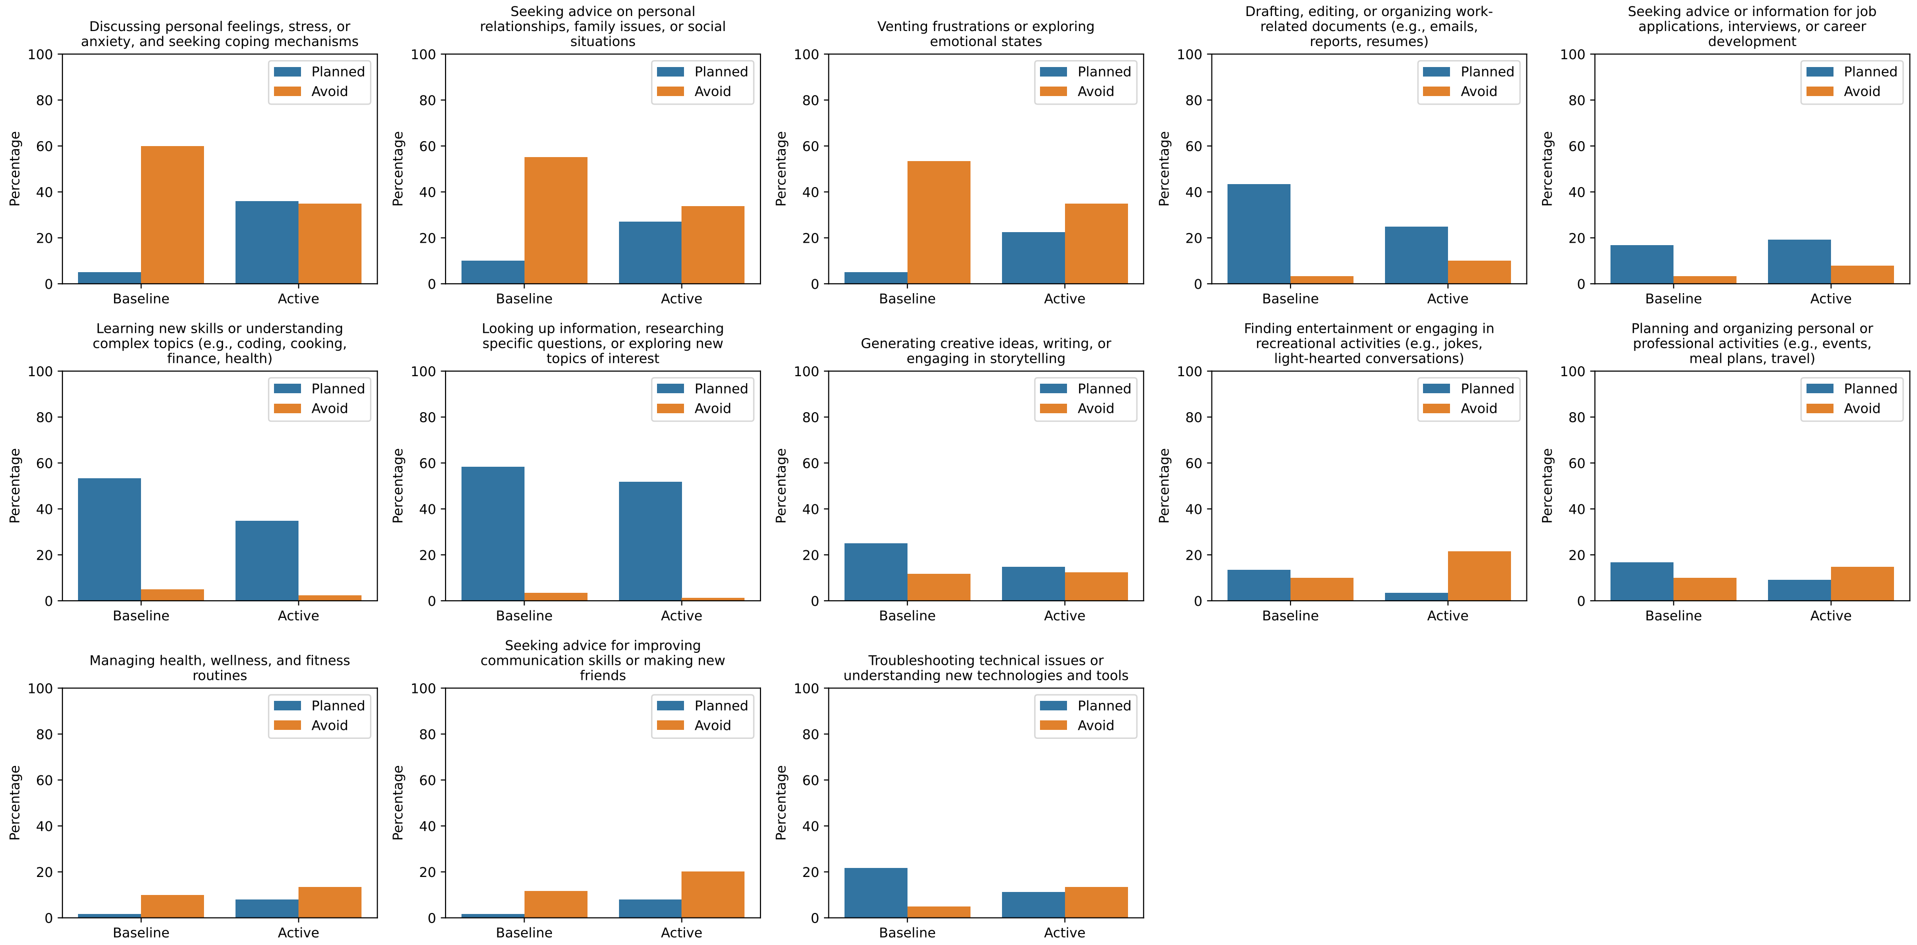

Figure 34: Percentage of times participants indicated that they plan to use AI (blue) or avoid using AI (orange) for 13 usage scenarios across Platform groups.

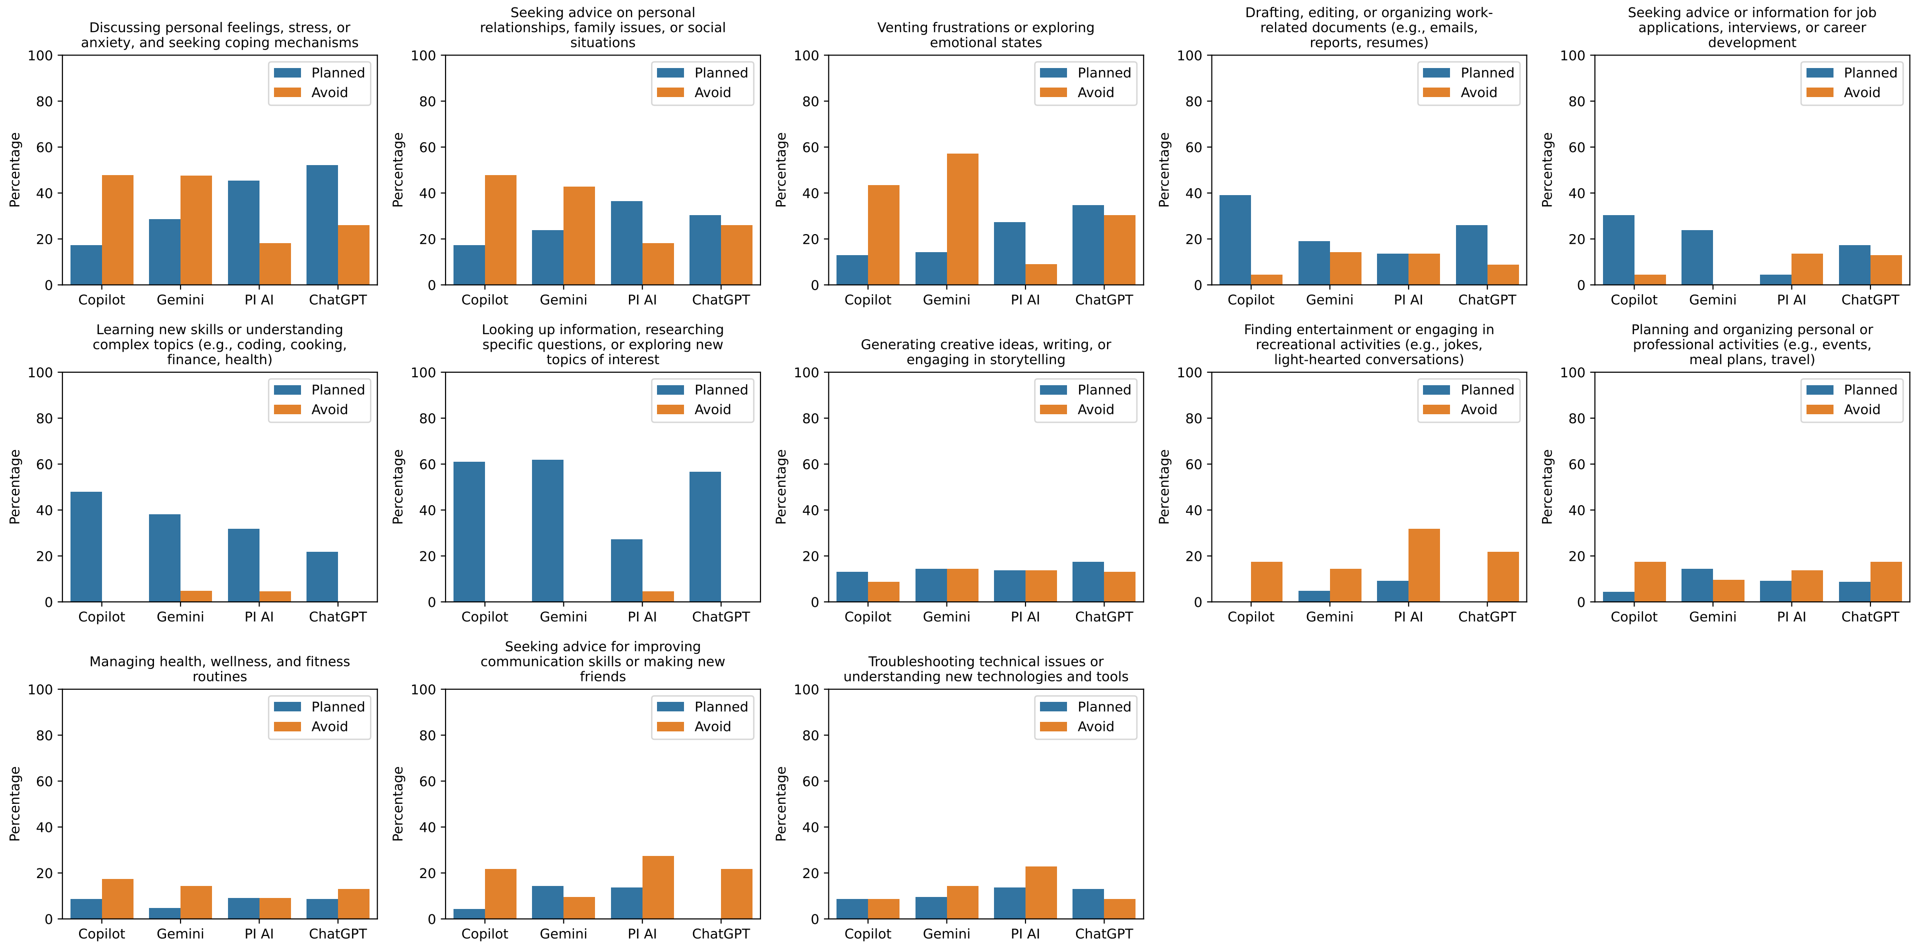

## What Designers Should Focus on for Reducing AI Dependence

Figure 35: Percentage of times participants indicated that they think designers should focus on (blue) or should not focus on (orange) 10 mitigation strategies for reducing AI dependence across baseline and active usage groups.

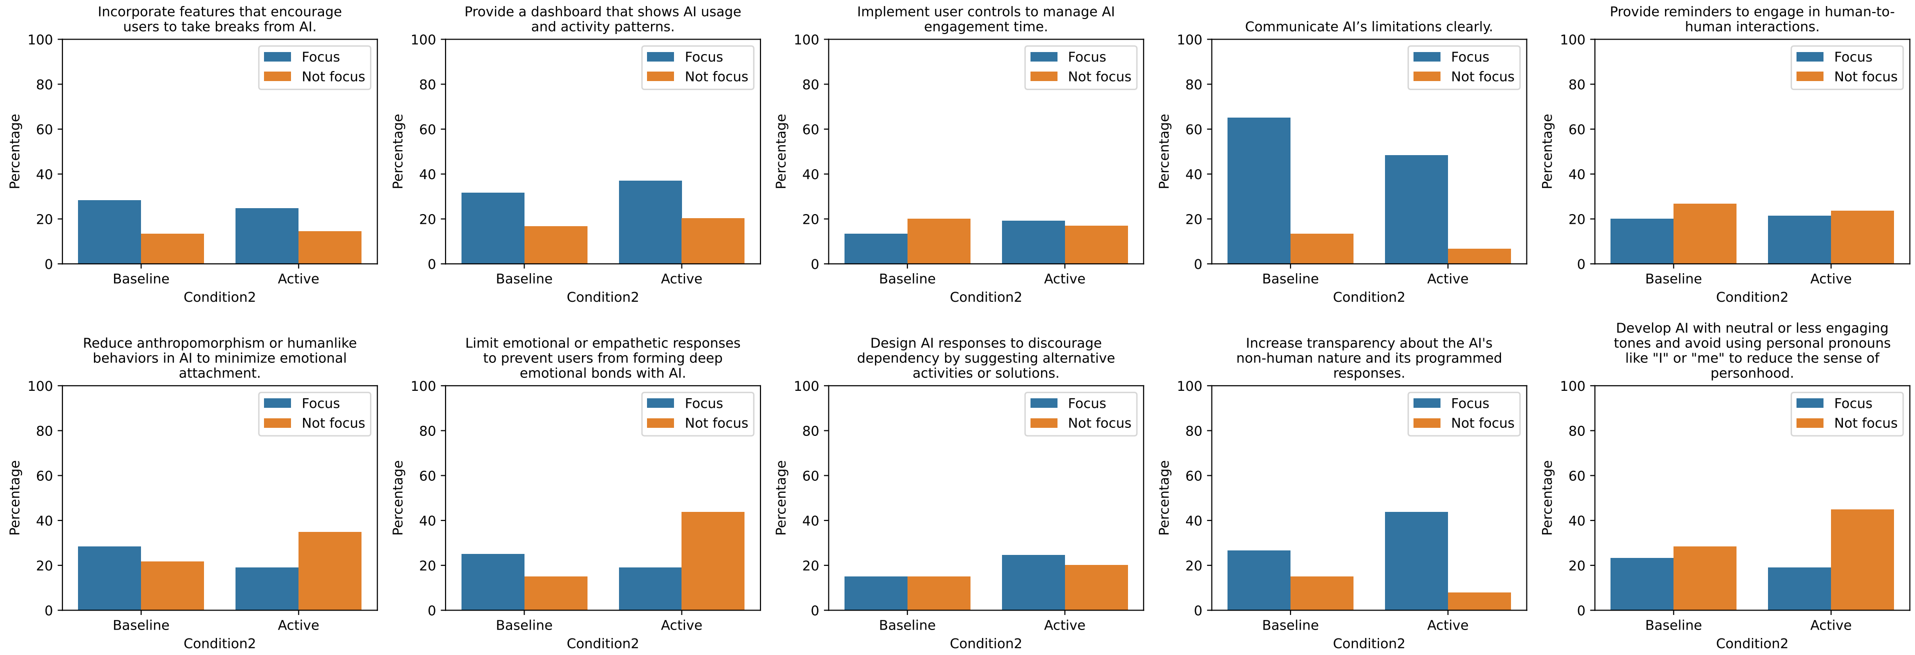

Figure 36: Percentage of times participants indicated that they think designers should focus on (blue) or should not focus on (orange) 10 mitigation strategies for reducing AI dependence across Platform groups.

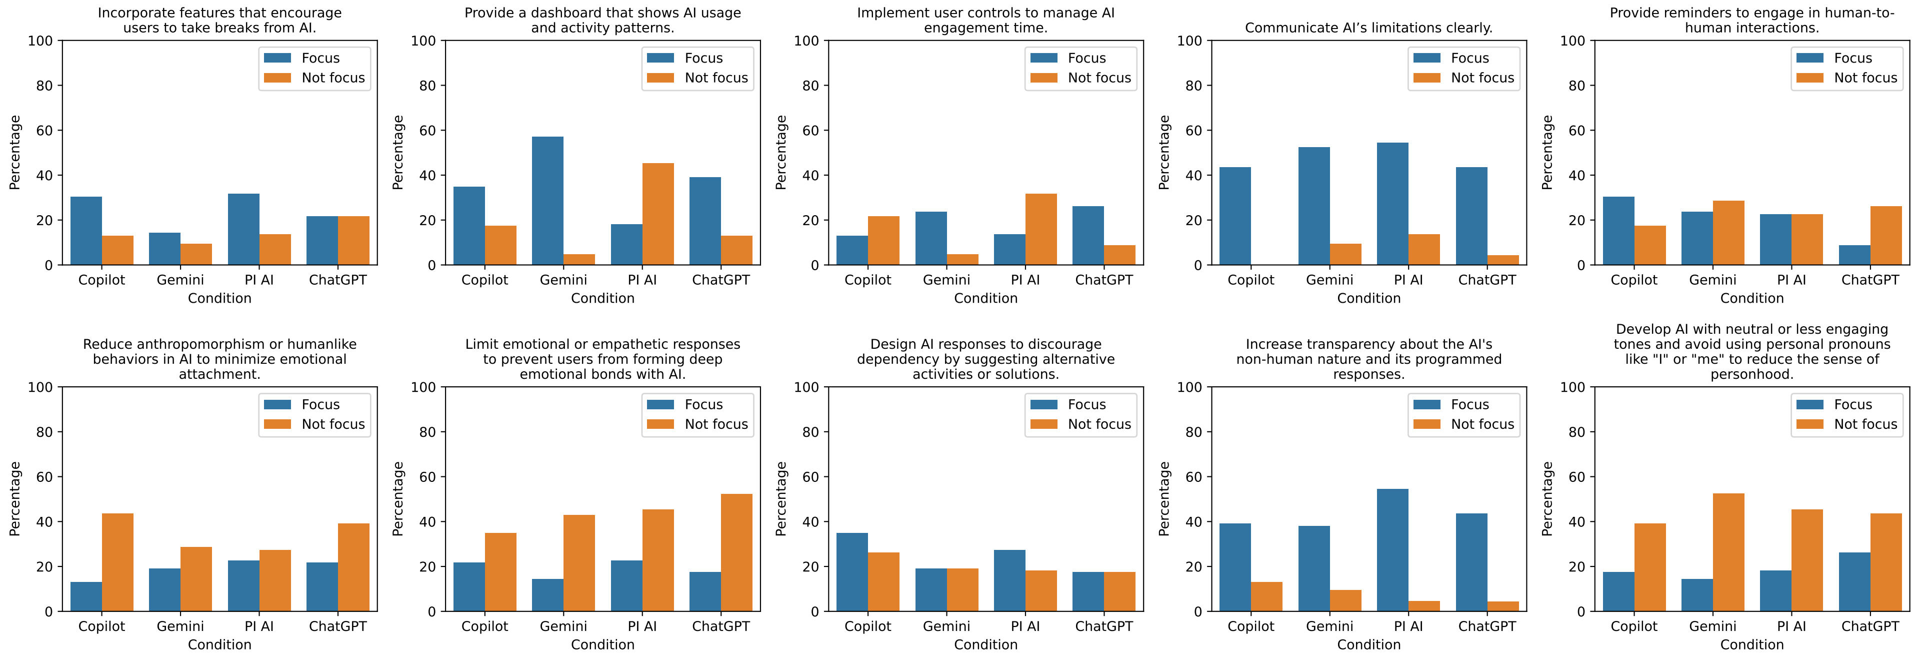

Supplement: Supplementary file 1 [file supplementary.pdf]
